# Supplementary material for: Orbital-free approximations to the kinetic-energy density in exchange-correlation MGGA functionals: tests on solids
Source: arXiv:1807.07302 ancillary file (2018-07-19)
Supplement: Supplementary file 1 [file Supplementary_Material.pdf]

# Supplementary material

## Orbital-free approximations to the kinetic-energy density in exchange-correlation MGGA functionals: tests on solids

Fabien Tran, Péter Kovács, Leila Kalantari, Georg K. H. Madsen, and Peter Blaha
*Institute of Materials Chemistry, Vienna University of Technology,*
*Getreidemarkt 9/165-TC, A-1060 Vienna, Austria*

TABLE S1. Equilibrium lattice constant $a_0$ (in Å) of 44 solids. The experimental values are from Refs. 1 and 2. All results were obtained non-self-consistently using PBE orbitals/density. The space group number is indicated in parenthesis.

| Solid | Expt. | MVS | MVS(GEA2L) | MVS(TW02L) | MVS(PC) | MVS(CR) | MVS(GEAloc) | MVS(PCopt) | MVS(CRopt) |
|---|---|---|---|---|---|---|---|---|---|
| C (227) | 3.553 | 3.544 | 3.572 | 3.574 | 3.579 | 3.571 | 3.577 | 3.550 | 3.576 |
| Si (227) | 5.412 | 5.396 | 5.406 | 5.409 | 5.408 | 5.406 | 5.412 | 5.389 | 5.428 |
| Ge (227) | 5.641 | 5.589 | 5.589 | 5.590 | 5.590 | 5.589 | 5.607 | 5.602 | 5.658 |
| Sn (227) | 6.477 | 6.468 | 6.448 | 6.448 | 6.449 | 6.448 | 6.486 | 6.486 | 6.550 |
| SiC (216) | 4.346 | 4.320 | 4.345 | 4.348 | 4.350 | 4.344 | 4.344 | 4.324 | 4.350 |
| BN (216) | 3.592 | 3.584 | 3.601 | 3.604 | 3.609 | 3.600 | 3.602 | 3.584 | 3.602 |
| BP (216) | 4.525 | 4.506 | 4.531 | 4.534 | 4.539 | 4.531 | 4.543 | 4.513 | 4.546 |
| AlN (216) | 4.368 | 4.336 | 4.339 | 4.344 | 4.344 | 4.339 | 4.335 | 4.322 | 4.348 |
| AlP (216) | 5.451 | 5.430 | 5.421 | 5.425 | 5.422 | 5.420 | 5.424 | 5.408 | 5.443 |
| AlAs (216) | 5.649 | 5.616 | 5.612 | 5.615 | 5.613 | 5.612 | 5.624 | 5.617 | 5.660 |
| GaN (216) | 4.509 | 4.437 | 4.466 | 4.468 | 4.470 | 4.465 | 4.475 | 4.458 | 4.499 |
| GaP (216) | 5.439 | 5.390 | 5.385 | 5.387 | 5.386 | 5.385 | 5.394 | 5.384 | 5.432 |
| GaAs (216) | 5.640 | 5.584 | 5.592 | 5.592 | 5.593 | 5.592 | 5.621 | 5.613 | 5.678 |
| InP (216) | 5.858 | 5.837 | 5.839 | 5.841 | 5.840 | 5.839 | 5.862 | 5.848 | 5.908 |
| InAs (216) | 6.047 | 6.034 | 6.041 | 6.041 | 6.042 | 6.041 | 6.088 | 6.081 | 6.157 |
| InSb (216) | 6.473 | 6.486 | 6.461 | 6.461 | 6.461 | 6.462 | 6.512 | 6.514 | 6.590 |
| LiH (225) | 3.979 | 4.000 | 3.955 | 3.972 | 3.973 | 3.952 | 3.966 | 3.939 | 3.961 |
| LiF (225) | 3.972 | 3.930 | 3.931 | 3.950 | 3.947 | 3.930 | 3.939 | 3.911 | 3.961 |
| LiCl (225) | 5.070 | 5.069 | 4.989 | 5.010 | 5.005 | 4.988 | 5.023 | 5.000 | 5.083 |
| NaF (225) | 4.582 | 4.576 | 4.537 | 4.564 | 4.537 | 4.537 | 4.553 | 4.535 | 4.658 |
| NaCl (225) | 5.569 | 5.584 | 5.477 | 5.512 | 5.477 | 5.477 | 5.512 | 5.497 | 5.665 |
| MgO (225) | 4.189 | 4.175 | 4.181 | 4.191 | 4.185 | 4.181 | 4.183 | 4.162 | 4.208 |
| Li (229) | 3.443 | 3.469 | 3.397 | 3.417 | 3.419 | 3.396 | 3.393 | 3.352 | 3.388 |
| Na (229) | 4.205 | 4.211 | 4.135 | 4.161 | 4.132 | 4.135 | 4.160 | 4.135 | 4.231 |
| Al (225) | 4.022 | 3.920 | 3.962 | 3.966 | 3.963 | 3.962 | 3.962 | 3.931 | 3.978 |
| K (229) | 5.246 | 5.395 | 5.238 | 5.280 | 5.232 | 5.237 | 5.276 | 5.244 | 5.383 |
| Ca (225) | 5.559 | 5.489 | 5.474 | 5.493 | 5.474 | 5.474 | 5.492 | 5.443 | 5.519 |
| Rb (229) | 5.629 | 5.766 | 5.637 | 5.681 | 5.635 | 5.637 | 5.690 | 5.656 | 5.782 |
| Sr (225) | 6.059 | 5.996 | 5.978 | 6.001 | 5.976 | 5.978 | 6.001 | 5.947 | 6.037 |
| Cs (229) | 6.043 | 6.361 | 6.217 | 6.272 | 6.214 | 6.217 | 6.286 | 6.219 | 6.342 |
| Ba (229) | 4.994 | 5.062 | 5.045 | 5.069 | 5.043 | 5.045 | 5.061 | 4.978 | 5.069 |
| V (229) | 3.023 | 2.952 | 2.967 | 2.970 | 2.967 | 2.967 | 2.979 | 2.964 | 2.992 |
| Ni (225) | 3.510 | 3.430 | 3.437 | 3.437 | 3.436 | 3.437 | 3.464 | 3.469 | 3.504 |
| Cu (225) | 3.599 | 3.525 | 3.517 | 3.517 | 3.518 | 3.517 | 3.546 | 3.556 | 3.587 |
| Nb (229) | 3.300 | 3.272 | 3.287 | 3.288 | 3.286 | 3.287 | 3.294 | 3.273 | 3.305 |
| Mo (229) | 3.142 | 3.124 | 3.137 | 3.138 | 3.137 | 3.137 | 3.146 | 3.132 | 3.157 |
| Rh (225) | 3.786 | 3.765 | 3.781 | 3.781 | 3.781 | 3.781 | 3.805 | 3.799 | 3.833 |
| Pd (225) | 3.876 | 3.866 | 3.872 | 3.871 | 3.872 | 3.872 | 3.910 | 3.914 | 3.961 |
| Ag (225) | 4.070 | 4.046 | 4.034 | 4.033 | 4.033 | 4.033 | 4.085 | 4.100 | 4.161 |
| Ta (229) | 3.298 | 3.279 | 3.285 | 3.284 | 3.284 | 3.285 | 3.312 | 3.315 | 3.340 |
| W (229) | 3.162 | 3.146 | 3.152 | 3.151 | 3.151 | 3.152 | 3.171 | 3.173 | 3.191 |
| Ir (225) | 3.831 | 3.820 | 3.825 | 3.823 | 3.825 | 3.825 | 3.854 | 3.864 | 3.881 |
| Pt (225) | 3.917 | 3.910 | 3.908 | 3.906 | 3.908 | 3.908 | 3.942 | 3.955 | 3.979 |
| Au (225) | 4.067 | 4.087 | 4.072 | 4.070 | 4.072 | 4.072 | 4.119 | 4.141 | 4.183 |
| ME | | -0.008 | -0.024 | -0.014 | -0.021 | -0.024 | -0.002 | -0.019 | 0.037 |
| MAE | | 0.043 | 0.036 | 0.034 | 0.035 | 0.036 | 0.036 | 0.043 | 0.050 |
| MRE | | -0.3 | -0.6 | -0.4 | -0.5 | -0.6 | -0.1 | -0.4 | 0.7 |
| MARE | | 0.9 | 0.8 | 0.7 | 0.7 | 0.8 | 0.8 | 1.0 | 1.1 |

TABLE S2. Equilibrium lattice constant $a_0$ (in Å) of 44 solids. All results were obtained non-self-consistently using PBE orbitals/density. The space group number is indicated in parenthesis.

| Solid | SCAN | SCAN(GEA2L) | SCAN(TW02L) | SCAN(PC) | SCAN(CR) | SCAN(GEAloc) | SCAN(PCopt) | SCAN(CRopt) |
|---|---|---|---|---|---|---|---|---|
| C (227) | 3.556 | 3.578 | 3.580 | 3.582 | 3.577 | 3.589 | 3.573 | 3.587 |
| Si (227) | 5.434 | 5.437 | 5.439 | 5.440 | 5.437 | 5.449 | 5.432 | 5.460 |
| Ge (227) | 5.670 | 5.691 | 5.694 | 5.692 | 5.691 | 5.717 | 5.690 | 5.735 |
| Sn (227) | 6.552 | 6.558 | 6.563 | 6.560 | 6.558 | 6.606 | 6.574 | 6.624 |
| SiC (216) | 4.360 | 4.378 | 4.380 | 4.381 | 4.377 | 4.385 | 4.364 | 4.388 |
| BN (216) | 3.607 | 3.627 | 3.630 | 3.632 | 3.627 | 3.634 | 3.614 | 3.631 |
| BP (216) | 4.529 | 4.543 | 4.545 | 4.547 | 4.542 | 4.558 | 4.540 | 4.559 |
| AlN (216) | 4.370 | 4.390 | 4.393 | 4.393 | 4.390 | 4.392 | 4.371 | 4.401 |
| AlP (216) | 5.482 | 5.480 | 5.482 | 5.481 | 5.479 | 5.487 | 5.468 | 5.502 |
| AlAs (216) | 5.682 | 5.680 | 5.683 | 5.681 | 5.680 | 5.693 | 5.675 | 5.710 |
| GaN (216) | 4.499 | 4.523 | 4.525 | 4.526 | 4.523 | 4.536 | 4.517 | 4.546 |
| GaP (216) | 5.446 | 5.460 | 5.463 | 5.462 | 5.460 | 5.483 | 5.453 | 5.499 |
| GaAs (216) | 5.664 | 5.672 | 5.675 | 5.674 | 5.672 | 5.703 | 5.684 | 5.725 |
| InP (216) | 5.898 | 5.895 | 5.898 | 5.896 | 5.895 | 5.923 | 5.901 | 5.938 |
| InAs (216) | 6.097 | 6.087 | 6.089 | 6.088 | 6.086 | 6.126 | 6.112 | 6.148 |
| InSb (216) | 6.534 | 6.518 | 6.522 | 6.519 | 6.518 | 6.564 | 6.543 | 6.580 |
| LiH (225) | 3.995 | 3.982 | 3.997 | 3.991 | 3.981 | 3.989 | 3.966 | 3.980 |
| LiF (225) | 3.986 | 4.002 | 4.017 | 4.011 | 4.001 | 4.010 | 3.985 | 4.027 |
| LiCl (225) | 5.096 | 5.069 | 5.084 | 5.079 | 5.068 | 5.092 | 5.065 | 5.111 |
| NaF (225) | 4.577 | 4.579 | 4.590 | 4.580 | 4.579 | 4.598 | 4.574 | 4.652 |
| NaCl (225) | 5.593 | 5.557 | 5.572 | 5.558 | 5.557 | 5.583 | 5.559 | 5.654 |
| MgO (225) | 4.204 | 4.220 | 4.224 | 4.222 | 4.219 | 4.228 | 4.207 | 4.248 |
| Li (229) | 3.471 | 3.455 | 3.471 | 3.466 | 3.454 | 3.465 | 3.429 | 3.453 |
| Na (229) | 4.205 | 4.147 | 4.158 | 4.146 | 4.147 | 4.172 | 4.166 | 4.228 |
| Al (225) | 4.012 | 4.006 | 4.008 | 4.007 | 4.006 | 4.008 | 4.011 | 4.020 |
| K (229) | 5.341 | 5.223 | 5.244 | 5.221 | 5.223 | 5.270 | 5.255 | 5.344 |
| Ca (225) | 5.555 | 5.518 | 5.527 | 5.519 | 5.518 | 5.557 | 5.522 | 5.578 |
| Rb (229) | 5.690 | 5.562 | 5.577 | 5.562 | 5.563 | 5.623 | 5.604 | 5.700 |
| Sr (225) | 6.077 | 5.998 | 6.008 | 5.998 | 5.998 | 6.050 | 6.023 | 6.082 |
| Cs (229) | 6.272 | 6.088 | 6.113 | 6.086 | 6.088 | 6.184 | 6.152 | 6.251 |
| Ba (229) | 5.042 | 4.987 | 4.996 | 4.988 | 4.987 | 5.076 | 5.032 | 5.096 |
| V (229) | 2.966 | 2.974 | 2.975 | 2.974 | 2.974 | 2.997 | 2.981 | 3.004 |
| Ni (225) | 3.456 | 3.458 | 3.459 | 3.458 | 3.458 | 3.488 | 3.472 | 3.496 |
| Cu (225) | 3.559 | 3.561 | 3.563 | 3.563 | 3.561 | 3.589 | 3.573 | 3.597 |
| Nb (229) | 3.294 | 3.296 | 3.296 | 3.296 | 3.296 | 3.321 | 3.303 | 3.326 |
| Mo (229) | 3.143 | 3.145 | 3.145 | 3.145 | 3.145 | 3.165 | 3.151 | 3.170 |
| Rh (225) | 3.783 | 3.793 | 3.793 | 3.793 | 3.793 | 3.827 | 3.809 | 3.831 |
| Pd (225) | 3.888 | 3.889 | 3.890 | 3.890 | 3.889 | 3.935 | 3.913 | 3.936 |
| Ag (225) | 4.084 | 4.073 | 4.076 | 4.074 | 4.073 | 4.133 | 4.104 | 4.134 |
| Ta (229) | 3.274 | 3.274 | 3.275 | 3.275 | 3.274 | 3.299 | 3.296 | 3.310 |
| W (229) | 3.149 | 3.150 | 3.150 | 3.150 | 3.150 | 3.167 | 3.164 | 3.175 |
| Ir (225) | 3.802 | 3.818 | 3.818 | 3.818 | 3.818 | 3.844 | 3.839 | 3.850 |
| Pt (225) | 3.907 | 3.920 | 3.920 | 3.920 | 3.920 | 3.955 | 3.942 | 3.955 |
| Au (225) | 4.093 | 4.094 | 4.096 | 4.096 | 4.094 | 4.144 | 4.122 | 4.133 |
| ME | 0.018 | 0.005 | 0.011 | 0.007 | 0.005 | 0.034 | 0.014 | 0.051 |
| MAE | 0.030 | 0.027 | 0.028 | 0.029 | 0.027 | 0.039 | 0.028 | 0.053 |
| MRE | 0.3 | 0.1 | 0.2 | 0.1 | 0.1 | 0.7 | 0.2 | 1.0 |
| MARE | 0.6 | 0.6 | 0.6 | 0.6 | 0.6 | 0.8 | 0.6 | 1.1 |

TABLE S3. Equilibrium lattice constant $a_0$ (in Å) of 44 solids. All results were obtained non-self-consistently using PBE orbitals/density. The space group number is indicated in parenthesis.

| Solid | TM | TM(GEA2L) | TM(TW02L) | TM(PC) | TM(CR) | TM(GEAloc) | TM(PCopt) | TM(CRopt) |
|---|---|---|---|---|---|---|---|---|
| C (227) | 3.555 | 3.557 | 3.558 | 3.558 | 3.557 | 3.557 | 3.561 | 3.557 |
| Si (227) | 5.416 | 5.415 | 5.415 | 5.414 | 5.415 | 5.411 | 5.422 | 5.420 |
| Ge (227) | 5.651 | 5.656 | 5.656 | 5.655 | 5.656 | 5.640 | 5.660 | 5.665 |
| Sn (227) | 6.527 | 6.524 | 6.523 | 6.524 | 6.525 | 6.506 | 6.528 | 6.538 |
| SiC (216) | 4.353 | 4.355 | 4.356 | 4.356 | 4.355 | 4.354 | 4.359 | 4.357 |
| BN (216) | 3.610 | 3.611 | 3.611 | 3.612 | 3.610 | 3.611 | 3.615 | 3.611 |
| BP (216) | 4.514 | 4.514 | 4.514 | 4.515 | 4.514 | 4.514 | 4.521 | 4.516 |
| AlN (216) | 4.379 | 4.380 | 4.380 | 4.380 | 4.379 | 4.379 | 4.385 | 4.385 |
| AlP (216) | 5.462 | 5.455 | 5.455 | 5.454 | 5.455 | 5.450 | 5.461 | 5.461 |
| AlAs (216) | 5.661 | 5.657 | 5.657 | 5.656 | 5.657 | 5.645 | 5.658 | 5.661 |
| GaN (216) | 4.506 | 4.509 | 4.509 | 4.509 | 4.509 | 4.511 | 4.523 | 4.523 |
| GaP (216) | 5.434 | 5.432 | 5.431 | 5.430 | 5.432 | 5.430 | 5.448 | 5.448 |
| GaAs (216) | 5.643 | 5.645 | 5.644 | 5.644 | 5.645 | 5.631 | 5.651 | 5.656 |
| InP (216) | 5.884 | 5.879 | 5.878 | 5.878 | 5.879 | 5.882 | 5.902 | 5.903 |
| InAs (216) | 6.082 | 6.080 | 6.079 | 6.078 | 6.080 | 6.069 | 6.091 | 6.098 |
| InSb (216) | 6.516 | 6.511 | 6.510 | 6.509 | 6.511 | 6.497 | 6.521 | 6.532 |
| LiH (225) | 3.938 | 3.955 | 3.959 | 3.950 | 3.954 | 3.932 | 3.935 | 3.936 |
| LiF (225) | 3.973 | 3.984 | 3.987 | 3.979 | 3.984 | 3.968 | 3.979 | 3.987 |
| LiCl (225) | 5.050 | 5.037 | 5.040 | 5.030 | 5.037 | 5.022 | 5.040 | 5.050 |
| NaF (225) | 4.590 | 4.594 | 4.598 | 4.585 | 4.593 | 4.577 | 4.595 | 4.614 |
| NaCl (225) | 5.567 | 5.551 | 5.557 | 5.537 | 5.551 | 5.528 | 5.550 | 5.578 |
| MgO (225) | 4.218 | 4.222 | 4.223 | 4.221 | 4.222 | 4.222 | 4.231 | 4.235 |
| Li (229) | 3.403 | 3.402 | 3.406 | 3.401 | 3.401 | 3.384 | 3.393 | 3.387 |
| Na (229) | 4.131 | 4.119 | 4.125 | 4.115 | 4.120 | 4.097 | 4.119 | 4.130 |
| Al (225) | 3.986 | 3.988 | 3.989 | 3.987 | 3.988 | 3.982 | 3.988 | 3.988 |
| K (229) | 5.210 | 5.179 | 5.187 | 5.174 | 5.179 | 5.158 | 5.188 | 5.203 |
| Ca (225) | 5.494 | 5.485 | 5.487 | 5.484 | 5.485 | 5.494 | 5.504 | 5.512 |
| Rb (229) | 5.575 | 5.526 | 5.552 | 5.541 | 5.546 | 5.527 | 5.564 | 5.581 |
| Sr (225) | 5.972 | 5.956 | 5.958 | 5.955 | 5.956 | 5.962 | 5.981 | 5.993 |
| Cs (229) | 6.084 | 6.038 | 6.046 | 6.033 | 6.036 | 6.033 | 6.076 | 6.093 |
| Ba (229) | 4.967 | 4.952 | 4.954 | 4.952 | 4.952 | 4.968 | 4.990 | 5.004 |
| V (229) | 2.982 | 2.979 | 2.978 | 2.978 | 2.979 | 2.985 | 2.990 | 2.993 |
| Ni (225) | 3.465 | 3.463 | 3.463 | 3.460 | 3.463 | 3.457 | 3.467 | 3.473 |
| Cu (225) | 3.559 | 3.559 | 3.559 | 3.561 | 3.560 | 3.552 | 3.564 | 3.568 |
| Nb (229) | 3.292 | 3.289 | 3.289 | 3.289 | 3.289 | 3.297 | 3.303 | 3.305 |
| Mo (229) | 3.142 | 3.139 | 3.138 | 3.139 | 3.139 | 3.144 | 3.149 | 3.150 |
| Rh (225) | 3.792 | 3.787 | 3.787 | 3.787 | 3.787 | 3.790 | 3.797 | 3.799 |
| Pd (225) | 3.890 | 3.884 | 3.883 | 3.885 | 3.884 | 3.885 | 3.895 | 3.901 |
| Ag (225) | 4.069 | 4.063 | 4.063 | 4.061 | 4.063 | 4.058 | 4.074 | 4.085 |
| Ta (229) | 3.290 | 3.292 | 3.291 | 3.292 | 3.292 | 3.292 | 3.298 | 3.301 |
| W (229) | 3.158 | 3.158 | 3.158 | 3.158 | 3.158 | 3.158 | 3.163 | 3.164 |
| Ir (225) | 3.835 | 3.833 | 3.832 | 3.833 | 3.833 | 3.834 | 3.840 | 3.841 |
| Pt (225) | 3.921 | 3.918 | 3.918 | 3.919 | 3.918 | 3.919 | 3.927 | 3.929 |
| Au (225) | 4.091 | 4.090 | 4.089 | 4.090 | 4.090 | 4.090 | 4.102 | 4.107 |
| ME | -0.006 | -0.011 | -0.010 | -0.013 | -0.011 | -0.016 | -0.003 | 0.003 |
| MAE | 0.023 | 0.025 | 0.024 | 0.026 | 0.025 | 0.026 | 0.026 | 0.027 |
| MRE | -0.2 | -0.3 | -0.2 | -0.3 | -0.3 | -0.4 | -0.1 | 0.0 |
| MARE | 0.5 | 0.5 | 0.5 | 0.6 | 0.5 | 0.6 | 0.6 | 0.6 |

TABLE S4. Bulk modulus $B_0$ (in GPa) of 44 solids. The experimental values are from Refs. 1 and 2. All results were obtained non-self-consistently using PBE orbitals/density. The space group number is indicated in parenthesis.

| Solid | Expt. | MVS | MVS(GEA2L) | MVS(TW02L) | MVS(PC) | MVS(CR) | MVS(GEAloc) | MVS(PCopt) | MVS(CRopt) |
|---|---|---|---|---|---|---|---|---|---|
| C (227) | 454.7 | 475.4 | 443.5 | 440.9 | 436.5 | 444.2 | 451.9 | 476.0 | 453.9 |
| Si (227) | 101.3 | 106.3 | 102.3 | 101.9 | 101.6 | 102.3 | 102.4 | 105.2 | 100.8 |
| Ge (227) | 79.4 | 90.0 | 81.2 | 81.2 | 81.5 | 81.3 | 81.5 | 84.5 | 74.3 |
| Sn (227) | 42.8 | 54.5 | 51.1 | 51.0 | 51.0 | 51.1 | 49.4 | 49.7 | 44.5 |
| SiC (216) | 229.1 | 247.8 | 227.3 | 226.2 | 225.6 | 227.5 | 226.7 | 234.1 | 225.8 |
| BN (216) | 410.2 | 422.1 | 399.9 | 397.4 | 393.7 | 400.5 | 400.2 | 413.1 | 400.8 |
| BP (216) | 168.0 | 178.0 | 170.8 | 169.9 | 168.9 | 171.0 | 170.3 | 177.3 | 169.7 |
| AlN (216) | 206.0 | 233.6 | 226.3 | 224.2 | 224.2 | 226.5 | 230.9 | 236.6 | 226.4 |
| AlP (216) | 87.4 | 100.6 | 98.2 | 97.8 | 97.9 | 98.2 | 98.3 | 99.7 | 96.0 |
| AlAs (216) | 75.0 | 88.2 | 84.1 | 83.8 | 83.9 | 84.1 | 83.3 | 83.2 | 79.1 |
| GaN (216) | 213.7 | 232.3 | 206.6 | 205.3 | 204.9 | 206.7 | 204.9 | 213.8 | 198.0 |
| GaP (216) | 89.6 | 104.9 | 97.9 | 97.5 | 97.6 | 98.0 | 98.5 | 103.1 | 93.3 |
| GaAs (216) | 76.7 | 89.2 | 79.6 | 79.5 | 79.5 | 79.6 | 77.9 | 80.5 | 71.3 |
| InP (216) | 72.0 | 79.5 | 75.0 | 74.6 | 74.8 | 75.0 | 73.1 | 74.5 | 68.6 |
| InAs (216) | 58.6 | 68.0 | 61.6 | 61.5 | 61.5 | 61.6 | 58.5 | 59.8 | 52.9 |
| InSb (216) | 46.1 | 50.8 | 48.6 | 48.5 | 48.6 | 48.6 | 46.1 | 46.2 | 40.9 |
| LiH (225) | 40.1 | 36.0 | 40.4 | 39.3 | 39.6 | 40.5 | 39.0 | 39.5 | 38.7 |
| LiF (225) | 76.3 | 84.0 | 86.0 | 82.2 | 83.7 | 86.1 | 85.8 | 90.3 | 80.7 |
| LiCl (225) | 38.7 | 36.6 | 41.4 | 39.6 | 40.6 | 41.5 | 39.7 | 40.5 | 35.4 |
| NaF (225) | 53.1 | 56.9 | 59.9 | 56.1 | 59.9 | 59.8 | 58.9 | 61.1 | 48.9 |
| NaCl (225) | 27.6 | 27.0 | 31.5 | 29.4 | 31.6 | 31.5 | 30.6 | 31.2 | 23.5 |
| MgO (225) | 169.8 | 192.2 | 171.3 | 167.8 | 170.5 | 171.7 | 173.6 | 185.2 | 170.4 |
| Li (229) | 13.1 | 13.8 | 14.4 | 13.9 | 14.0 | 14.5 | 14.3 | 16.5 | 14.5 |
| Na (229) | 7.9 | 8.1 | 8.7 | 8.4 | 8.8 | 8.7 | 8.5 | 8.8 | 7.7 |
| Al (225) | 77.1 | 121.0 | 92.6 | 92.4 | 92.5 | 92.7 | 89.8 | 93.5 | 87.1 |
| K (229) | 3.8 | 3.4 | 3.9 | 3.8 | 4.0 | 3.9 | 3.8 | 4.0 | 3.4 |
| Ca (225) | 15.9 | 20.5 | 19.6 | 19.5 | 19.6 | 19.6 | 19.4 | 19.8 | 19.0 |
| Rb (229) | 3.6 | 2.8 | 3.1 | 3.0 | 3.1 | 3.1 | 3.0 | 3.1 | 2.8 |
| Sr (225) | 12.0 | 12.3 | 12.8 | 12.5 | 12.8 | 12.8 | 12.6 | 13.0 | 12.1 |
| Cs (229) | 2.3 | 1.8 | 2.0 | 2.0 | 2.0 | 2.0 | 2.0 | 2.0 | 1.9 |
| Ba (229) | 10.6 | 8.7 | 9.2 | 9.0 | 9.2 | 9.2 | 9.3 | 9.5 | 8.9 |
| V (229) | 165.8 | 205.3 | 200.5 | 199.7 | 200.5 | 200.5 | 193.1 | 195.8 | 185.2 |
| Ni (225) | 192.5 | 243.7 | 251.5 | 251.3 | 253.5 | 251.6 | 230.7 | 220.4 | 203.1 |
| Cu (225) | 144.3 | 191.1 | 204.5 | 204.3 | 202.8 | 204.4 | 188.2 | 178.0 | 167.8 |
| Nb (229) | 173.2 | 181.2 | 181.2 | 180.6 | 181.3 | 181.2 | 176.1 | 178.1 | 170.8 |
| Mo (229) | 276.2 | 284.9 | 277.7 | 277.3 | 277.7 | 277.7 | 267.4 | 269.9 | 257.9 |
| Rh (225) | 277.1 | 306.1 | 301.8 | 302.3 | 302.1 | 301.8 | 277.2 | 272.4 | 253.1 |
| Pd (225) | 187.2 | 205.0 | 206.9 | 207.2 | 207.0 | 207.0 | 181.9 | 173.5 | 152.8 |
| Ag (225) | 105.7 | 119.8 | 126.0 | 125.7 | 127.2 | 126.0 | 107.6 | 99.9 | 83.0 |
| Ta (229) | 202.7 | 210.3 | 210.2 | 210.0 | 210.3 | 210.2 | 203.7 | 205.0 | 196.2 |
| W (229) | 327.5 | 336.7 | 330.3 | 330.5 | 330.3 | 330.3 | 318.2 | 317.7 | 305.8 |
| Ir (225) | 362.2 | 394.9 | 392.6 | 394.1 | 392.8 | 392.6 | 365.1 | 353.8 | 341.6 |
| Pt (225) | 285.5 | 288.0 | 295.0 | 296.3 | 295.0 | 295.0 | 267.0 | 252.3 | 236.4 |
| Au (225) | 182.0 | 169.5 | 178.3 | 178.8 | 178.3 | 178.3 | 154.5 | 141.6 | 124.2 |
| ME | | 12.2 | 8.3 | 7.6 | 7.7 | 8.3 | 3.0 | 3.8 | -4.9 |
| MAE | | 13.3 | 9.9 | 9.7 | 10.1 | 9.9 | 7.4 | 9.5 | 10.0 |
| MRE | | 8.2 | 7.1 | 5.7 | 6.7 | 7.1 | 3.5 | 5.2 | -3.6 |
| MARE | | 12.7 | 9.4 | 8.7 | 9.2 | 9.4 | 7.4 | 9.5 | 9.0 |

TABLE S5. Bulk modulus $B_0$ (in GPa) of 44 solids. All results were obtained non-self-consistently using PBE orbitals/density. The space group number is indicated in parenthesis.

| Solid | SCAN | SCAN(GEA2L) | SCAN(TW02L) | SCAN(PC) | SCAN(CR) | SCAN(GEAloc) | SCAN(PCopt) | SCAN(CRopt) |
|---|---|---|---|---|---|---|---|---|
| C (227) | 461.3 | 422.5 | 421.0 | 418.6 | 423.0 | 415.3 | 435.2 | 417.1 |
| Si (227) | 98.8 | 92.4 | 92.2 | 91.7 | 92.4 | 92.3 | 94.9 | 91.1 |
| Ge (227) | 71.1 | 63.3 | 63.0 | 63.3 | 63.3 | 61.0 | 64.9 | 59.1 |
| Sn (227) | 41.6 | 39.6 | 39.3 | 39.4 | 39.6 | 37.9 | 39.0 | 36.7 |
| SiC (216) | 226.0 | 214.1 | 213.4 | 213.1 | 214.3 | 212.1 | 219.2 | 211.6 |
| BN (216) | 397.4 | 373.4 | 371.5 | 370.4 | 373.8 | 370.9 | 385.4 | 372.6 |
| BP (216) | 172.4 | 162.2 | 161.7 | 161.2 | 162.4 | 159.6 | 165.1 | 159.3 |
| AlN (216) | 216.0 | 198.3 | 197.2 | 197.2 | 198.3 | 199.2 | 208.1 | 197.2 |
| AlP (216) | 90.8 | 86.7 | 86.4 | 86.5 | 86.7 | 86.8 | 89.1 | 85.5 |
| AlAs (216) | 76.2 | 72.9 | 72.6 | 72.7 | 72.9 | 72.4 | 74.3 | 71.1 |
| GaN (216) | 200.7 | 182.2 | 181.3 | 181.1 | 182.3 | 179.1 | 186.4 | 175.2 |
| GaP (216) | 87.9 | 79.6 | 79.3 | 79.3 | 79.6 | 78.0 | 81.9 | 75.4 |
| GaAs (216) | 70.5 | 65.9 | 65.7 | 65.7 | 65.9 | 64.0 | 64.9 | 60.8 |
| InP (216) | 69.9 | 65.6 | 65.3 | 65.4 | 65.6 | 63.7 | 66.4 | 62.0 |
| InAs (216) | 58.3 | 55.3 | 55.0 | 55.1 | 55.3 | 52.3 | 54.1 | 50.4 |
| InSb (216) | 44.3 | 42.8 | 42.5 | 42.7 | 42.8 | 40.6 | 42.2 | 39.6 |
| LiH (225) | 36.6 | 37.2 | 36.2 | 36.7 | 37.2 | 37.0 | 37.9 | 37.3 |
| LiF (225) | 75.9 | 74.2 | 71.6 | 73.3 | 74.3 | 73.4 | 76.8 | 72.1 |
| LiCl (225) | 35.6 | 37.1 | 35.9 | 36.7 | 37.1 | 36.6 | 37.6 | 34.6 |
| NaF (225) | 57.5 | 56.5 | 55.1 | 56.4 | 56.5 | 55.2 | 57.5 | 49.4 |
| NaCl (225) | 28.0 | 28.6 | 27.8 | 28.7 | 28.7 | 27.9 | 28.9 | 25.2 |
| MgO (225) | 171.5 | 159.0 | 157.6 | 158.5 | 159.1 | 156.9 | 162.8 | 153.0 |
| Li (229) | 13.1 | 12.8 | 12.8 | 13.0 | 12.8 | 12.8 | 13.1 | 12.7 |
| Na (229) | 7.7 | 8.4 | 8.2 | 8.4 | 8.4 | 8.6 | 8.1 | 8.0 |
| Al (225) | 80.1 | 87.7 | 87.7 | 87.6 | 87.8 | 92.1 | 81.9 | 89.9 |
| K (229) | 3.3 | 3.8 | 3.7 | 3.8 | 3.8 | 3.8 | 3.7 | 3.5 |
| Ca (225) | 17.7 | 18.8 | 18.7 | 18.8 | 18.8 | 19.7 | 18.4 | 19.1 |
| Rb (229) | 2.8 | 3.3 | 3.2 | 3.3 | 3.2 | 3.2 | 3.2 | 2.9 |
| Sr (225) | 11.1 | 12.7 | 12.6 | 12.7 | 12.7 | 12.8 | 12.6 | 12.3 |
| Cs (229) | 1.9 | 2.1 | 2.1 | 2.1 | 2.1 | 2.1 | 2.1 | 2.0 |
| Ba (229) | 8.6 | 9.2 | 9.1 | 9.2 | 9.2 | 9.2 | 9.0 | 8.9 |
| V (229) | 194.6 | 196.1 | 195.5 | 195.8 | 196.1 | 189.9 | 189.4 | 185.3 |
| Ni (225) | 225.2 | 230.8 | 229.1 | 230.8 | 230.8 | 212.5 | 220.4 | 208.6 |
| Cu (225) | 172.6 | 173.0 | 171.3 | 172.0 | 173.0 | 162.2 | 167.6 | 158.5 |
| Nb (229) | 177.8 | 178.7 | 178.3 | 178.7 | 178.7 | 172.1 | 176.5 | 170.8 |
| Mo (229) | 274.5 | 274.6 | 274.2 | 274.5 | 274.6 | 260.8 | 269.1 | 259.1 |
| Rh (225) | 300.6 | 291.6 | 290.6 | 291.2 | 291.6 | 265.1 | 276.3 | 263.9 |
| Pd (225) | 193.4 | 196.9 | 195.3 | 196.4 | 196.9 | 170.5 | 180.9 | 171.9 |
| Ag (225) | 107.4 | 112.6 | 111.0 | 112.7 | 112.6 | 94.9 | 102.2 | 95.4 |
| Ta (229) | 203.9 | 206.0 | 205.9 | 205.7 | 206.4 | 200.4 | 201.5 | 196.2 |
| W (229) | 322.9 | 323.7 | 323.8 | 323.5 | 323.7 | 312.1 | 316.7 | 306.7 |
| Ir (225) | 431.5 | 398.9 | 398.8 | 399.0 | 398.8 | 363.4 | 371.5 | 359.4 |
| Pt (225) | 292.6 | 280.8 | 279.7 | 280.2 | 280.8 | 253.1 | 263.8 | 257.6 |
| Au (225) | 168.1 | 168.9 | 167.6 | 168.2 | 168.9 | 147.7 | 156.2 | 154.8 |
| ME | 3.5 | -1.0 | -1.7 | -1.4 | -0.9 | -6.9 | -2.9 | -8.2 |
| MAE | 7.4 | 9.8 | 9.9 | 10.1 | 9.7 | 10.8 | 7.7 | 11.2 |
| MRE | -0.5 | -1.2 | -2.0 | -1.4 | -1.2 | -4.2 | -2.3 | -6.6 |
| MARE | 6.5 | 7.7 | 7.9 | 7.9 | 7.7 | 8.9 | 6.7 | 9.8 |

TABLE S6. Bulk modulus $B_0$ (in GPa) of 44 solids. All results were obtained non-self-consistently using PBE orbitals/density. The space group number is indicated in parenthesis.

| Solid | TM | TM(GEA2L) | TM(TW02L) | TM(PC) | TM(CR) | TM(GEAloc) | TM(PCopt) | TM(CRopt) |
|---|---|---|---|---|---|---|---|---|
| C (227) | 454.5 | 449.0 | 449.0 | 447.8 | 449.4 | 444.2 | 438.4 | 444.8 |
| Si (227) | 98.1 | 95.8 | 95.9 | 95.9 | 95.8 | 95.3 | 93.3 | 94.3 |
| Ge (227) | 72.4 | 70.5 | 70.6 | 71.1 | 70.5 | 72.8 | 70.0 | 69.3 |
| Sn (227) | 44.2 | 43.6 | 43.7 | 43.7 | 43.6 | 45.2 | 43.6 | 42.9 |
| SiC (216) | 228.2 | 223.7 | 223.7 | 224.0 | 223.8 | 222.5 | 219.3 | 221.8 |
| BN (216) | 390.8 | 384.9 | 384.8 | 384.4 | 385.2 | 381.7 | 378.0 | 381.0 |
| BP (216) | 172.5 | 171.0 | 171.1 | 170.8 | 170.6 | 169.7 | 166.9 | 169.0 |
| AlN (216) | 207.0 | 202.4 | 202.3 | 202.5 | 202.6 | 201.7 | 199.7 | 199.8 |
| AlP (216) | 91.1 | 89.8 | 89.8 | 90.0 | 89.8 | 90.2 | 88.7 | 88.9 |
| AlAs (216) | 76.7 | 75.4 | 75.5 | 75.6 | 75.5 | 77.1 | 75.6 | 75.3 |
| GaN (216) | 191.3 | 185.9 | 186.1 | 186.1 | 186.0 | 183.6 | 179.8 | 179.6 |
| GaP (216) | 88.0 | 86.5 | 86.6 | 86.7 | 86.6 | 85.9 | 83.5 | 83.6 |
| GaAs (216) | 73.2 | 71.6 | 71.8 | 71.8 | 71.6 | 73.2 | 70.7 | 70.1 |
| InP (216) | 68.2 | 67.1 | 67.2 | 67.3 | 67.1 | 66.2 | 64.3 | 64.0 |
| InAs (216) | 57.6 | 56.9 | 56.9 | 57.0 | 56.8 | 57.8 | 55.9 | 55.1 |
| InSb (216) | 44.4 | 44.0 | 44.0 | 44.1 | 43.9 | 45.0 | 43.4 | 42.6 |
| LiH (225) | 40.4 | 39.2 | 39.0 | 39.4 | 39.2 | 40.5 | 40.4 | 40.4 |
| LiF (225) | 78.5 | 77.5 | 76.9 | 78.4 | 77.6 | 79.6 | 78.5 | 76.9 |
| LiCl (225) | 38.3 | 38.2 | 37.8 | 38.8 | 38.2 | 39.7 | 38.6 | 37.9 |
| NaF (225) | 54.7 | 53.8 | 53.0 | 55.3 | 53.9 | 56.0 | 54.5 | 52.3 |
| NaCl (225) | 29.0 | 29.1 | 28.8 | 29.8 | 29.1 | 30.2 | 29.4 | 28.2 |
| MgO (225) | 164.4 | 158.9 | 158.5 | 159.3 | 159.1 | 158.7 | 157.0 | 156.0 |
| Li (229) | 14.5 | 14.6 | 14.5 | 14.6 | 14.6 | 15.0 | 14.8 | 14.9 |
| Na (229) | 8.6 | 8.7 | 8.7 | 8.8 | 8.7 | 9.0 | 8.8 | 8.7 |
| Al (225) | 91.7 | 89.7 | 89.6 | 89.4 | 89.7 | 90.6 | 89.3 | 90.2 |
| K (229) | 4.0 | 4.0 | 3.9 | 4.1 | 4.0 | 4.2 | 3.9 | 3.9 |
| Ca (225) | 18.9 | 19.1 | 19.1 | 19.2 | 19.1 | 19.6 | 19.3 | 19.4 |
| Rb (229) | 3.2 | 3.3 | 3.2 | 3.3 | 3.2 | 3.4 | 3.2 | 3.1 |
| Sr (225) | 12.8 | 12.9 | 12.8 | 12.9 | 12.9 | 13.0 | 12.8 | 12.7 |
| Cs (229) | 2.1 | 2.2 | 2.2 | 2.2 | 2.2 | 2.2 | 2.2 | 2.2 |
| Ba (229) | 9.3 | 9.3 | 9.3 | 9.3 | 9.3 | 9.5 | 9.3 | 9.3 |
| V (229) | 194.5 | 196.5 | 196.4 | 196.6 | 196.5 | 198.3 | 196.2 | 194.7 |
| Ni (225) | 230.6 | 232.1 | 232.0 | 233.4 | 232.2 | 235.9 | 230.4 | 225.4 |
| Cu (225) | 180.6 | 178.3 | 178.2 | 179.5 | 177.6 | 184.7 | 177.1 | 175.1 |
| Nb (229) | 177.2 | 178.2 | 178.2 | 178.3 | 178.2 | 177.8 | 176.1 | 174.8 |
| Mo (229) | 273.3 | 275.3 | 275.5 | 275.4 | 275.3 | 274.3 | 271.2 | 269.6 |
| Rh (225) | 289.8 | 292.8 | 293.2 | 292.7 | 292.8 | 292.6 | 287.2 | 283.8 |
| Pd (225) | 195.7 | 198.1 | 198.3 | 197.9 | 198.1 | 198.9 | 193.4 | 188.1 |
| Ag (225) | 113.3 | 113.8 | 113.9 | 115.6 | 113.9 | 115.9 | 110.7 | 105.9 |
| Ta (229) | 205.5 | 205.3 | 205.2 | 205.2 | 205.2 | 206.1 | 203.8 | 203.0 |
| W (229) | 323.7 | 324.2 | 324.5 | 324.5 | 324.3 | 325.6 | 321.8 | 320.9 |
| Ir (225) | 383.4 | 385.5 | 385.8 | 385.2 | 385.5 | 384.2 | 379.5 | 377.5 |
| Pt (225) | 284.7 | 286.1 | 286.6 | 285.8 | 286.1 | 286.0 | 279.8 | 276.8 |
| Au (225) | 170.3 | 168.5 | 168.8 | 167.7 | 168.5 | 168.9 | 162.0 | 159.2 |
| ME | 2.4 | 1.6 | 1.6 | 1.7 | 1.6 | 2.0 | -0.5 | -1.2 |
| MAE | 6.6 | 7.5 | 7.5 | 7.6 | 7.5 | 8.2 | 8.3 | 7.6 |
| MRE | 2.1 | 1.5 | 1.3 | 2.0 | 1.5 | 2.9 | 0.5 | -0.3 |
| MARE | 6.2 | 6.6 | 6.5 | 6.8 | 6.6 | 7.4 | 7.1 | 6.7 |

TABLE S7. Cohesive energy $E_{coh}$ (in eV/atom) of 44 solids. The experimental values are from Refs. 1 and 2. All results were obtained non-self-consistently using PBE orbitals/density. The space group number is indicated in parenthesis.

| Solid | Expt. | MVS | MVS(GEA2L) | MVS(TW02L) | MVS(PC) | MVS(CR) | MVS(GEAloc) | MVS(PCopt) | MVS(CRopt) |
|---|---|---|---|---|---|---|---|---|---|
| C (227) | 7.55 | 7.94 | 7.64 | 7.48 | 7.46 | 7.70 | 7.46 | 7.89 | 7.45 |
| Si (227) | 4.68 | 5.10 | 4.94 | 4.85 | 4.81 | 4.96 | 4.82 | 5.04 | 4.71 |
| Ge (227) | 3.89 | 4.14 | 3.85 | 3.73 | 3.84 | 3.85 | 3.59 | 3.72 | 3.26 |
| Sn (227) | 3.16 | 3.37 | 3.33 | 3.25 | 3.34 | 3.33 | 3.04 | 3.04 | 2.58 |
| SiC (216) | 6.48 | 7.00 | 6.58 | 6.45 | 6.42 | 6.62 | 6.44 | 6.77 | 6.39 |
| BN (216) | 6.76 | 7.12 | 6.89 | 6.75 | 6.65 | 6.97 | 6.70 | 7.05 | 6.74 |
| BP (216) | 5.14 | 5.58 | 5.42 | 5.31 | 5.24 | 5.47 | 5.25 | 5.56 | 5.22 |
| AlN (216) | 5.85 | 6.16 | 5.83 | 5.69 | 5.65 | 5.88 | 5.74 | 6.04 | 5.76 |
| AlP (216) | 4.32 | 4.61 | 4.41 | 4.32 | 4.31 | 4.44 | 4.32 | 4.49 | 4.24 |
| AlAs (216) | 3.82 | 4.12 | 3.84 | 3.74 | 3.76 | 3.86 | 3.66 | 3.86 | 3.49 |
| GaN (216) | 4.55 | 4.94 | 4.59 | 4.46 | 4.50 | 4.63 | 4.43 | 4.66 | 4.26 |
| GaP (216) | 3.61 | 4.07 | 3.84 | 3.74 | 3.80 | 3.86 | 3.71 | 3.88 | 3.50 |
| GaAs (216) | 3.34 | 3.55 | 3.31 | 3.20 | 3.29 | 3.31 | 3.05 | 3.20 | 2.75 |
| InP (216) | 3.47 | 3.64 | 3.51 | 3.41 | 3.49 | 3.52 | 3.35 | 3.44 | 3.06 |
| InAs (216) | 3.08 | 3.20 | 3.06 | 2.95 | 3.05 | 3.06 | 2.79 | 2.89 | 2.44 |
| InSb (216) | 2.81 | 2.81 | 2.78 | 2.69 | 2.78 | 2.78 | 2.49 | 2.52 | 2.10 |
| LiH (225) | 2.49 | 2.39 | 2.39 | 2.33 | 2.33 | 2.40 | 2.35 | 2.41 | 2.38 |
| LiF (225) | 4.46 | 4.58 | 4.30 | 4.18 | 4.25 | 4.32 | 4.29 | 4.49 | 4.28 |
| LiCl (225) | 3.59 | 3.64 | 3.52 | 3.42 | 3.46 | 3.53 | 3.46 | 3.58 | 3.39 |
| NaF (225) | 3.97 | 4.18 | 3.87 | 3.74 | 3.84 | 3.88 | 3.84 | 4.01 | 3.83 |
| NaCl (225) | 3.34 | 3.48 | 3.34 | 3.25 | 3.29 | 3.35 | 3.31 | 3.41 | 3.20 |
| MgO (225) | 5.20 | 5.71 | 5.25 | 5.13 | 5.04 | 5.28 | 5.14 | 5.43 | 5.22 |
| Li (229) | 1.67 | 1.51 | 1.53 | 1.47 | 1.49 | 1.55 | 1.50 | 1.60 | 1.51 |
| Na (229) | 1.12 | 1.07 | 1.09 | 1.03 | 1.08 | 1.10 | 1.05 | 1.08 | 0.96 |
| Al (225) | 3.43 | 3.96 | 3.62 | 3.56 | 3.46 | 3.66 | 3.39 | 3.65 | 3.37 |
| K (229) | 0.94 | 0.86 | 0.91 | 0.86 | 0.91 | 0.92 | 0.88 | 0.90 | 0.79 |
| Ca (225) | 1.87 | 2.38 | 2.25 | 2.21 | 2.23 | 2.28 | 2.21 | 2.30 | 2.17 |
| Rb (229) | 0.86 | 0.82 | 0.85 | 0.81 | 0.85 | 0.86 | 0.82 | 0.84 | 0.77 |
| Sr (225) | 1.73 | 2.11 | 2.02 | 1.99 | 2.01 | 2.04 | 1.98 | 2.04 | 1.92 |
| Cs (229) | 0.81 | 0.74 | 0.80 | 0.76 | 0.79 | 0.80 | 0.77 | 0.79 | 0.69 |
| Ba (229) | 1.91 | 2.41 | 2.33 | 2.28 | 2.31 | 2.34 | 2.29 | 2.35 | 2.20 |
| V (229) | 5.35 | 5.18 | 5.92 | 5.78 | 5.92 | 5.92 | 5.29 | 5.01 | 4.73 |
| Ni (225) | 4.48 | 5.79 | 5.47 | 5.37 | 5.46 | 5.47 | 5.13 | 5.04 | 4.51 |
| Cu (225) | 3.51 | 4.67 | 4.74 | 4.66 | 4.74 | 4.74 | 4.44 | 4.22 | 3.80 |
| Nb (229) | 7.60 | 6.71 | 7.17 | 7.02 | 7.18 | 7.17 | 6.53 | 6.28 | 5.89 |
| Mo (229) | 6.86 | 5.78 | 6.95 | 6.79 | 6.96 | 6.95 | 6.28 | 5.82 | 5.41 |
| Rh (225) | 5.78 | 6.36 | 6.29 | 6.16 | 6.28 | 6.29 | 5.77 | 5.68 | 5.05 |
| Pd (225) | 3.93 | 4.35 | 4.65 | 4.56 | 4.66 | 4.65 | 4.07 | 3.75 | 3.29 |
| Ag (225) | 2.96 | 3.35 | 3.37 | 3.27 | 3.37 | 3.37 | 3.01 | 2.87 | 2.36 |
| Ta (229) | 8.13 | 8.41 | 8.58 | 8.52 | 8.56 | 8.59 | 7.86 | 7.82 | 7.43 |
| W (229) | 8.94 | 8.17 | 8.82 | 8.69 | 8.83 | 8.82 | 8.07 | 7.62 | 6.95 |
| Ir (225) | 6.99 | 7.17 | 7.59 | 7.51 | 7.58 | 7.59 | 6.60 | 6.44 | 5.76 |
| Pt (225) | 5.87 | 6.39 | 6.49 | 6.42 | 6.50 | 6.49 | 5.84 | 5.60 | 4.82 |
| Au (225) | 3.83 | 3.92 | 4.05 | 3.98 | 4.06 | 4.05 | 3.67 | 3.44 | 2.72 |
| ME | | 0.21 | 0.18 | 0.08 | 0.13 | 0.19 | -0.08 | -0.04 | -0.38 |
| MAE | | 0.37 | 0.24 | 0.24 | 0.24 | 0.25 | 0.22 | 0.29 | 0.44 |
| MRE | | 5.8 | 4.5 | 1.9 | 3.4 | 5.0 | -1.1 | 0.5 | -8.3 |
| MARE | | 9.3 | 6.3 | 6.7 | 6.3 | 6.5 | 5.9 | 6.8 | 10.8 |

TABLE S8. Cohesive energy $E_{coh}$ (in eV/atom) of 44 solids. All results were obtained non-self-consistently using PBE orbitals/density. The space group number is indicated in parenthesis.

| Solid | SCAN | SCAN(GEA2L) | SCAN(TW02L) | SCAN(PC) | SCAN(CR) | SCAN(GEAloc) | SCAN(PCopt) | SCAN(CRopt) |
|---|---|---|---|---|---|---|---|---|
| C (227) | 7.56 | 7.38 | 7.29 | 7.29 | 7.41 | 7.14 | 7.41 | 7.10 |
| Si (227) | 4.73 | 4.64 | 4.59 | 4.55 | 4.64 | 4.51 | 4.64 | 4.43 |
| Ge (227) | 3.96 | 3.95 | 3.89 | 3.95 | 3.95 | 3.66 | 3.73 | 3.50 |
| Sn (227) | 3.37 | 3.43 | 3.38 | 3.42 | 3.43 | 3.14 | 3.22 | 3.04 |
| SiC (216) | 6.49 | 6.28 | 6.21 | 6.18 | 6.29 | 6.10 | 6.33 | 6.06 |
| BN (216) | 6.88 | 6.81 | 6.72 | 6.70 | 6.84 | 6.64 | 6.85 | 6.63 |
| BP (216) | 5.34 | 5.25 | 5.18 | 5.16 | 5.27 | 5.08 | 5.25 | 5.04 |
| AlN (216) | 5.81 | 5.69 | 5.62 | 5.62 | 5.71 | 5.59 | 5.75 | 5.57 |
| AlP (216) | 4.25 | 4.18 | 4.14 | 4.14 | 4.20 | 4.07 | 4.18 | 4.00 |
| AlAs (216) | 3.88 | 3.87 | 3.83 | 3.83 | 3.88 | 3.68 | 3.75 | 3.57 |
| GaN (216) | 4.45 | 4.39 | 4.32 | 4.36 | 4.41 | 4.19 | 4.32 | 4.08 |
| GaP (216) | 3.64 | 3.57 | 3.51 | 3.55 | 3.57 | 3.38 | 3.49 | 3.25 |
| GaAs (216) | 3.33 | 3.35 | 3.29 | 3.34 | 3.35 | 3.08 | 3.13 | 2.91 |
| InP (216) | 3.28 | 3.27 | 3.22 | 3.25 | 3.27 | 3.06 | 3.16 | 2.96 |
| InAs (216) | 3.05 | 3.11 | 3.05 | 3.10 | 3.11 | 2.83 | 2.89 | 2.69 |
| InSb (216) | 2.80 | 2.88 | 2.83 | 2.87 | 2.88 | 2.60 | 2.67 | 2.48 |
| LiH (225) | 2.45 | 2.41 | 2.37 | 2.38 | 2.41 | 2.40 | 2.43 | 2.42 |
| LiF (225) | 4.42 | 4.24 | 4.17 | 4.20 | 4.24 | 4.17 | 4.32 | 4.17 |
| LiCl (225) | 3.52 | 3.44 | 3.39 | 3.39 | 3.44 | 3.40 | 3.48 | 3.34 |
| NaF (225) | 3.93 | 3.81 | 3.74 | 3.78 | 3.81 | 3.74 | 3.85 | 3.64 |
| NaCl (225) | 3.28 | 3.18 | 3.14 | 3.14 | 3.18 | 3.16 | 3.23 | 3.09 |
| MgO (225) | 5.25 | 5.05 | 4.99 | 4.95 | 5.07 | 4.99 | 5.15 | 4.97 |
| Li (229) | 1.58 | 1.56 | 1.52 | 1.54 | 1.57 | 1.54 | 1.56 | 1.55 |
| Na (229) | 1.07 | 1.10 | 1.08 | 1.09 | 1.10 | 1.08 | 1.08 | 1.01 |
| Al (225) | 3.60 | 3.56 | 3.53 | 3.49 | 3.57 | 3.42 | 3.50 | 3.42 |
| K (229) | 0.85 | 0.88 | 0.86 | 0.87 | 0.88 | 0.85 | 0.86 | 0.80 |
| Ca (225) | 2.08 | 2.07 | 2.05 | 2.06 | 2.08 | 2.05 | 2.10 | 2.03 |
| Rb (229) | 0.74 | 0.79 | 0.77 | 0.78 | 0.79 | 0.77 | 0.77 | 0.70 |
| Sr (225) | 1.80 | 1.79 | 1.77 | 1.78 | 1.79 | 1.76 | 1.81 | 1.72 |
| Cs (229) | 0.67 | 0.70 | 0.69 | 0.70 | 0.70 | 0.68 | 0.69 | 0.64 |
| Ba (229) | 2.06 | 2.04 | 2.02 | 2.03 | 2.04 | 1.98 | 2.05 | 1.94 |
| V (229) | 4.69 | 5.46 | 5.36 | 5.44 | 5.47 | 5.08 | 5.18 | 4.89 |
| Ni (225) | 4.61 | 4.81 | 4.75 | 4.80 | 4.82 | 4.33 | 4.60 | 4.20 |
| Cu (225) | 3.98 | 3.91 | 3.84 | 3.90 | 3.91 | 3.68 | 3.79 | 3.51 |
| Nb (229) | 6.62 | 7.16 | 7.07 | 7.15 | 7.16 | 6.55 | 6.71 | 6.37 |
| Mo (229) | 5.87 | 6.70 | 6.58 | 6.69 | 6.70 | 6.08 | 6.37 | 6.03 |
| Rh (225) | 5.48 | 5.89 | 5.81 | 5.88 | 5.90 | 5.15 | 5.52 | 5.14 |
| Pd (225) | 4.25 | 4.46 | 4.39 | 4.45 | 4.46 | 4.02 | 4.15 | 4.03 |
| Ag (225) | 2.89 | 2.93 | 2.86 | 2.92 | 2.93 | 2.61 | 2.74 | 2.59 |
| Ta (229) | 8.55 | 8.70 | 8.67 | 8.68 | 8.71 | 7.96 | 8.11 | 7.78 |
| W (229) | 8.75 | 8.89 | 8.79 | 8.88 | 8.89 | 8.14 | 8.47 | 7.84 |
| Ir (225) | 7.74 | 8.04 | 7.97 | 8.02 | 8.04 | 7.03 | 7.31 | 7.00 |
| Pt (225) | 6.18 | 6.33 | 6.27 | 6.32 | 6.33 | 5.70 | 5.95 | 5.62 |
| Au (225) | 3.56 | 3.67 | 3.58 | 3.65 | 3.67 | 3.28 | 3.53 | 3.31 |
| ME | -0.02 | 0.03 | -0.02 | 0.00 | 0.04 | -0.22 | -0.09 | -0.30 |
| MAE | 0.19 | 0.18 | 0.19 | 0.19 | 0.18 | 0.25 | 0.17 | 0.31 |
| MRE | -0.7 | 0.3 | -1.2 | -0.4 | 0.4 | -5.2 | -2.3 | -7.4 |
| MARE | 4.9 | 4.7 | 5.0 | 5.0 | 4.7 | 6.2 | 4.8 | 7.9 |

TABLE S9. Cohesive energy $E_{\mathrm{coh}}$ (in eV/atom) of 44 solids. All results were obtained non-self-consistently using PBE orbitals/density. The space group number is indicated in parenthesis.

| Solid | TM | TM(GEA2L) | TM(TW02L) | TM(PC) | TM(CR) | TM(GEAloc) | TM(PCopt) | TM(CRopt) |
|---|---|---|---|---|---|---|---|---|
| C (227) | 7.64 | 7.68 | 7.67 | 7.63 | 7.71 | 7.47 | 7.41 | 7.46 |
| Si (227) | 4.76 | 4.76 | 4.75 | 4.67 | 4.77 | 4.64 | 4.60 | 4.60 |
| Ge (227) | 4.03 | 4.06 | 4.05 | 4.07 | 4.06 | 4.04 | 3.94 | 3.88 |
| Sn (227) | 3.46 | 3.50 | 3.49 | 3.51 | 3.50 | 3.51 | 3.41 | 3.34 |
| SiC (216) | 6.52 | 6.49 | 6.47 | 6.42 | 6.50 | 6.33 | 6.28 | 6.31 |
| BN (216) | 6.96 | 6.87 | 6.85 | 6.80 | 6.91 | 6.82 | 6.79 | 6.79 |
| BP (216) | 5.40 | 5.38 | 5.37 | 5.32 | 5.41 | 5.31 | 5.25 | 5.26 |
| AlN (216) | 5.89 | 5.74 | 5.72 | 5.69 | 5.76 | 5.75 | 5.72 | 5.70 |
| AlP (216) | 4.31 | 4.28 | 4.27 | 4.25 | 4.29 | 4.25 | 4.20 | 4.19 |
| AlAs (216) | 3.94 | 3.93 | 3.91 | 3.90 | 3.93 | 3.91 | 3.84 | 3.81 |
| GaN (216) | 4.67 | 4.59 | 4.57 | 4.57 | 4.60 | 4.61 | 4.54 | 4.49 |
| GaP (216) | 3.77 | 3.77 | 3.76 | 3.77 | 3.78 | 3.75 | 3.67 | 3.63 |
| GaAs (216) | 3.47 | 3.48 | 3.46 | 3.48 | 3.48 | 3.47 | 3.37 | 3.31 |
| InP (216) | 3.42 | 3.44 | 3.42 | 3.44 | 3.44 | 3.43 | 3.36 | 3.30 |
| InAs (216) | 3.19 | 3.21 | 3.19 | 3.21 | 3.21 | 3.21 | 3.12 | 3.05 |
| InSb (216) | 2.91 | 2.95 | 2.93 | 2.95 | 2.94 | 2.95 | 2.86 | 2.78 |
| LiH (225) | 2.45 | 2.41 | 2.40 | 2.40 | 2.41 | 2.45 | 2.43 | 2.45 |
| LiF (225) | 4.36 | 4.33 | 4.31 | 4.31 | 4.33 | 4.24 | 4.22 | 4.23 |
| LiCl (225) | 3.47 | 3.44 | 3.43 | 3.39 | 3.44 | 3.40 | 3.38 | 3.38 |
| NaF (225) | 3.88 | 3.85 | 3.84 | 3.84 | 3.86 | 3.77 | 3.74 | 3.74 |
| NaCl (225) | 3.23 | 3.19 | 3.18 | 3.15 | 3.19 | 3.16 | 3.14 | 3.13 |
| MgO (225) | 5.20 | 5.07 | 5.05 | 4.93 | 5.08 | 5.02 | 5.02 | 5.02 |
| Li (229) | 1.68 | 1.66 | 1.65 | 1.65 | 1.66 | 1.67 | 1.66 | 1.68 |
| Na (229) | 1.20 | 1.20 | 1.19 | 1.20 | 1.20 | 1.22 | 1.20 | 1.19 |
| Al (225) | 3.86 | 3.84 | 3.83 | 3.78 | 3.85 | 3.81 | 3.76 | 3.79 |
| K (229) | 1.00 | 1.01 | 1.00 | 1.01 | 1.01 | 1.04 | 1.01 | 1.01 |
| Ca (225) | 2.29 | 2.26 | 2.25 | 2.26 | 2.26 | 2.28 | 2.24 | 2.25 |
| Rb (229) | 0.92 | 0.93 | 0.92 | 0.94 | 0.93 | 0.97 | 0.93 | 0.93 |
| Sr (225) | 2.05 | 2.02 | 2.01 | 2.03 | 2.02 | 2.08 | 2.02 | 2.03 |
| Cs (229) | 0.85 | 0.87 | 0.86 | 0.88 | 0.87 | 0.91 | 0.87 | 0.87 |
| Ba (229) | 2.34 | 2.31 | 2.30 | 2.31 | 2.31 | 2.37 | 2.31 | 2.31 |
| V (229) | 5.86 | 6.05 | 6.03 | 6.06 | 6.05 | 6.04 | 5.95 | 5.87 |
| Ni (225) | 5.45 | 5.49 | 5.48 | 5.49 | 5.49 | 5.49 | 5.34 | 5.27 |
| Cu (225) | 4.45 | 4.30 | 4.28 | 4.31 | 4.30 | 4.45 | 4.31 | 4.22 |
| Nb (229) | 7.56 | 7.70 | 7.68 | 7.71 | 7.70 | 7.70 | 7.57 | 7.47 |
| Mo (229) | 6.96 | 7.11 | 7.09 | 7.12 | 7.11 | 7.15 | 7.03 | 6.87 |
| Rh (225) | 6.41 | 6.56 | 6.55 | 6.56 | 6.56 | 6.50 | 6.30 | 6.23 |
| Pd (225) | 4.58 | 4.52 | 4.50 | 4.53 | 4.52 | 4.63 | 4.47 | 4.35 |
| Ag (225) | 3.28 | 3.20 | 3.18 | 3.21 | 3.20 | 3.31 | 3.16 | 3.07 |
| Ta (229) | 9.12 | 9.13 | 9.13 | 9.13 | 9.14 | 9.13 | 8.96 | 8.93 |
| W (229) | 9.30 | 9.32 | 9.29 | 9.33 | 9.32 | 9.38 | 9.20 | 9.07 |
| Ir (225) | 8.27 | 8.31 | 8.30 | 8.31 | 8.31 | 8.29 | 8.06 | 7.98 |
| Pt (225) | 6.53 | 6.50 | 6.49 | 6.51 | 6.50 | 6.56 | 6.36 | 6.26 |
| Au (225) | 3.91 | 3.83 | 3.81 | 3.84 | 3.83 | 3.93 | 3.75 | 3.65 |
| ME | 0.24 | 0.24 | 0.22 | 0.22 | 0.24 | 0.23 | 0.15 | 0.11 |
| MAE | 0.27 | 0.28 | 0.27 | 0.28 | 0.28 | 0.30 | 0.24 | 0.22 |
| MRE | 6.4 | 6.1 | 5.7 | 5.9 | 6.2 | 6.6 | 4.4 | 3.5 |
| MARE | 7.0 | 7.2 | 7.0 | 7.4 | 7.3 | 8.1 | 6.5 | 6.0 |

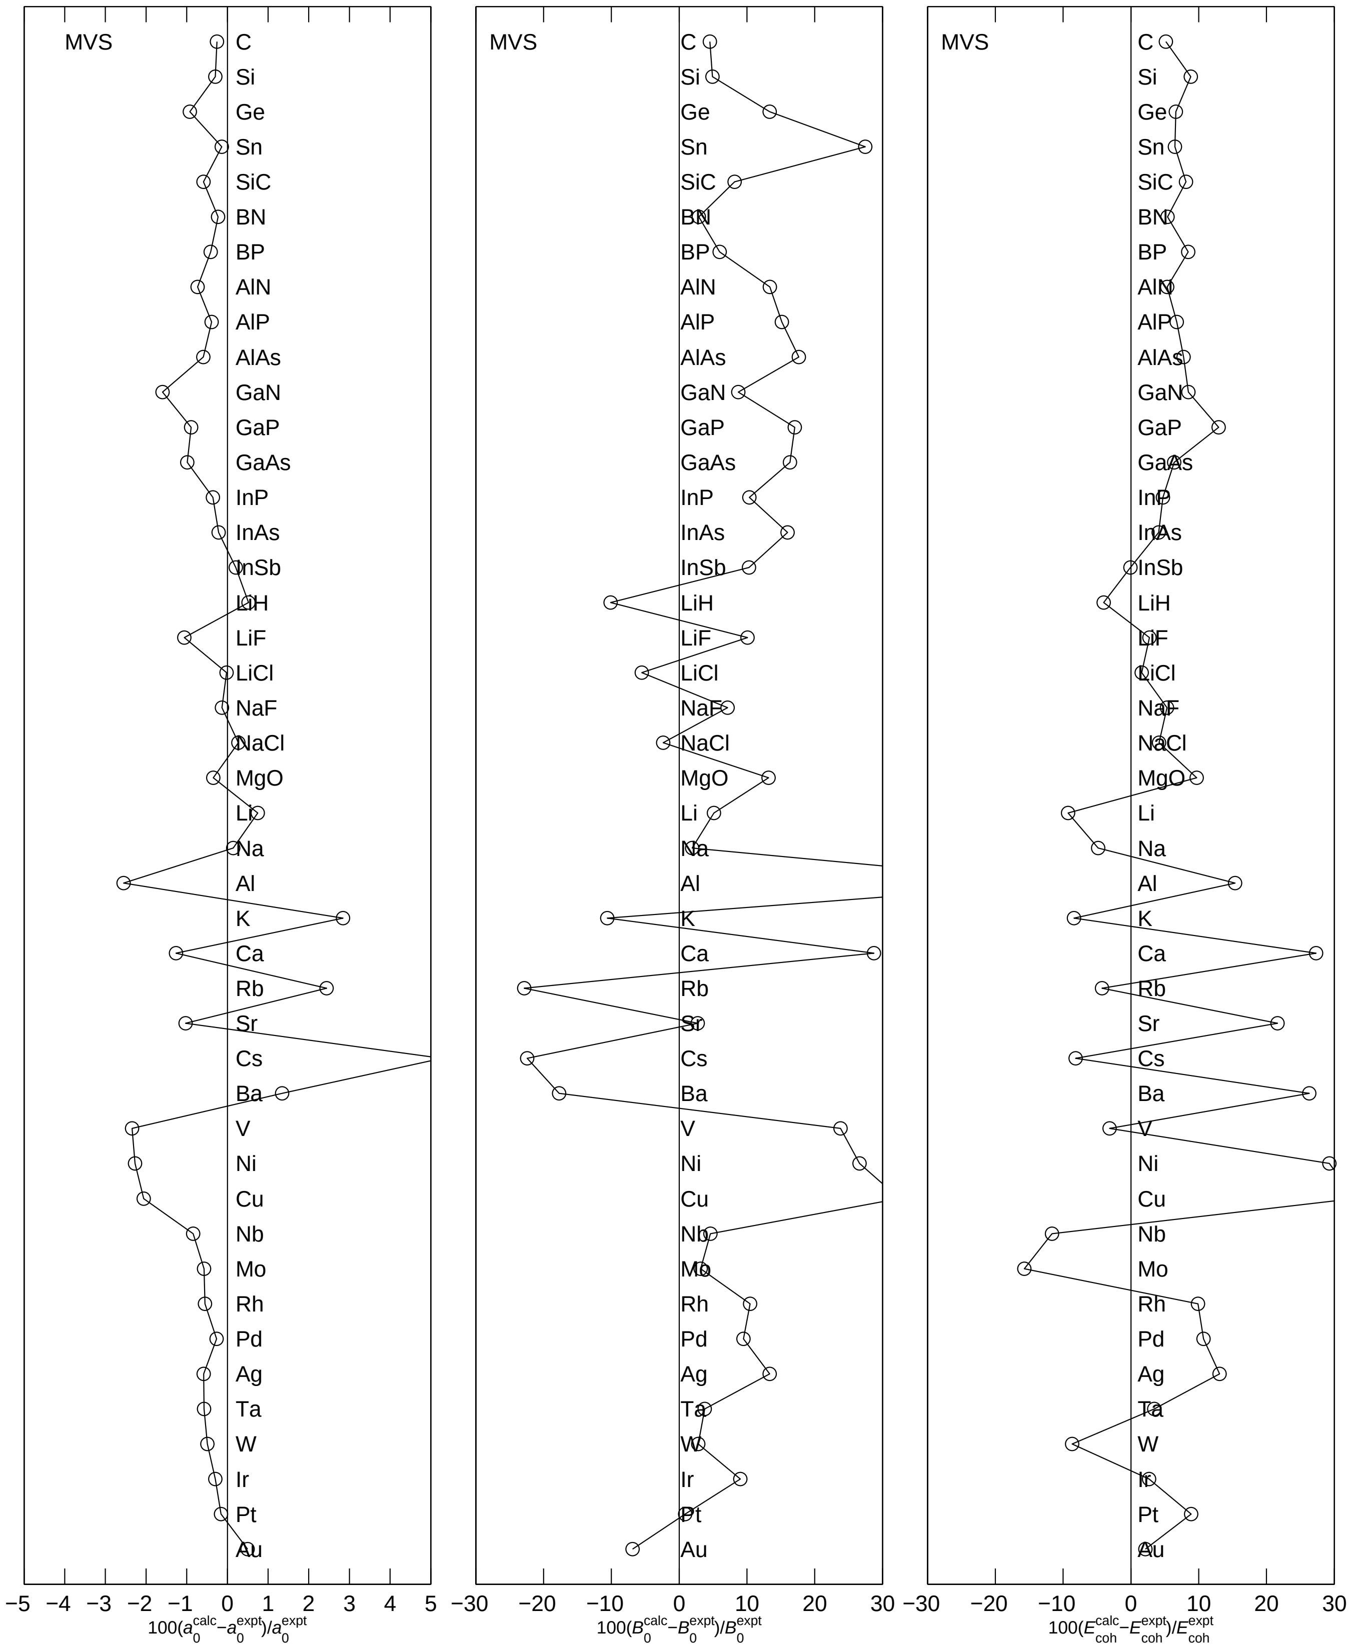


FIG. S1. Relative error (in %) in the calculated lattice constants $a_0$ (left), bulk modulus $B_0$ (middle), and cohesive energy $E_{\mathrm{coh}}$ (right) with respect to the experimental values.

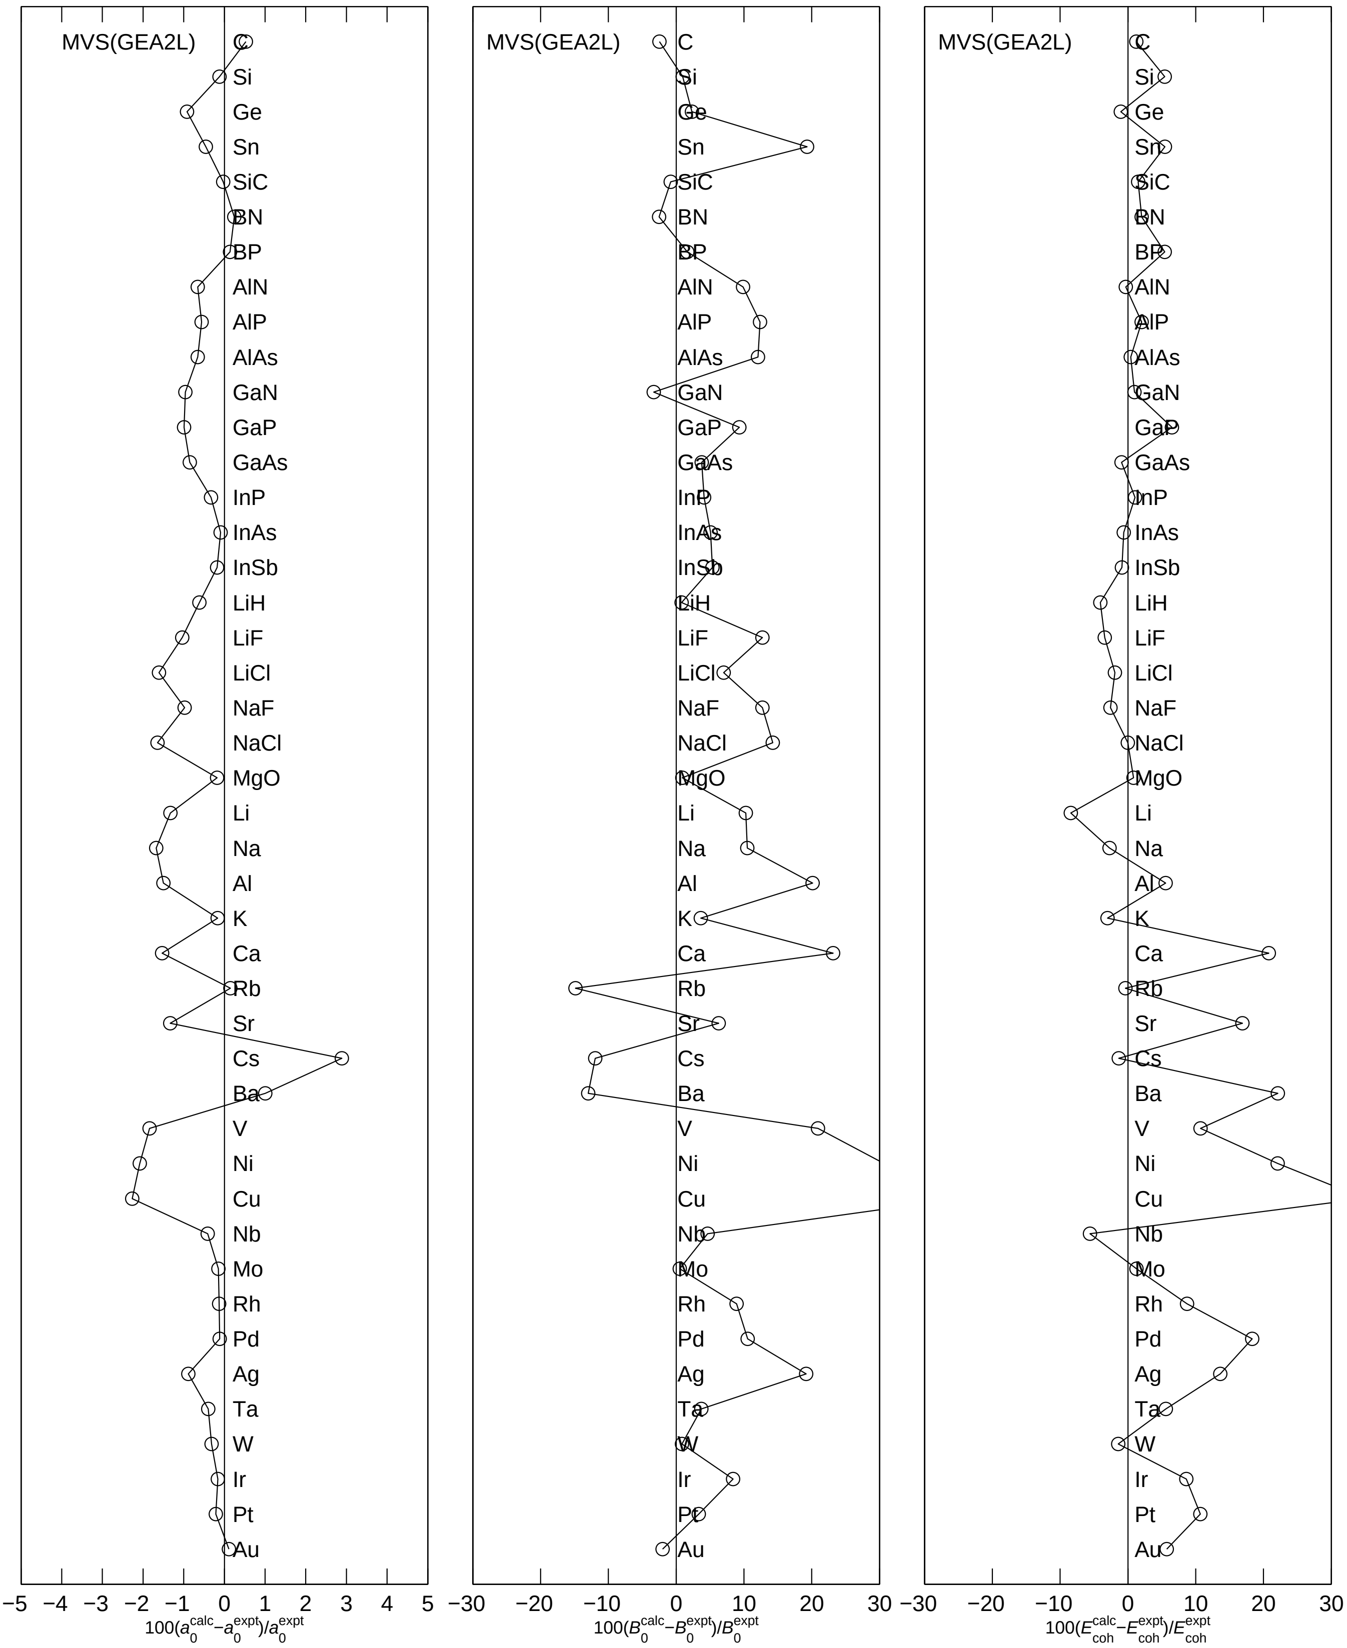


FIG. S2. Relative error (in %) in the calculated lattice constants $a_0$ (left), bulk modulus $B_0$ (middle), and cohesive energy $E_{\mathrm{coh}}$ (right) with respect to the experimental values.

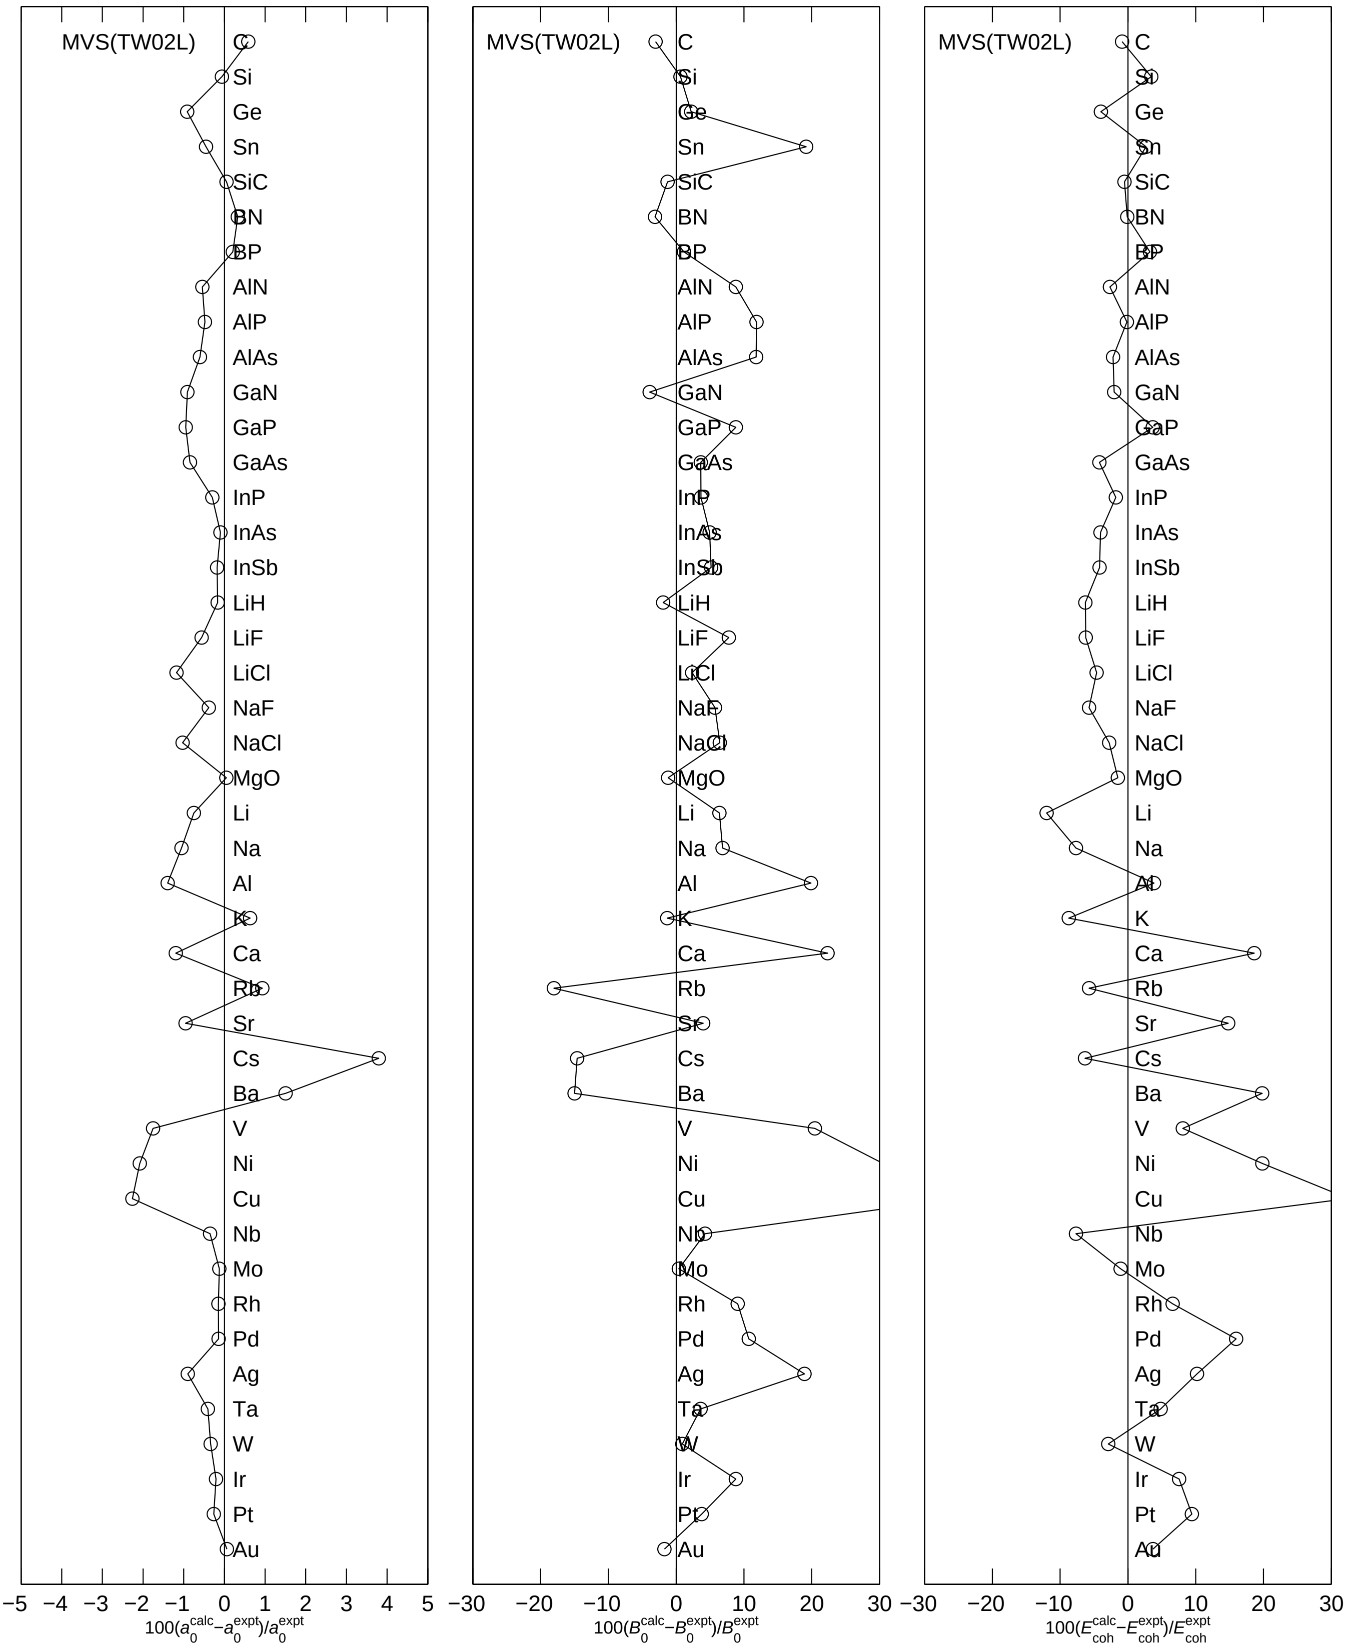


FIG. S3. Relative error (in %) in the calculated lattice constants $a_0$ (left), bulk modulus $B_0$ (middle), and cohesive energy $E_{\rm coh}$ (right) with respect to the experimental values.

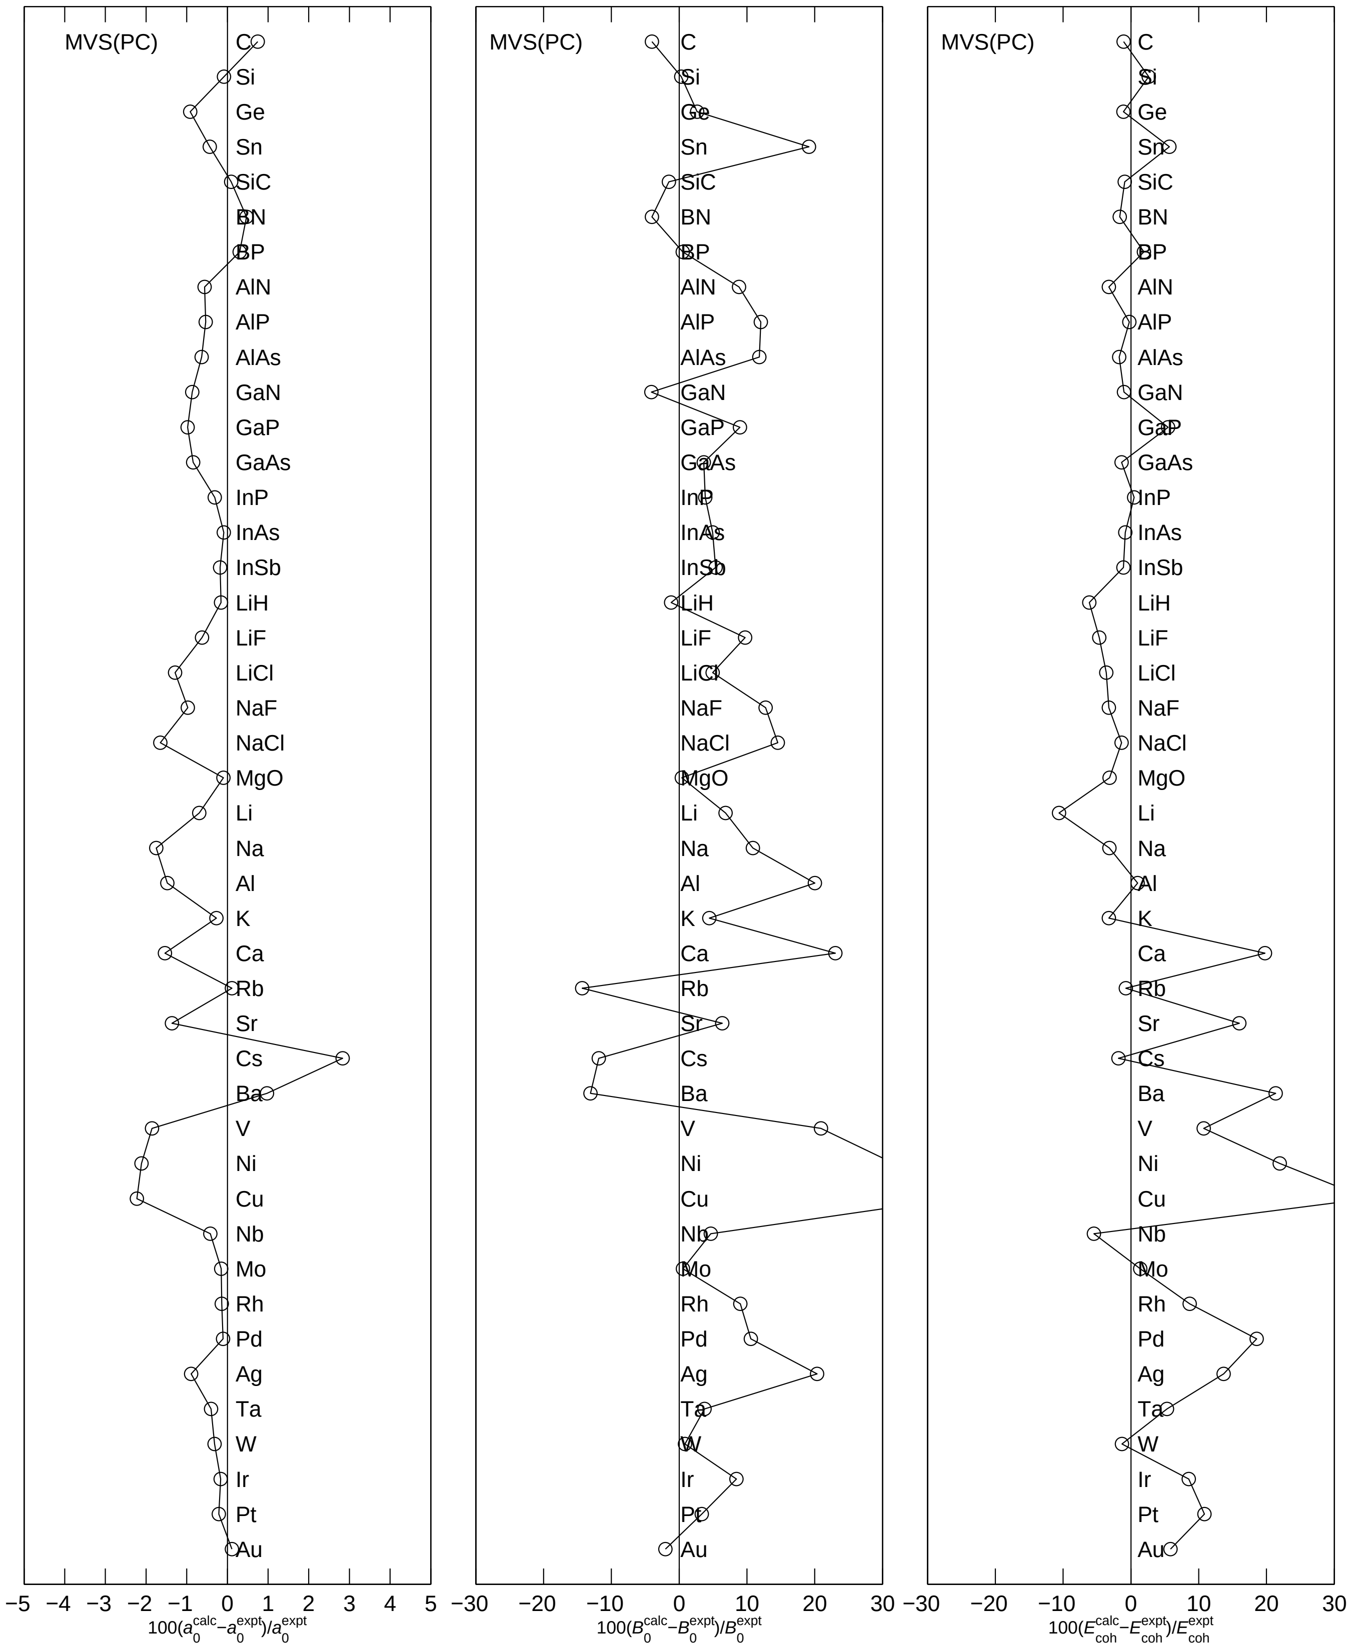


FIG. S4. Relative error (in %) in the calculated lattice constants $a_0$ (left), bulk modulus $B_0$ (middle), and cohesive energy $E_{\rm coh}$ (right) with respect to the experimental values.

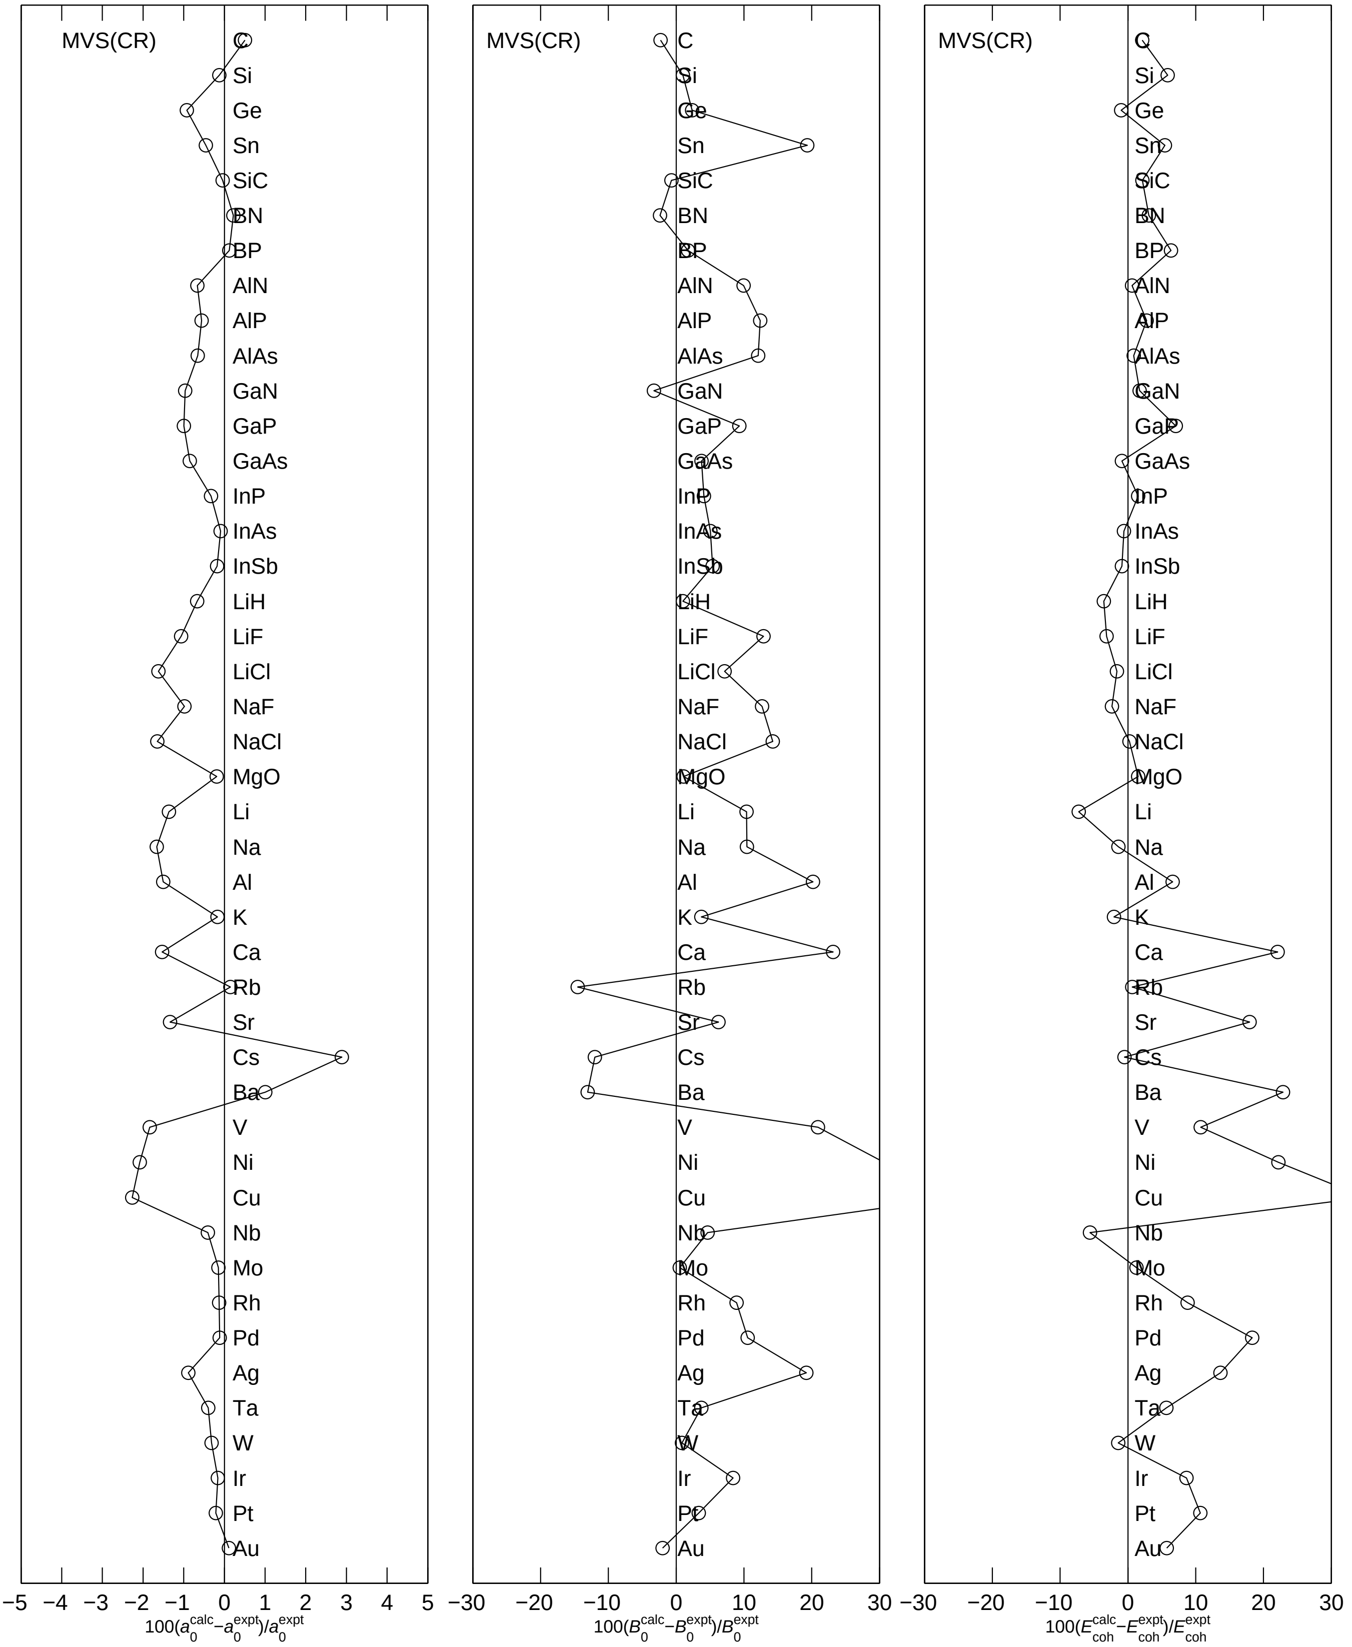


FIG. S5. Relative error (in %) in the calculated lattice constants $a_0$ (left), bulk modulus $B_0$ (middle), and cohesive energy $E_{\rm coh}$ (right) with respect to the experimental values.

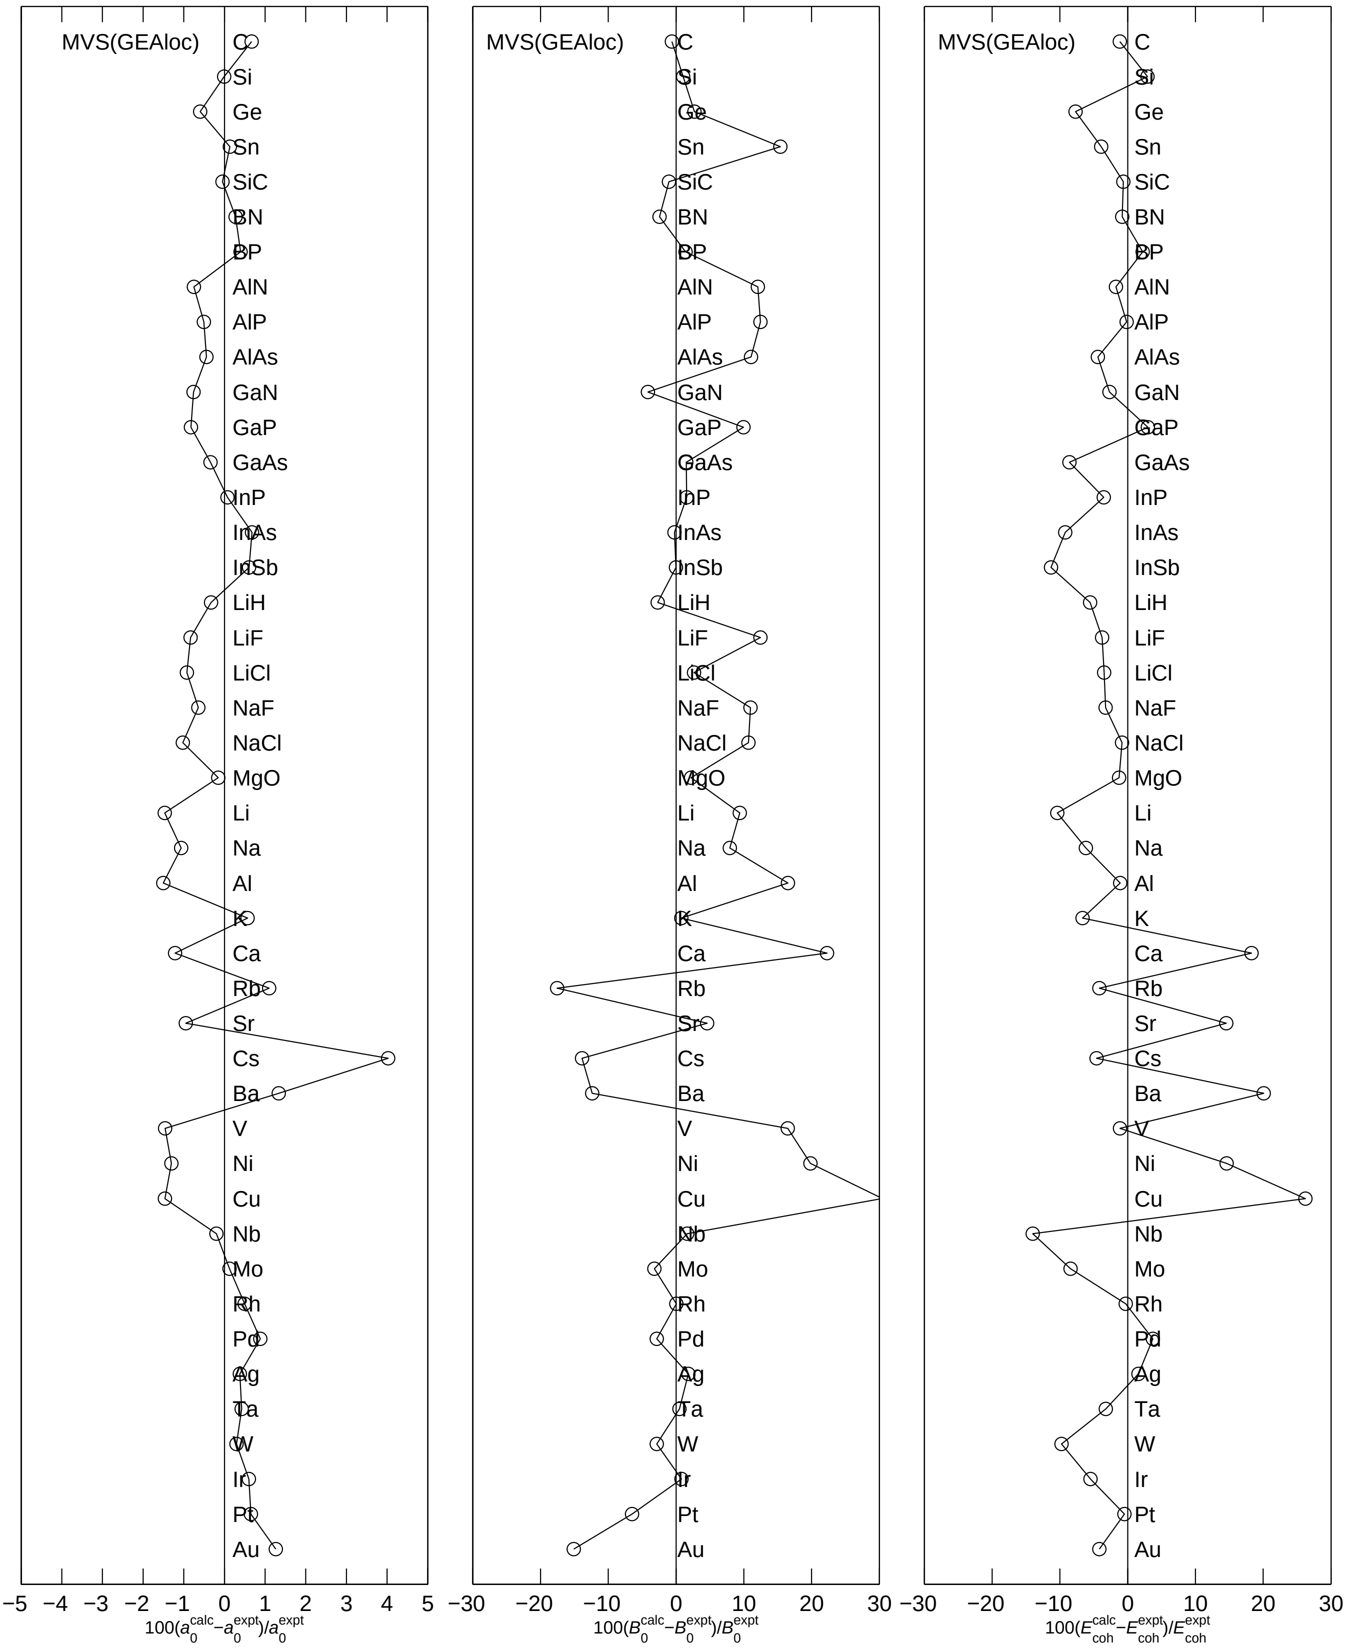


FIG. S6. Relative error (in %) in the calculated lattice constants $a_0$ (left), bulk modulus $B_0$ (middle), and cohesive energy $E_{\rm coh}$ (right) with respect to the experimental values.

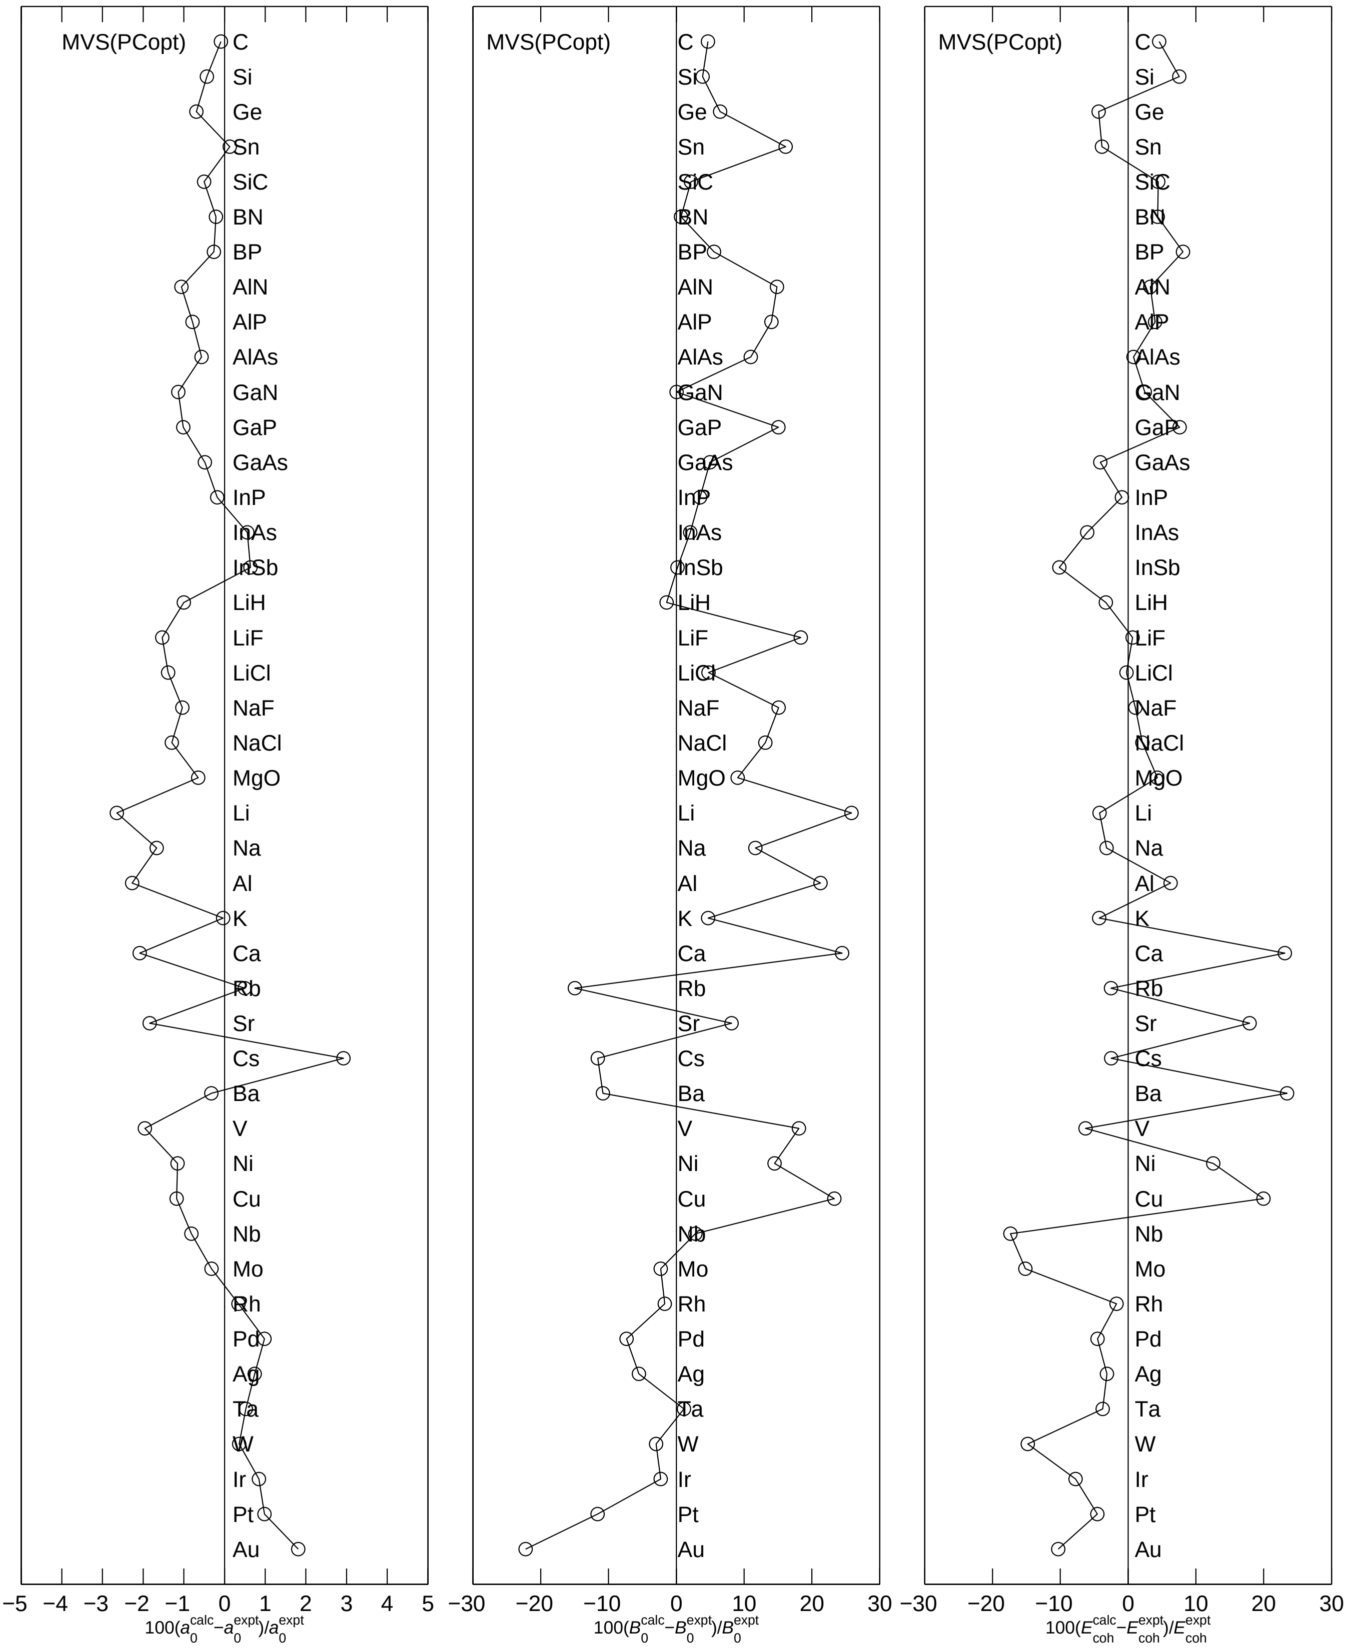


FIG. S7. Relative error (in %) in the calculated lattice constants $a_0$ (left), bulk modulus $B_0$ (middle), and cohesive energy $E_{\mathrm{coh}}$ (right) with respect to the experimental values.

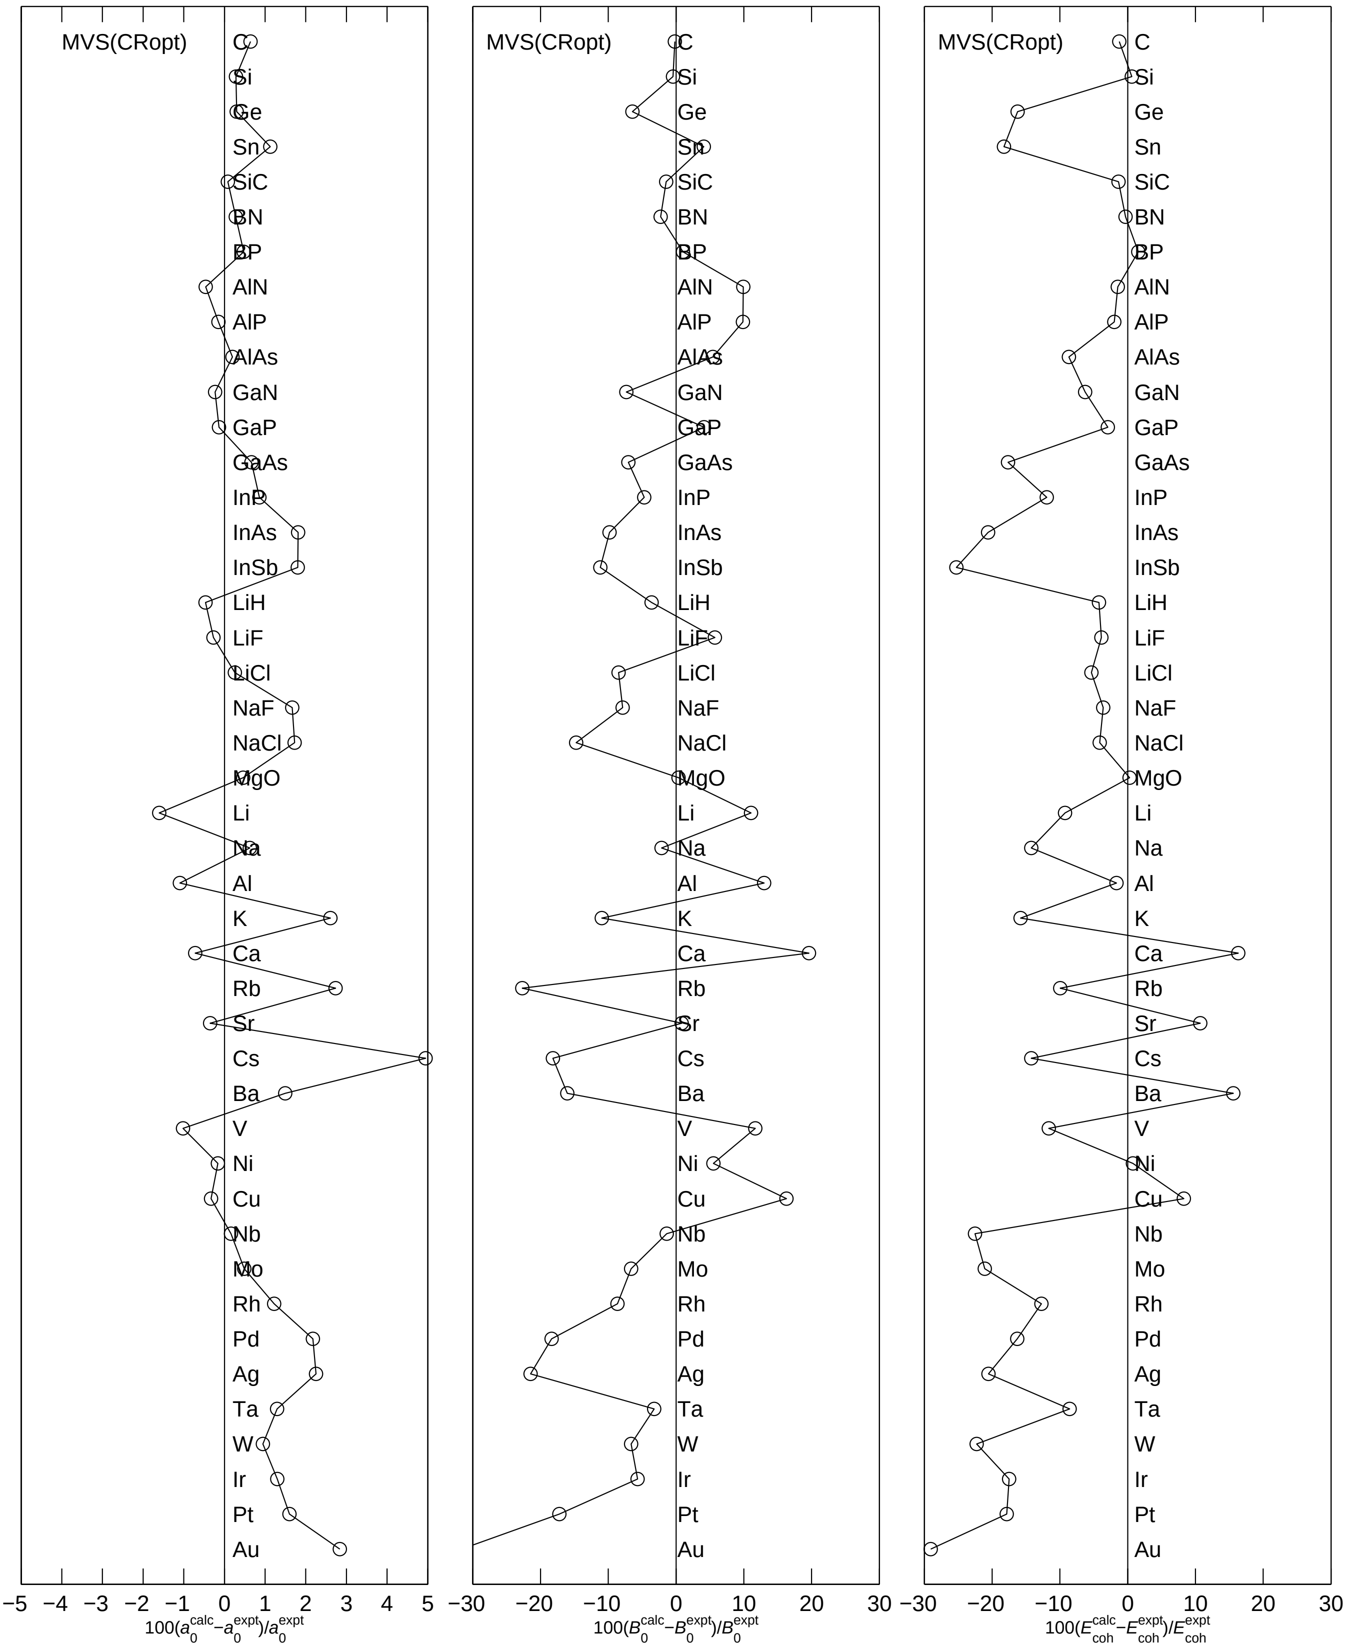


FIG. S8. Relative error (in %) in the calculated lattice constants $a_0$ (left), bulk modulus $B_0$ (middle), and cohesive energy $E_{\mathrm{coh}}$ (right) with respect to the experimental values.

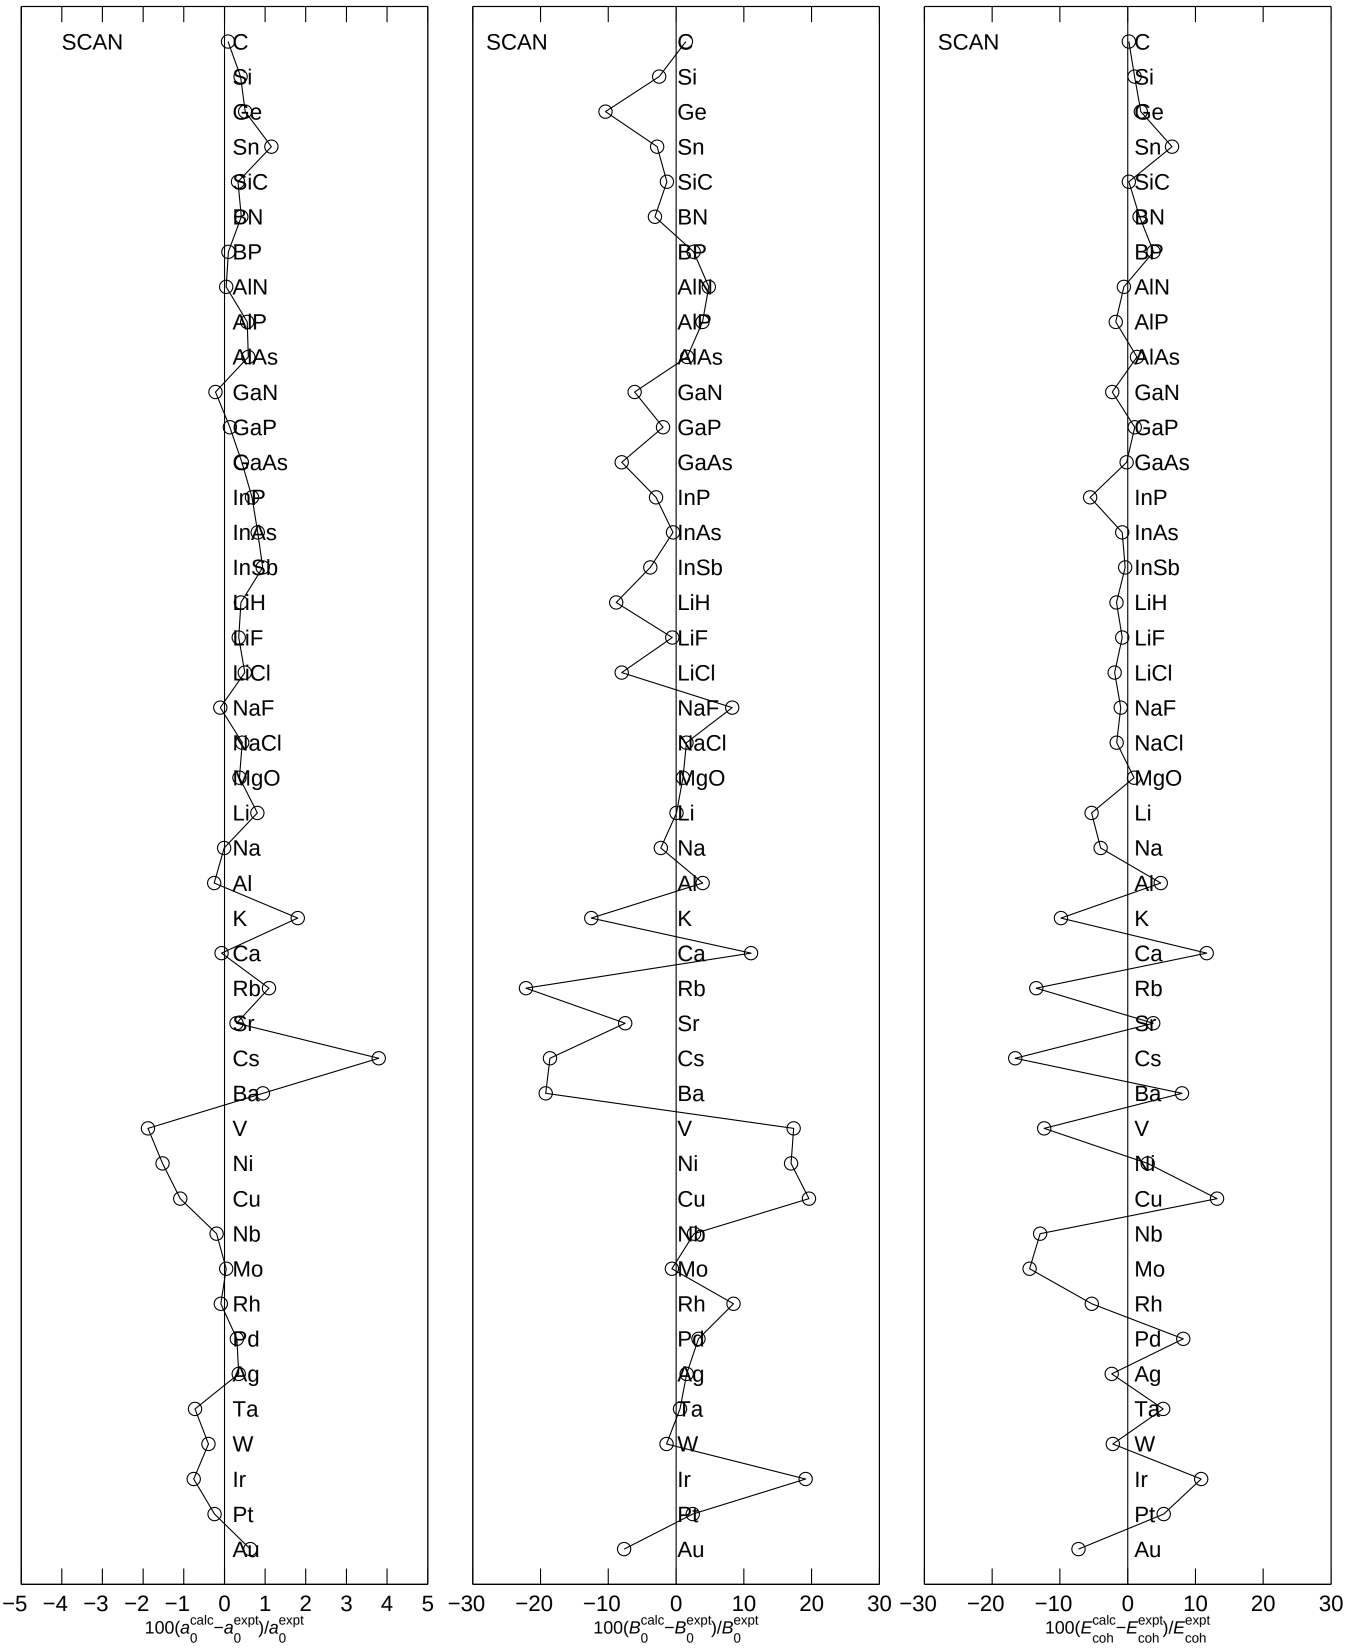


FIG. S9. Relative error (in %) in the calculated lattice constants $a_0$ (left), bulk modulus $B_0$ (middle), and cohesive energy $E_{\mathrm{coh}}$ (right) with respect to the experimental values.

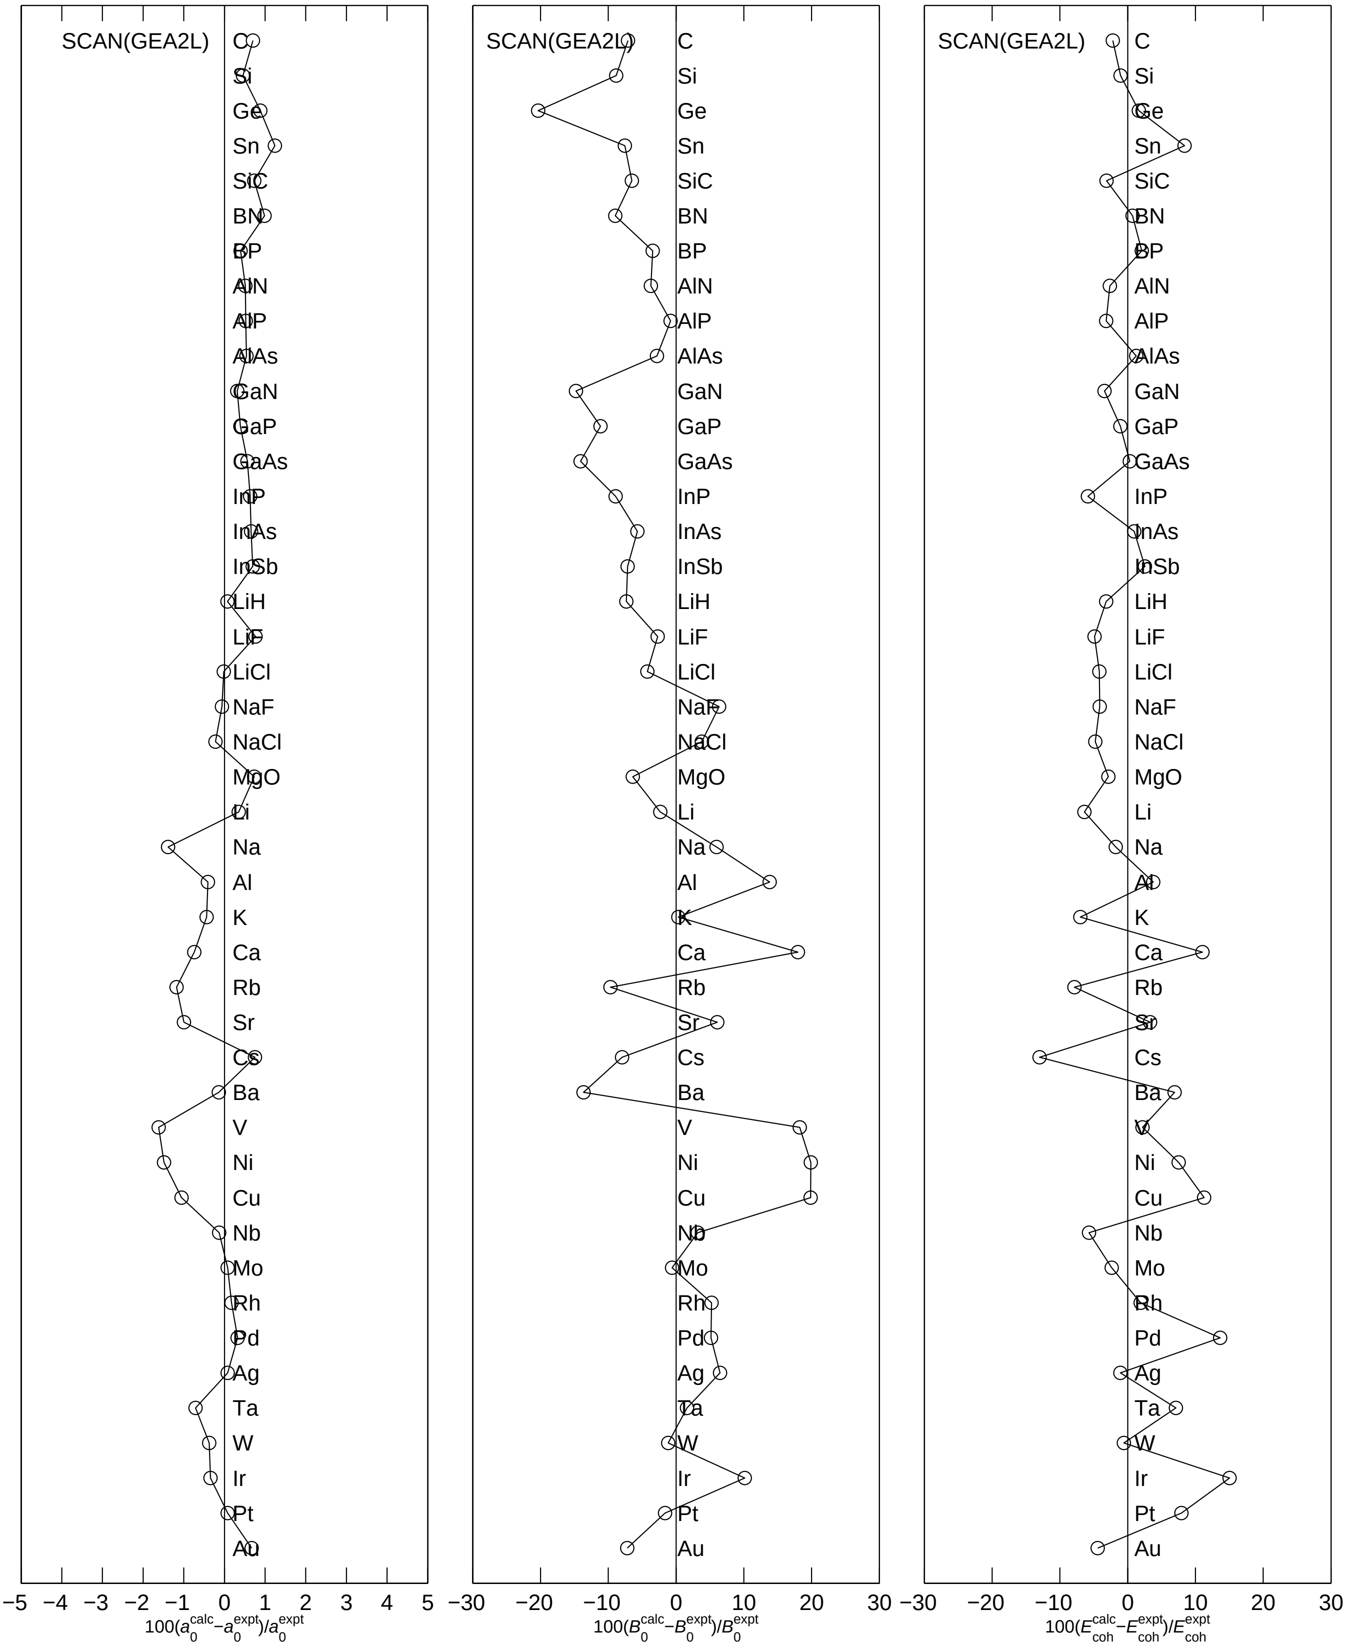


FIG. S10. Relative error (in %) in the calculated lattice constants $a_0$ (left), bulk modulus $B_0$ (middle), and cohesive energy $E_{\mathrm{coh}}$ (right) with respect to the experimental values.

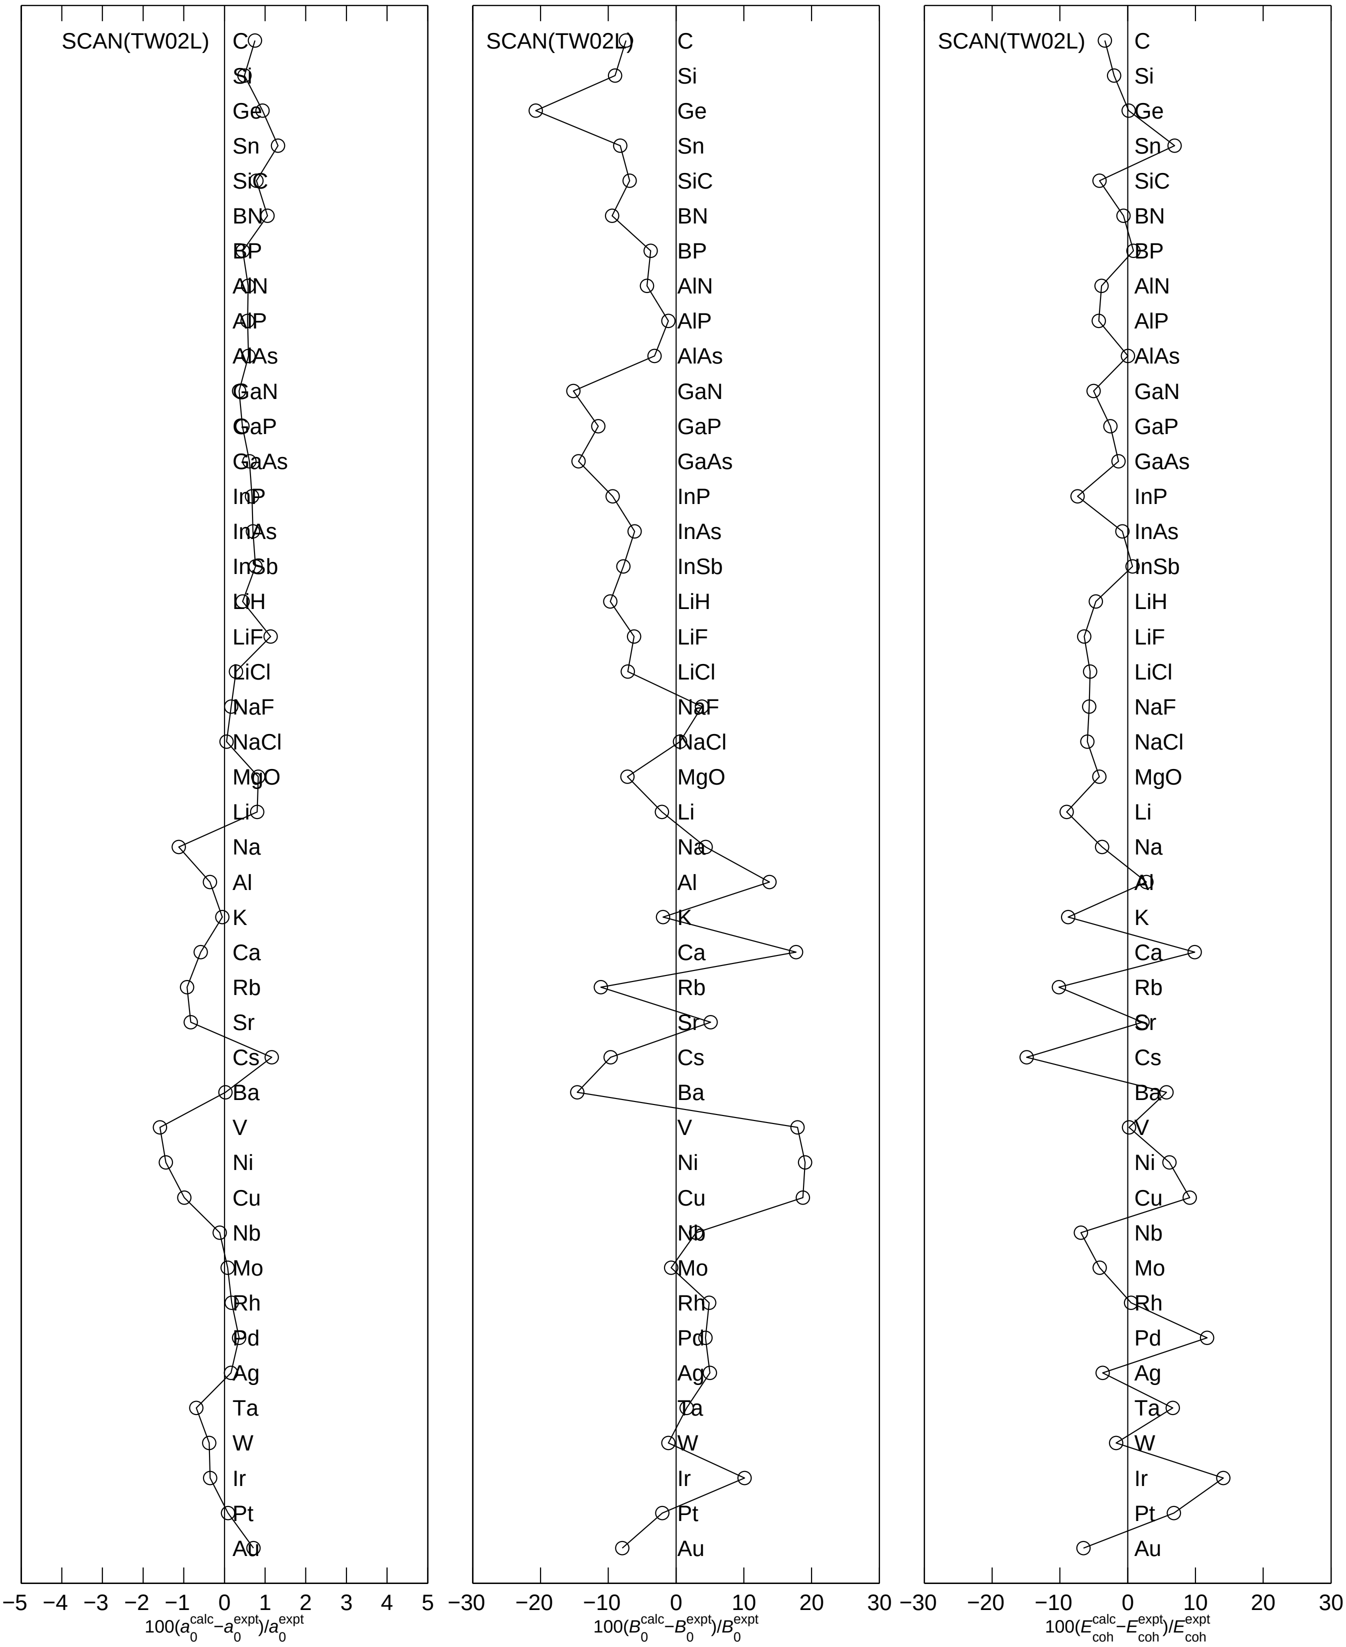


FIG. S11. Relative error (in %) in the calculated lattice constants $a_0$ (left), bulk modulus $B_0$ (middle), and cohesive energy $E_{\rm coh}$ (right) with respect to the experimental values.

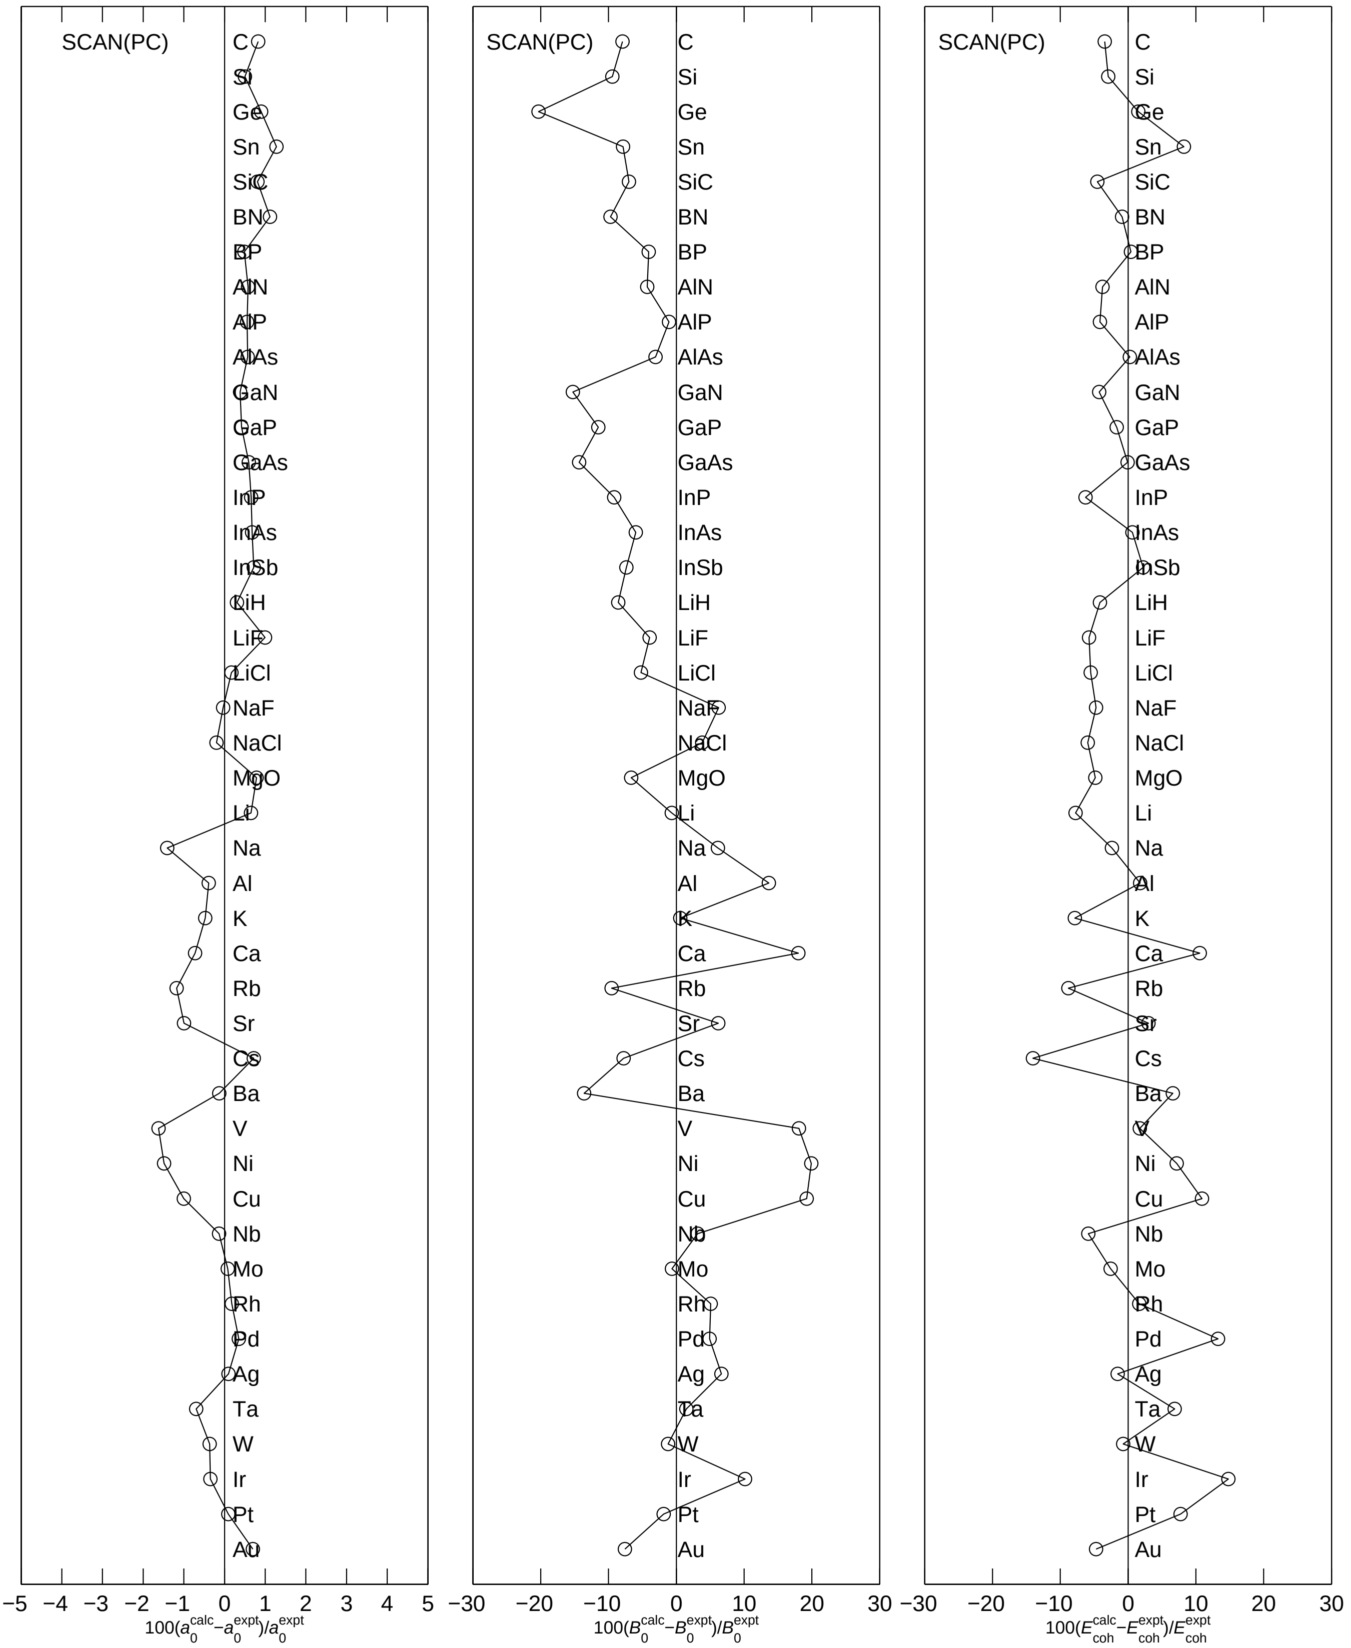


FIG. S12. Relative error (in %) in the calculated lattice constants $a_0$ (left), bulk modulus $B_0$ (middle), and cohesive energy $E_{\mathrm{coh}}$ (right) with respect to the experimental values.

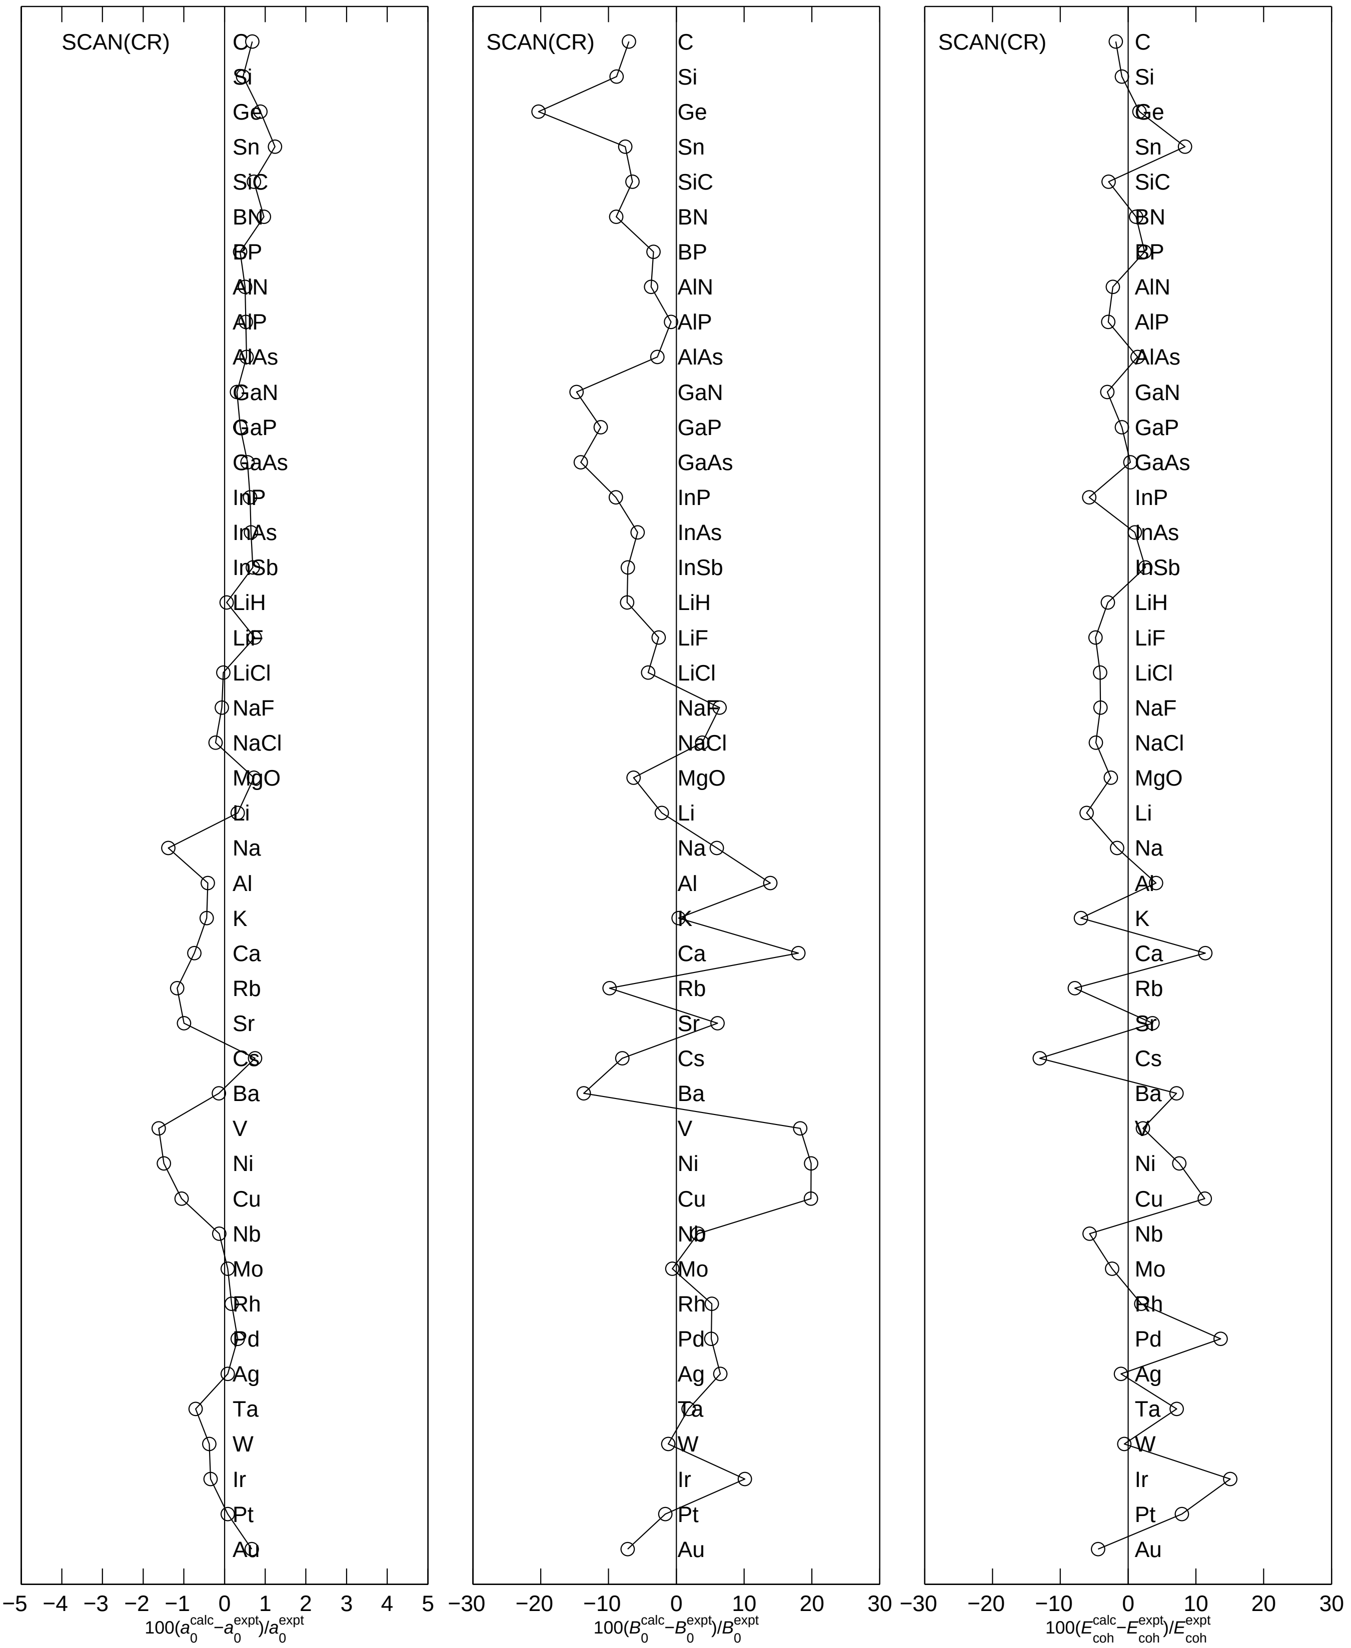


FIG. S13. Relative error (in %) in the calculated lattice constants $a_0$ (left), bulk modulus $B_0$ (middle), and cohesive energy $E_{\mathrm{coh}}$ (right) with respect to the experimental values.

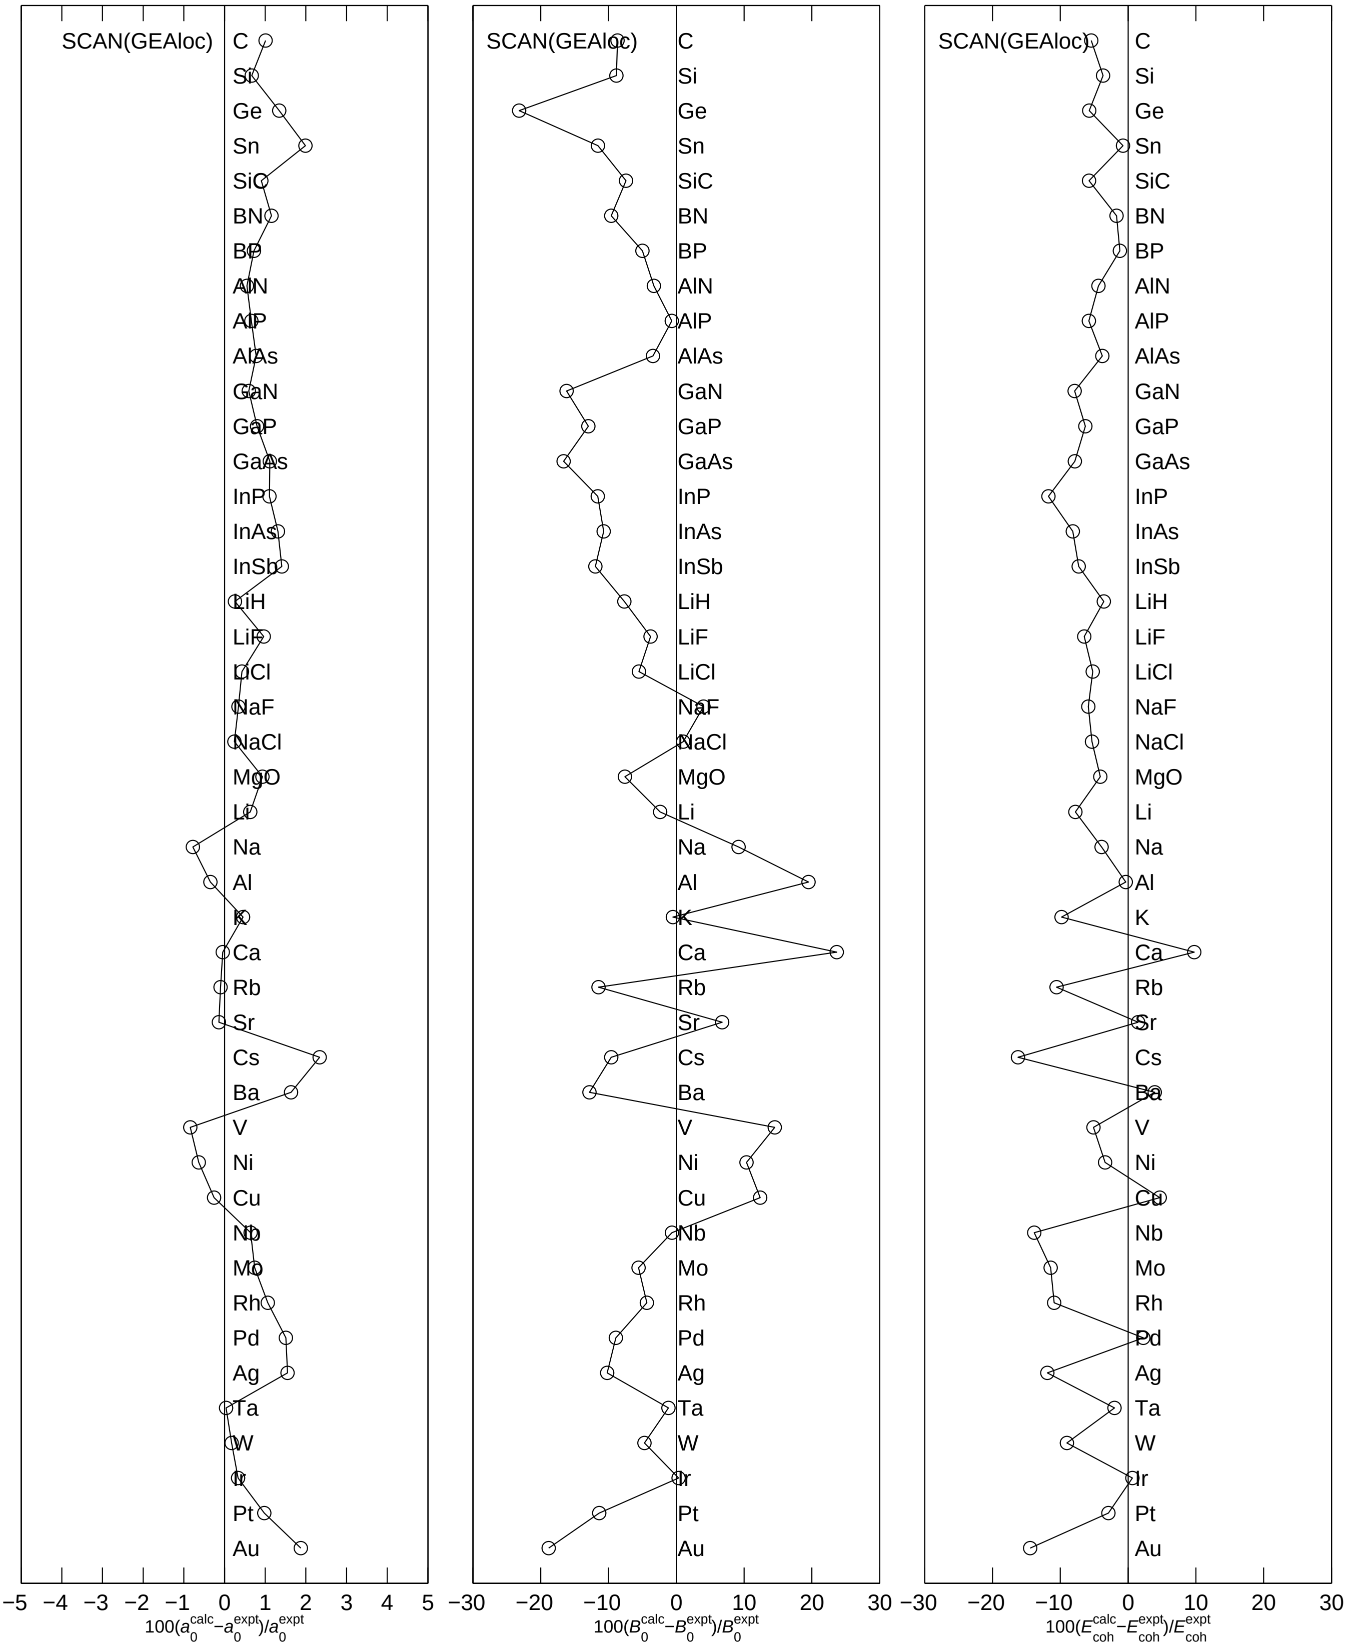


FIG. S14. Relative error (in %) in the calculated lattice constants $a_0$ (left), bulk modulus $B_0$ (middle), and cohesive energy $E_{\rm coh}$ (right) with respect to the experimental values.

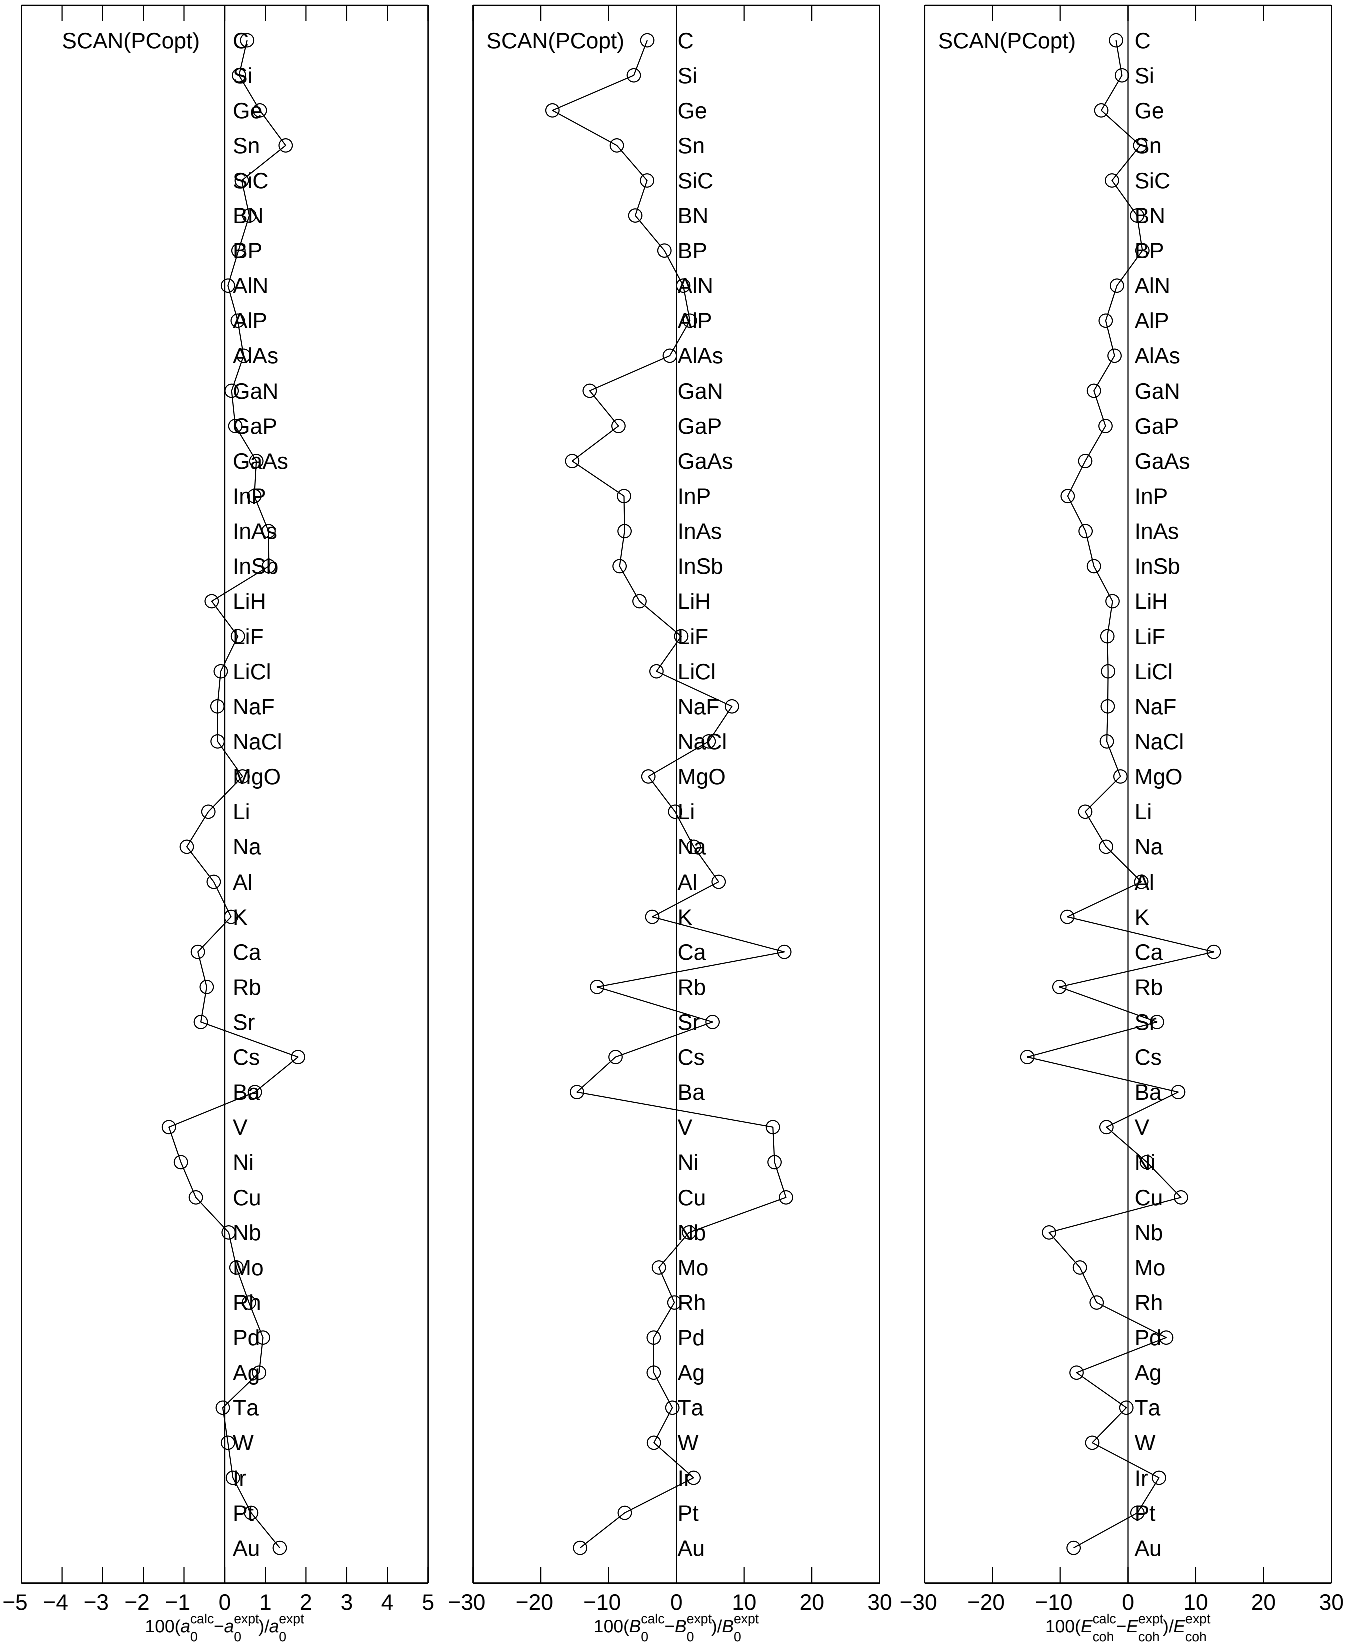


FIG. S15. Relative error (in %) in the calculated lattice constants $a_0$ (left), bulk modulus $B_0$ (middle), and cohesive energy $E_{\rm coh}$ (right) with respect to the experimental values.

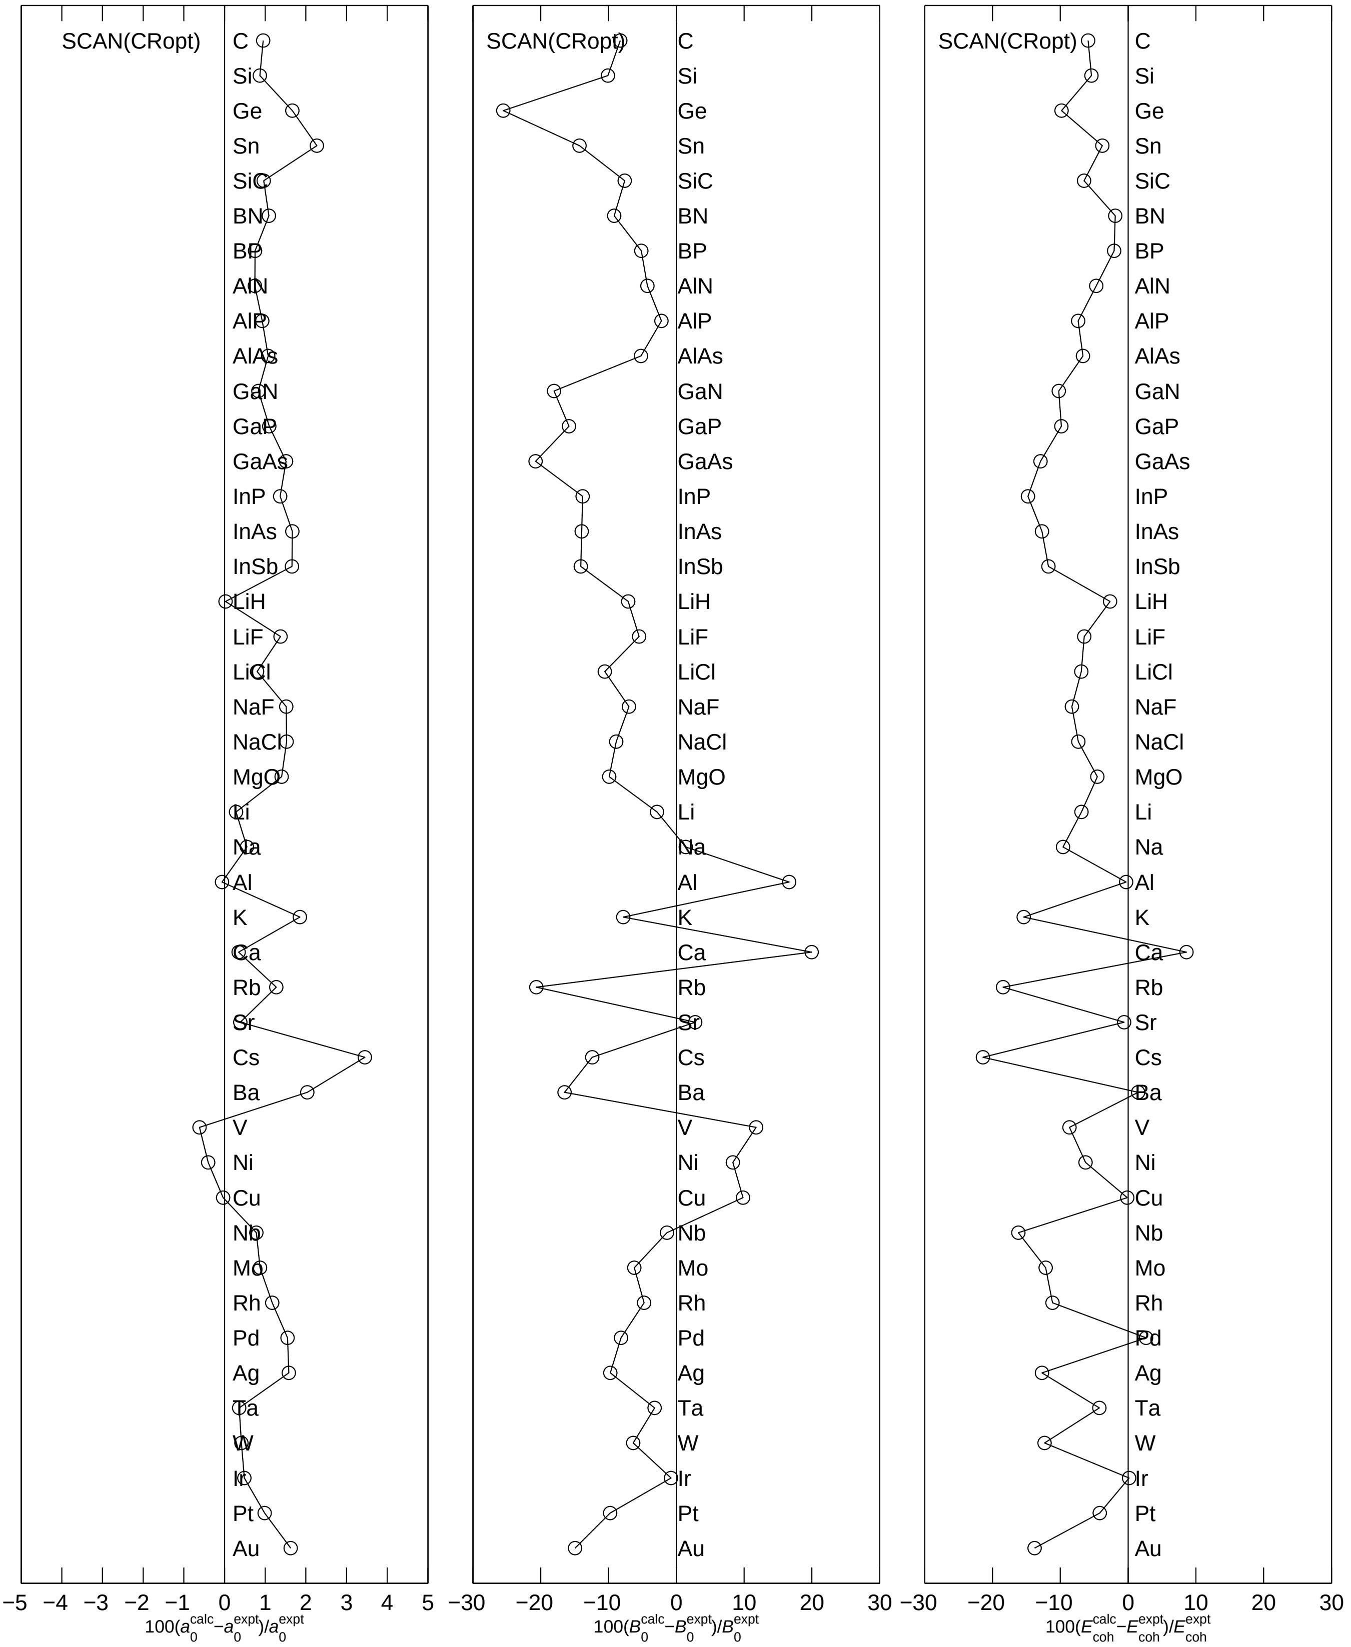


FIG. S16. Relative error (in %) in the calculated lattice constants $a_0$ (left), bulk modulus $B_0$ (middle), and cohesive energy $E_{\rm coh}$ (right) with respect to the experimental values.

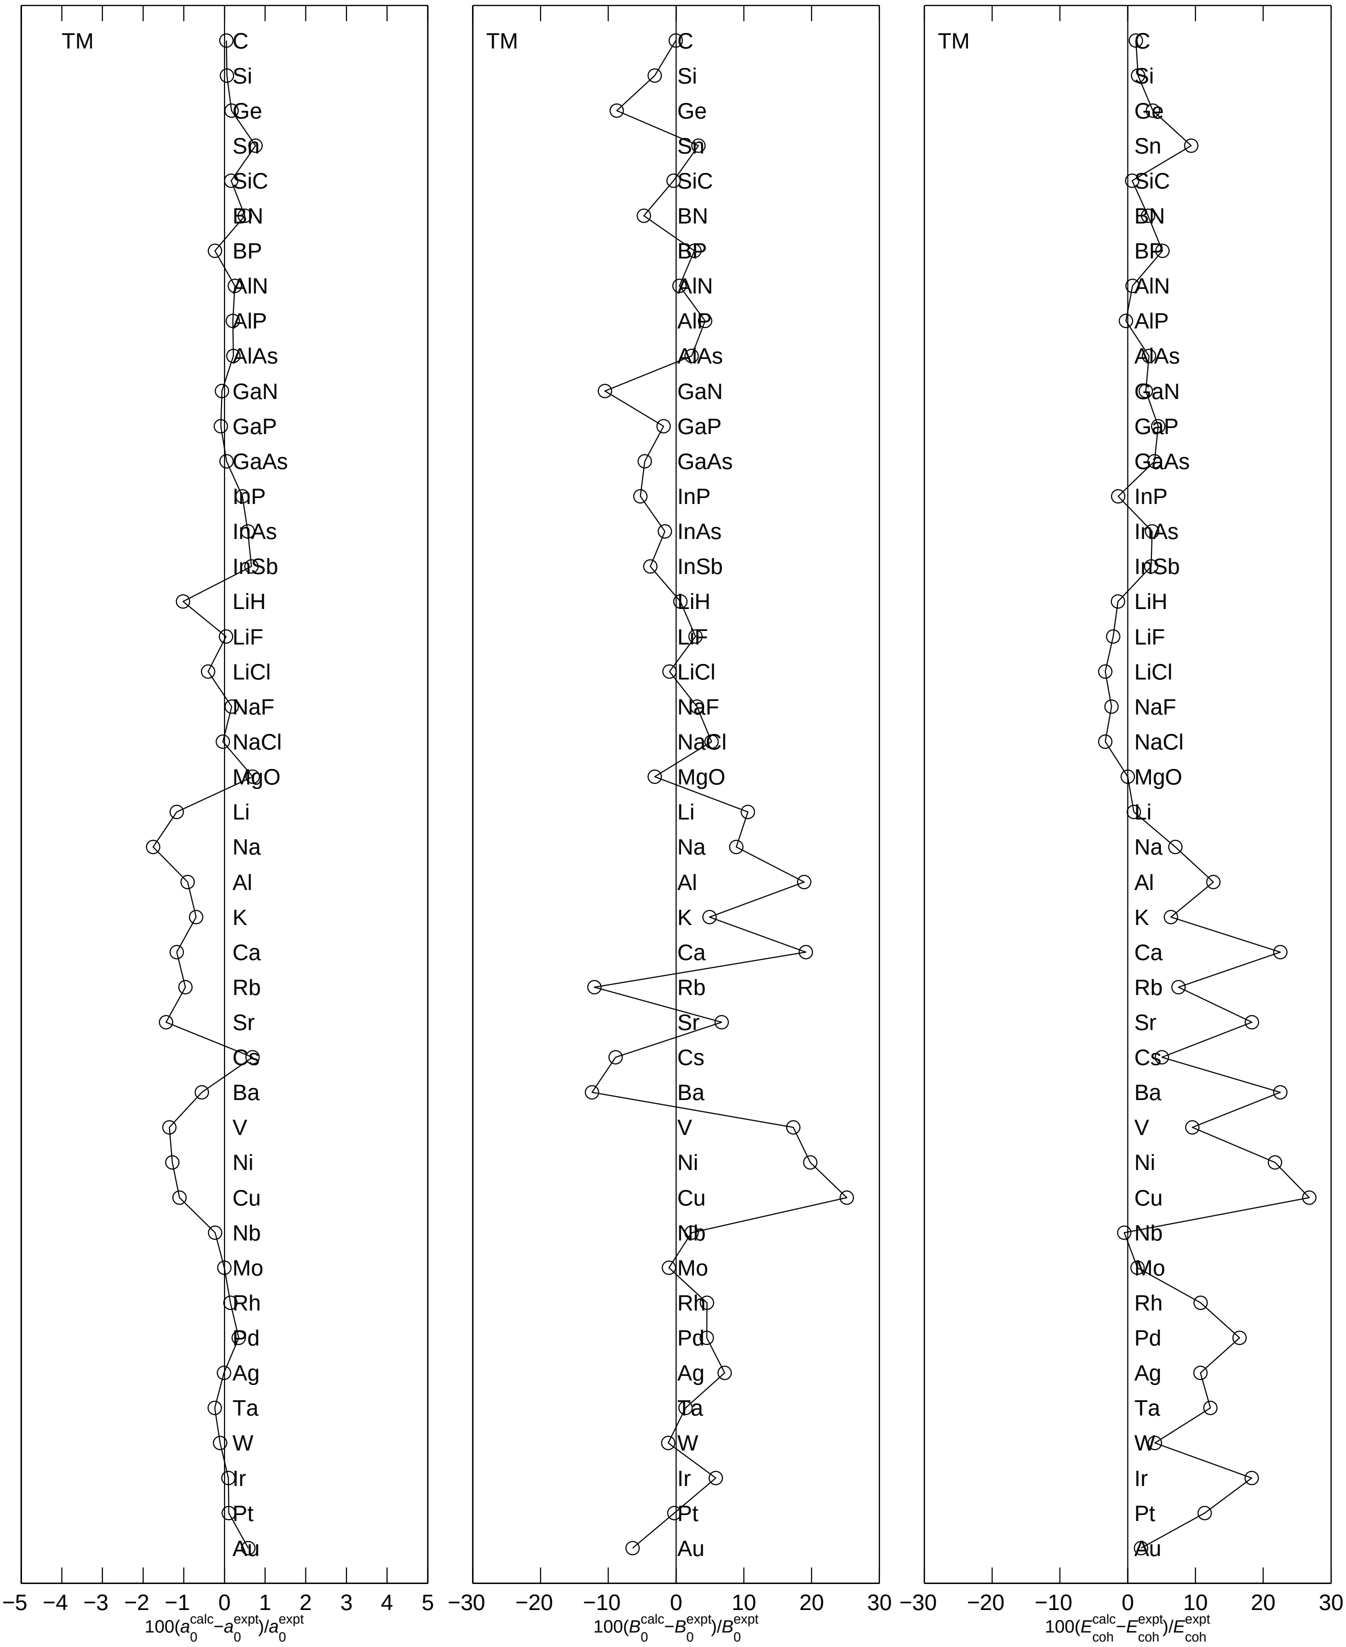


FIG. S17. Relative error (in %) in the calculated lattice constants $a_0$ (left), bulk modulus $B_0$ (middle), and cohesive energy $E_{\rm coh}$ (right) with respect to the experimental values.

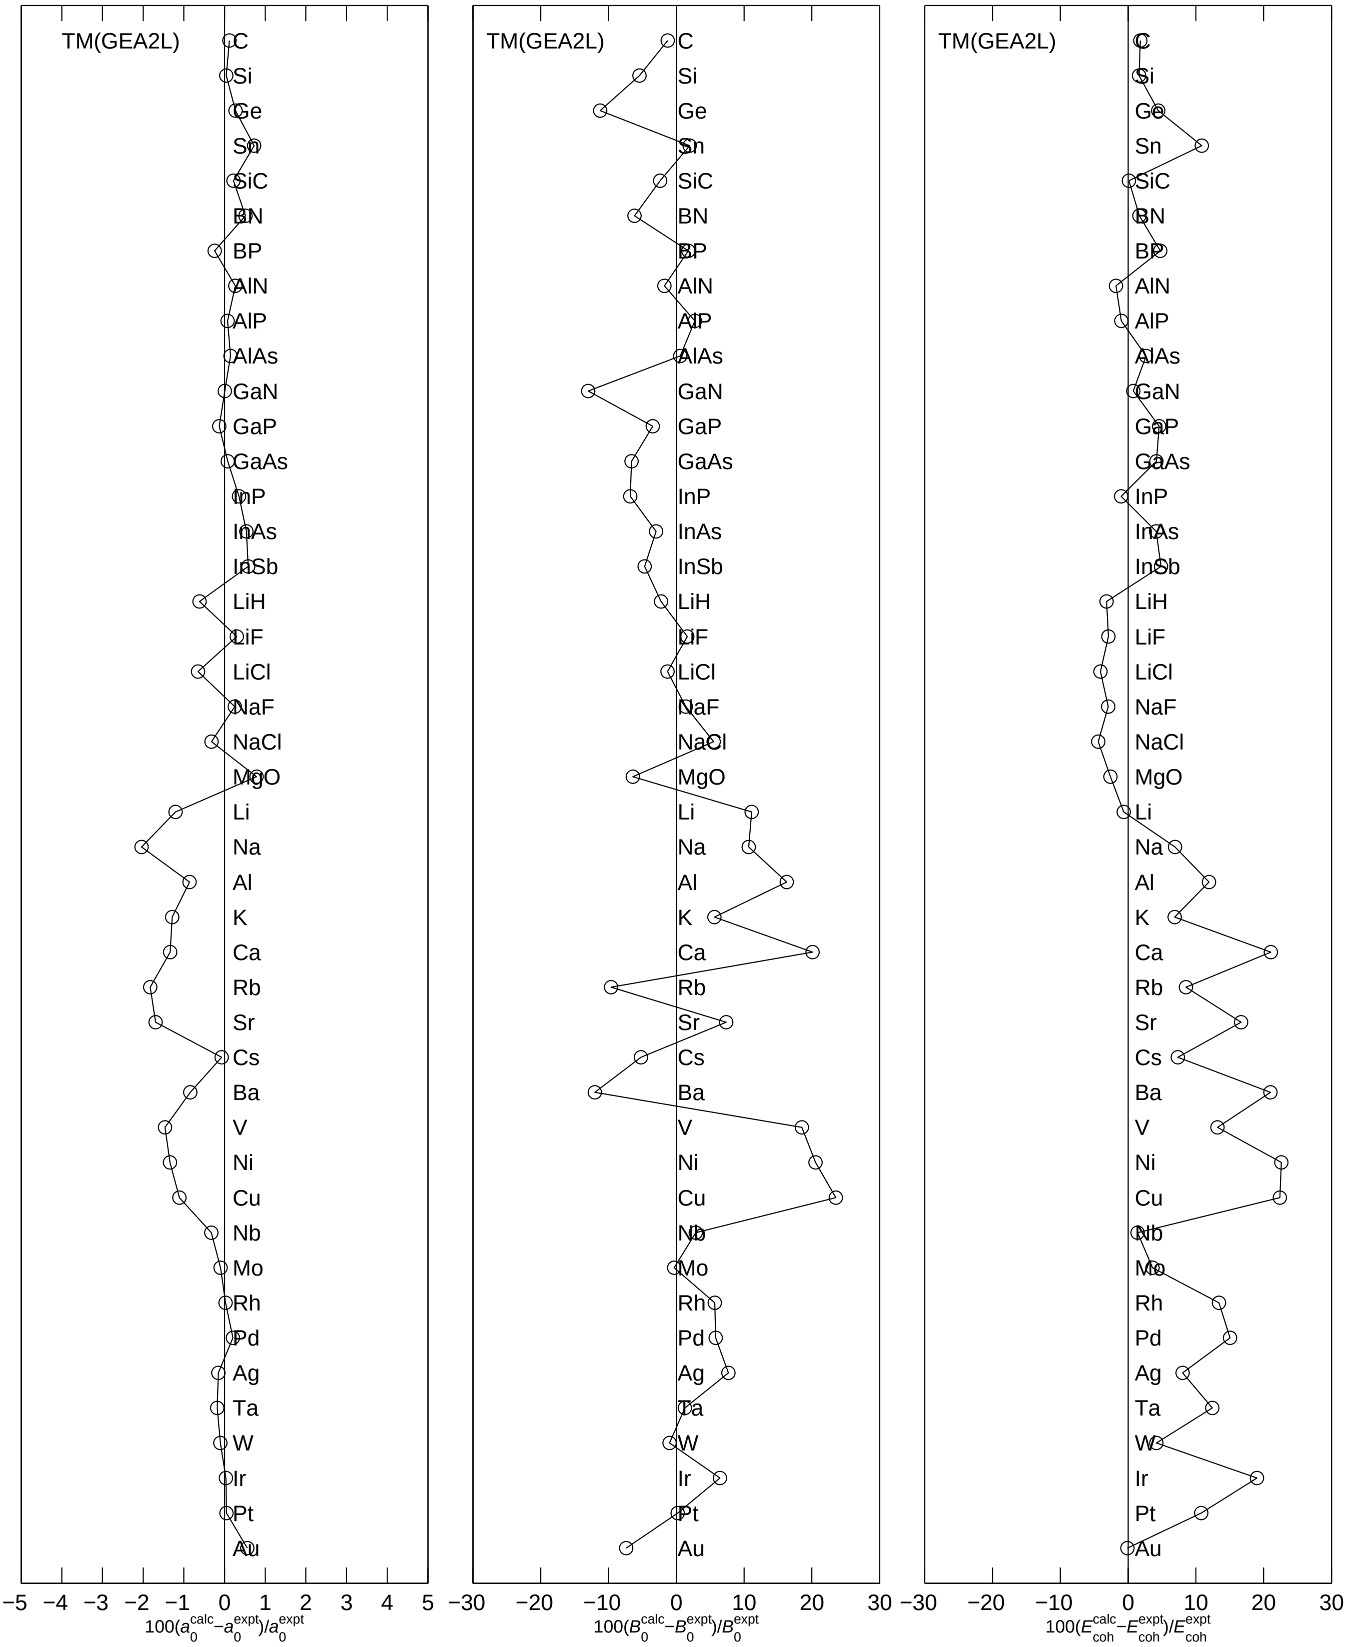


FIG. S18. Relative error (in %) in the calculated lattice constants $a_0$ (left), bulk modulus $B_0$ (middle), and cohesive energy $E_{\rm coh}$ (right) with respect to the experimental values.

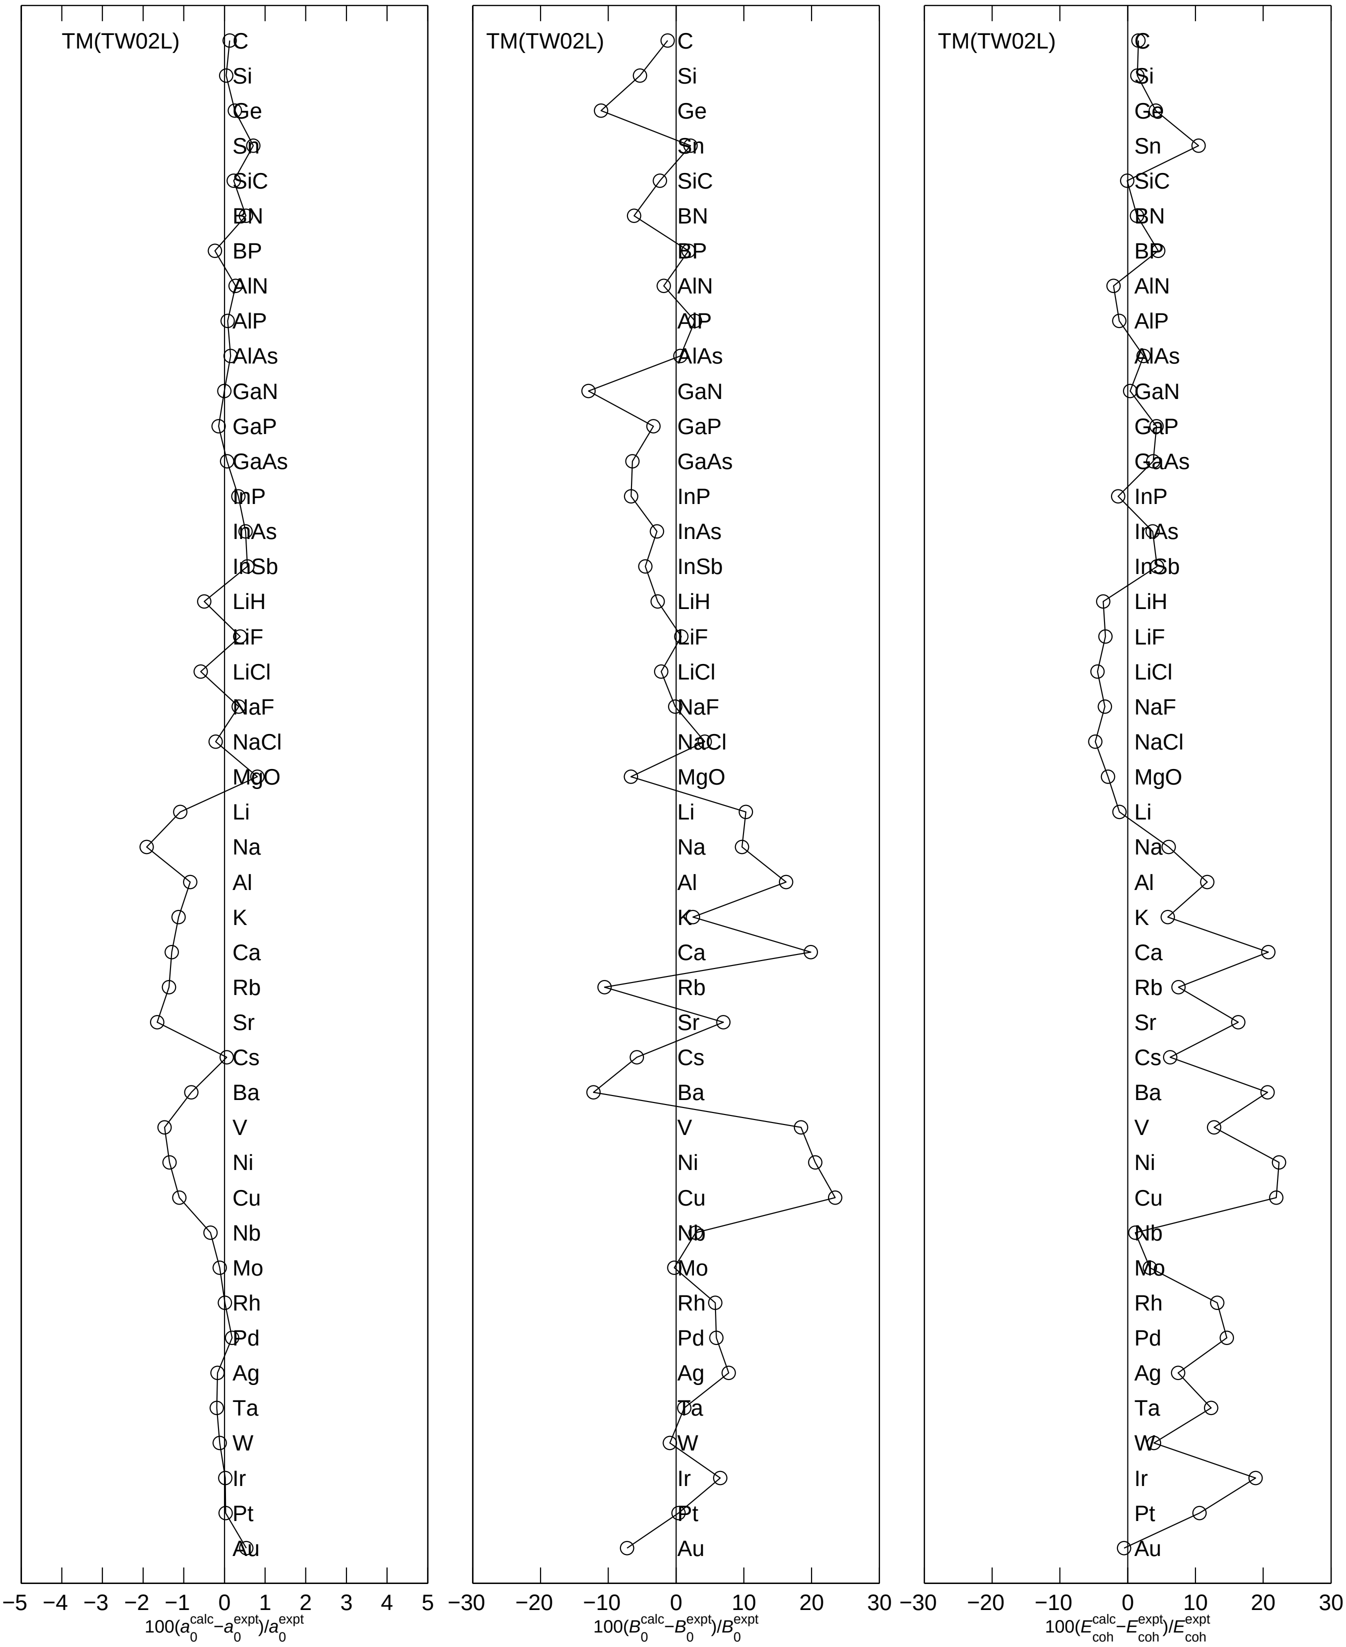


FIG. S19. Relative error (in %) in the calculated lattice constants $a_0$ (left), bulk modulus $B_0$ (middle), and cohesive energy $E_{\rm coh}$ (right) with respect to the experimental values.

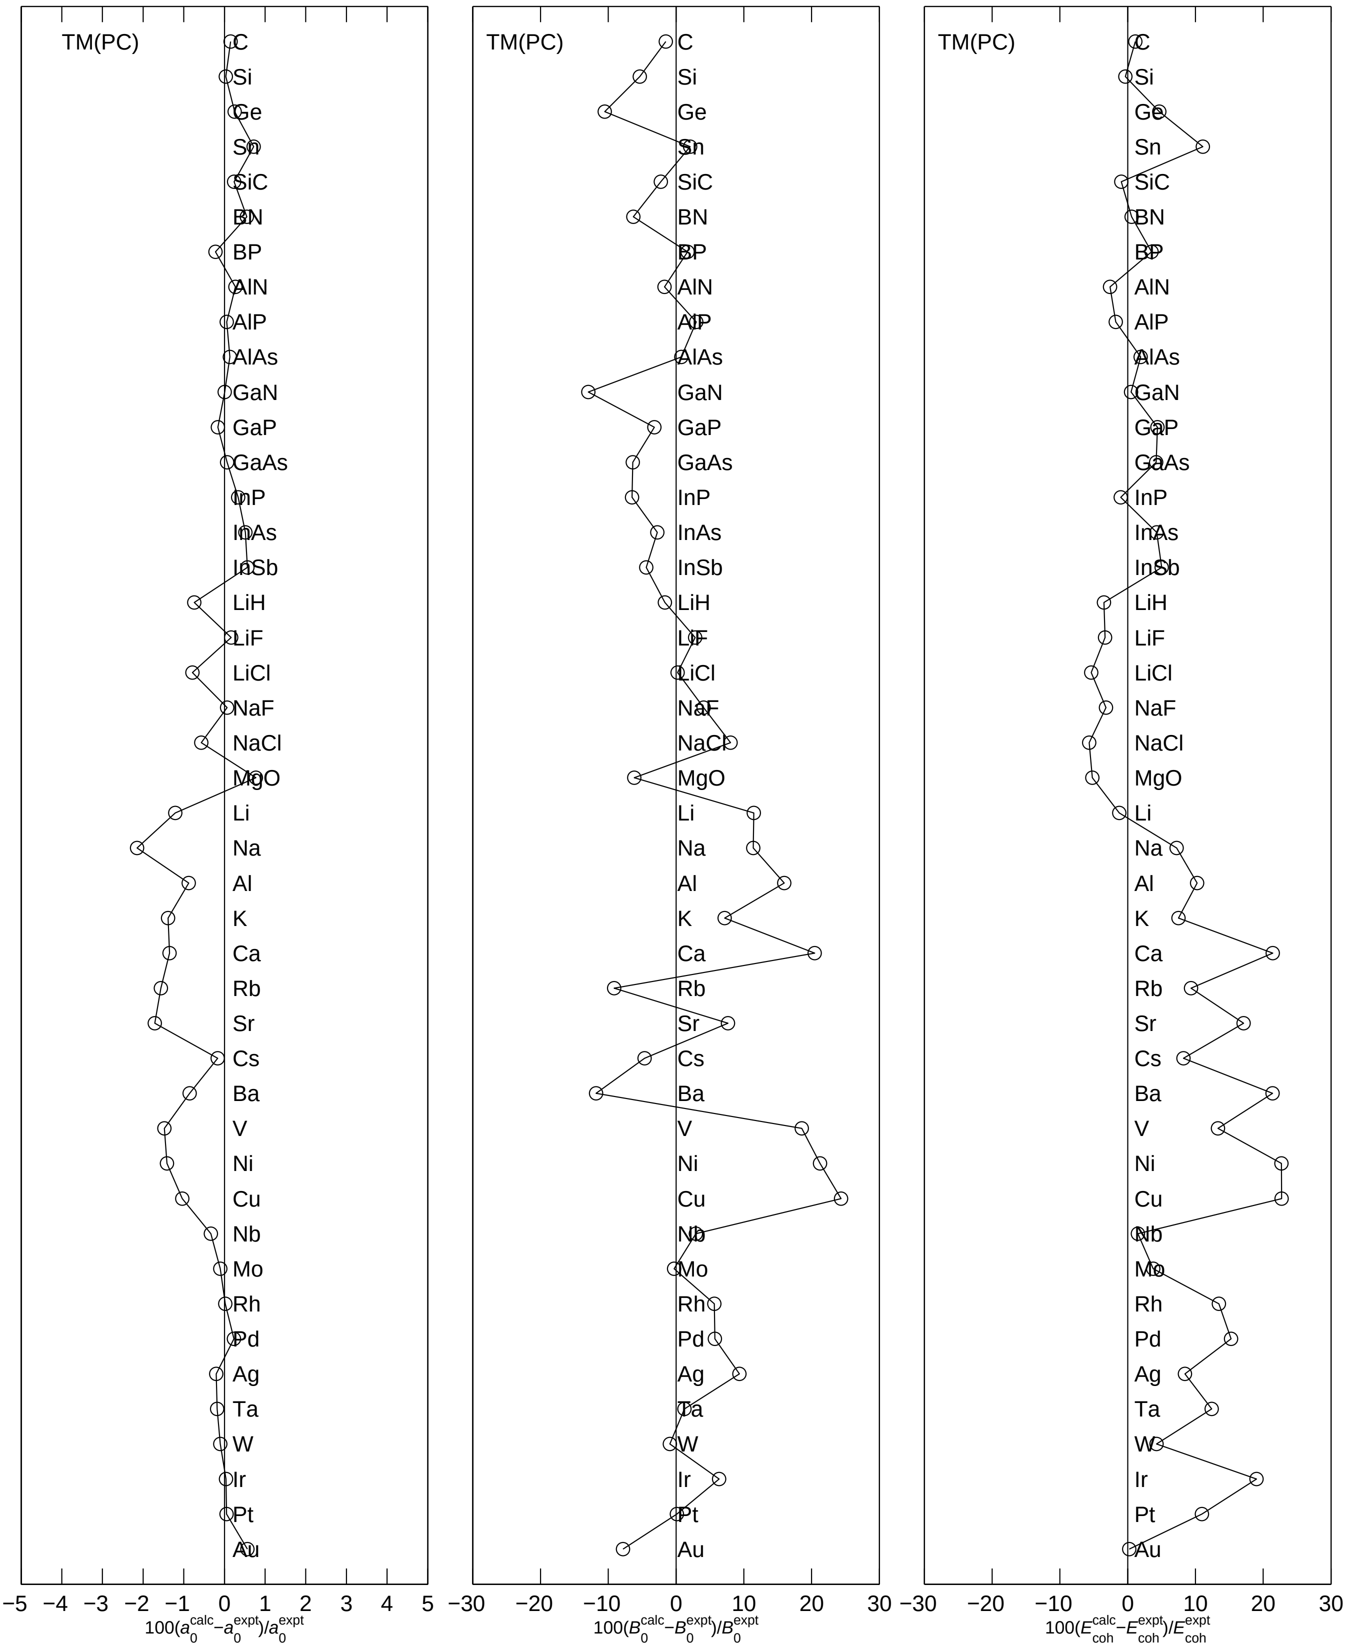


FIG. S20. Relative error (in %) in the calculated lattice constants $a_0$ (left), bulk modulus $B_0$ (middle), and cohesive energy $E_{\rm coh}$ (right) with respect to the experimental values.

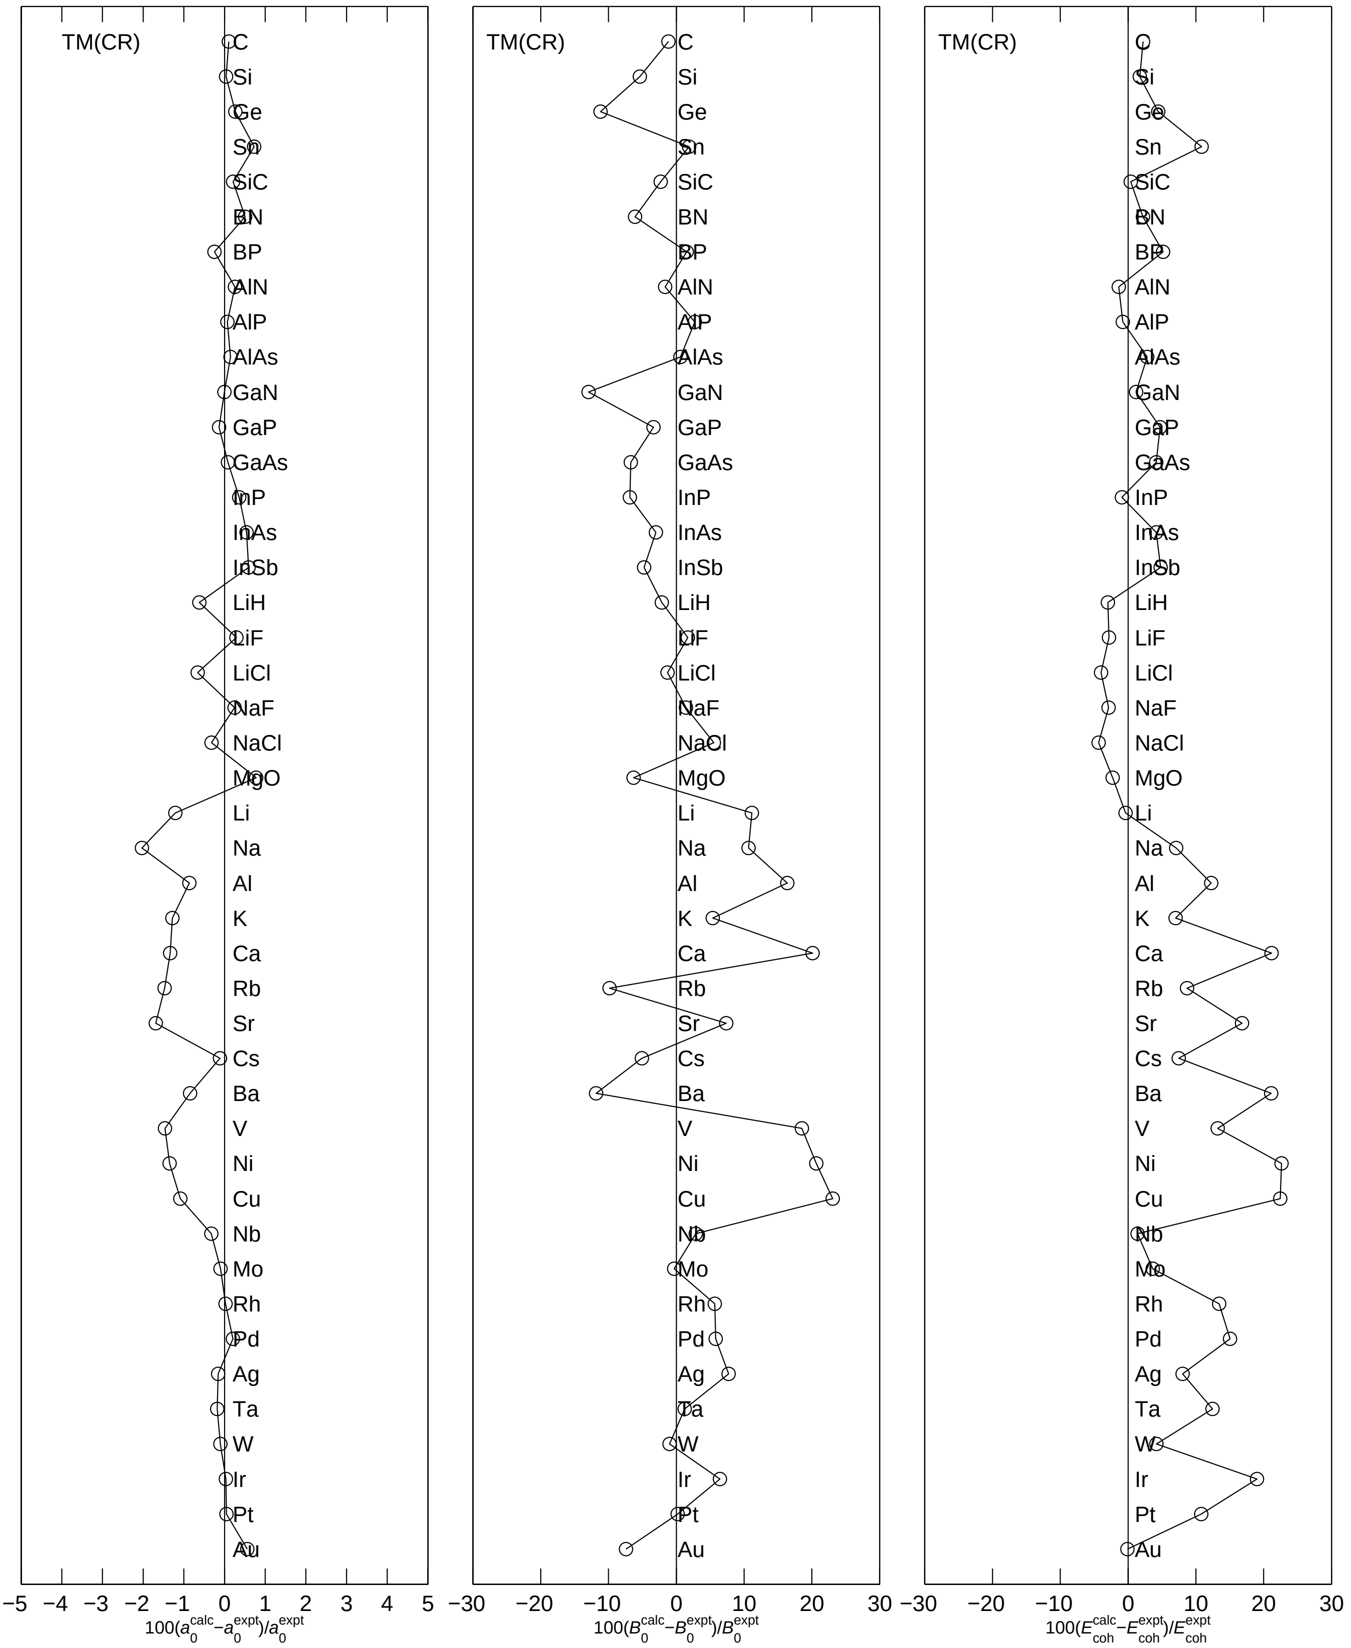


FIG. S21. Relative error (in %) in the calculated lattice constants $a_0$ (left), bulk modulus $B_0$ (middle), and cohesive energy $E_{\rm coh}$ (right) with respect to the experimental values.

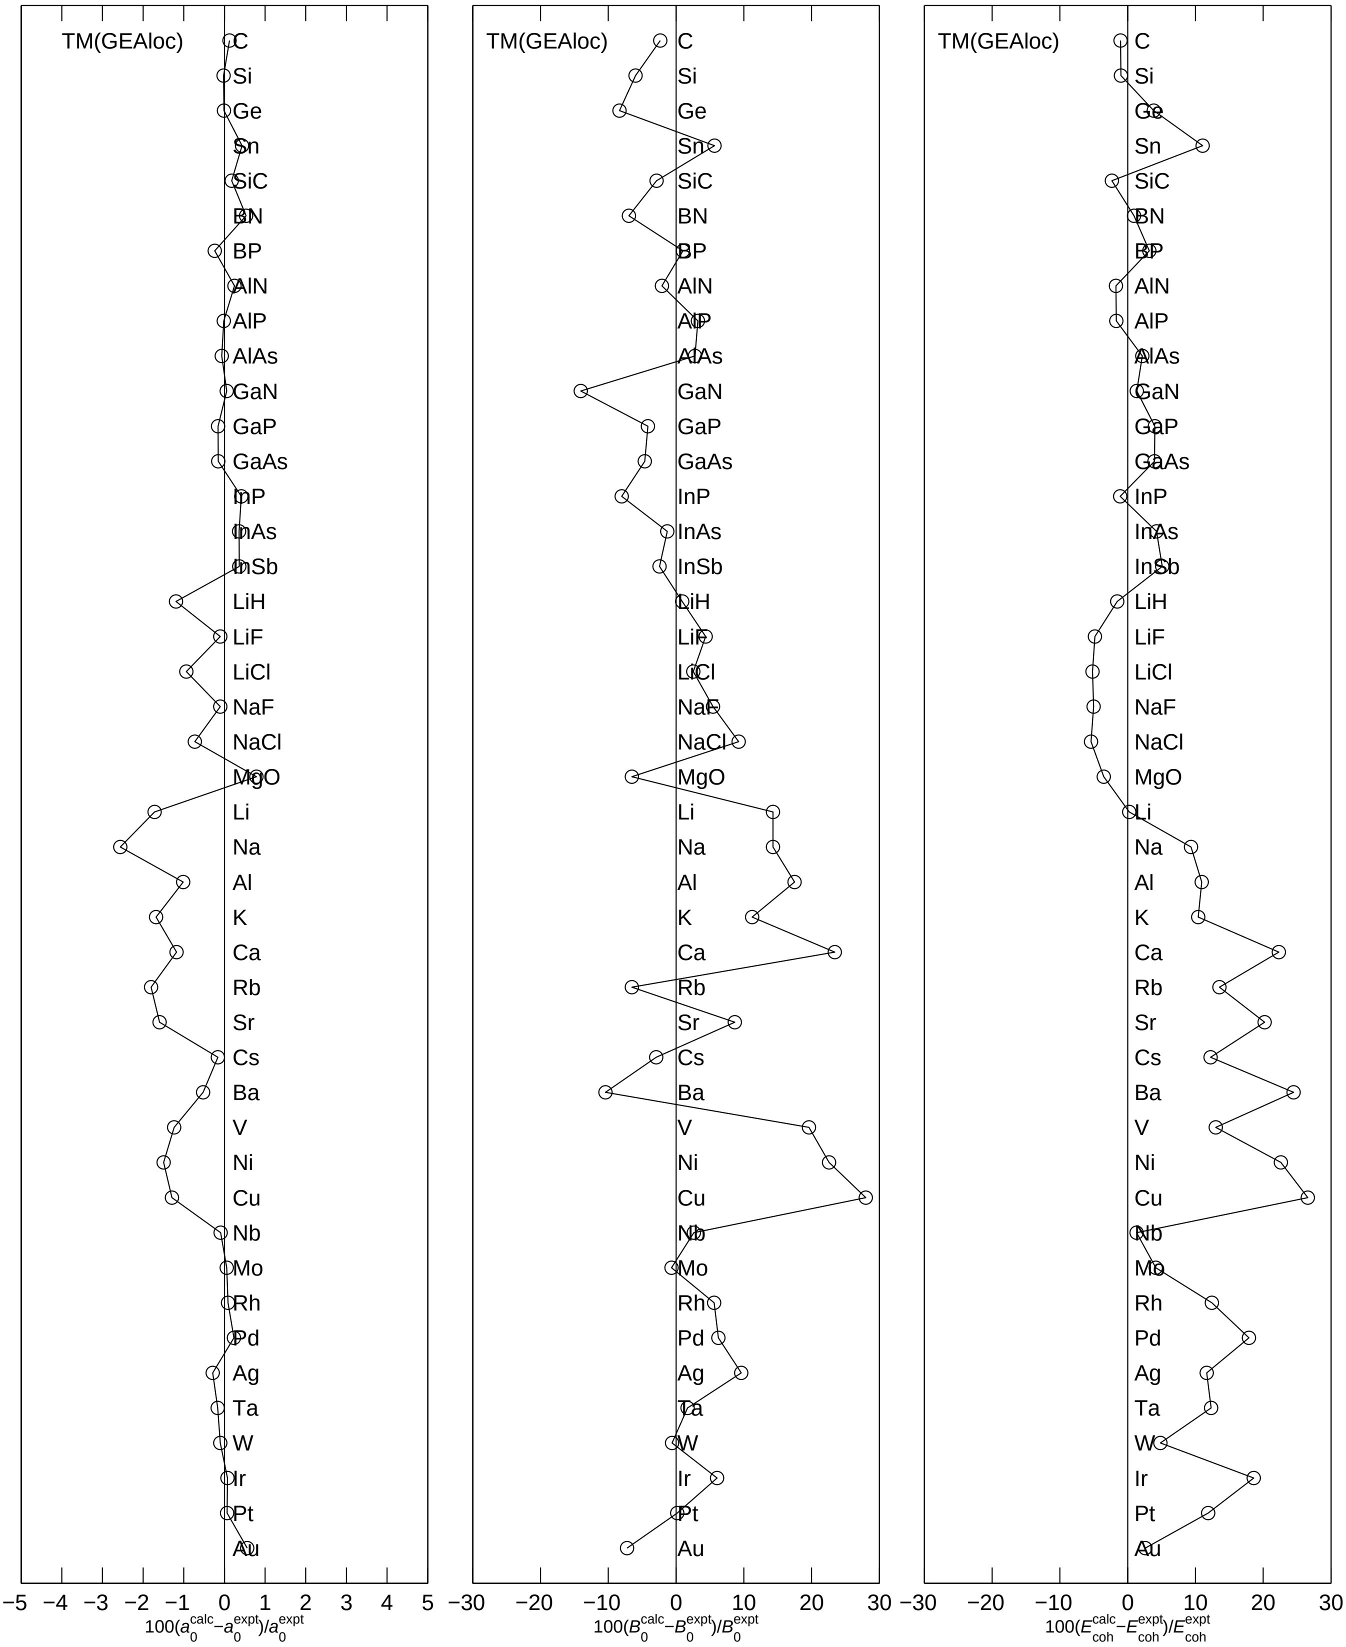


FIG. S22. Relative error (in %) in the calculated lattice constants $a_0$ (left), bulk modulus $B_0$ (middle), and cohesive energy $E_{\rm coh}$ (right) with respect to the experimental values.

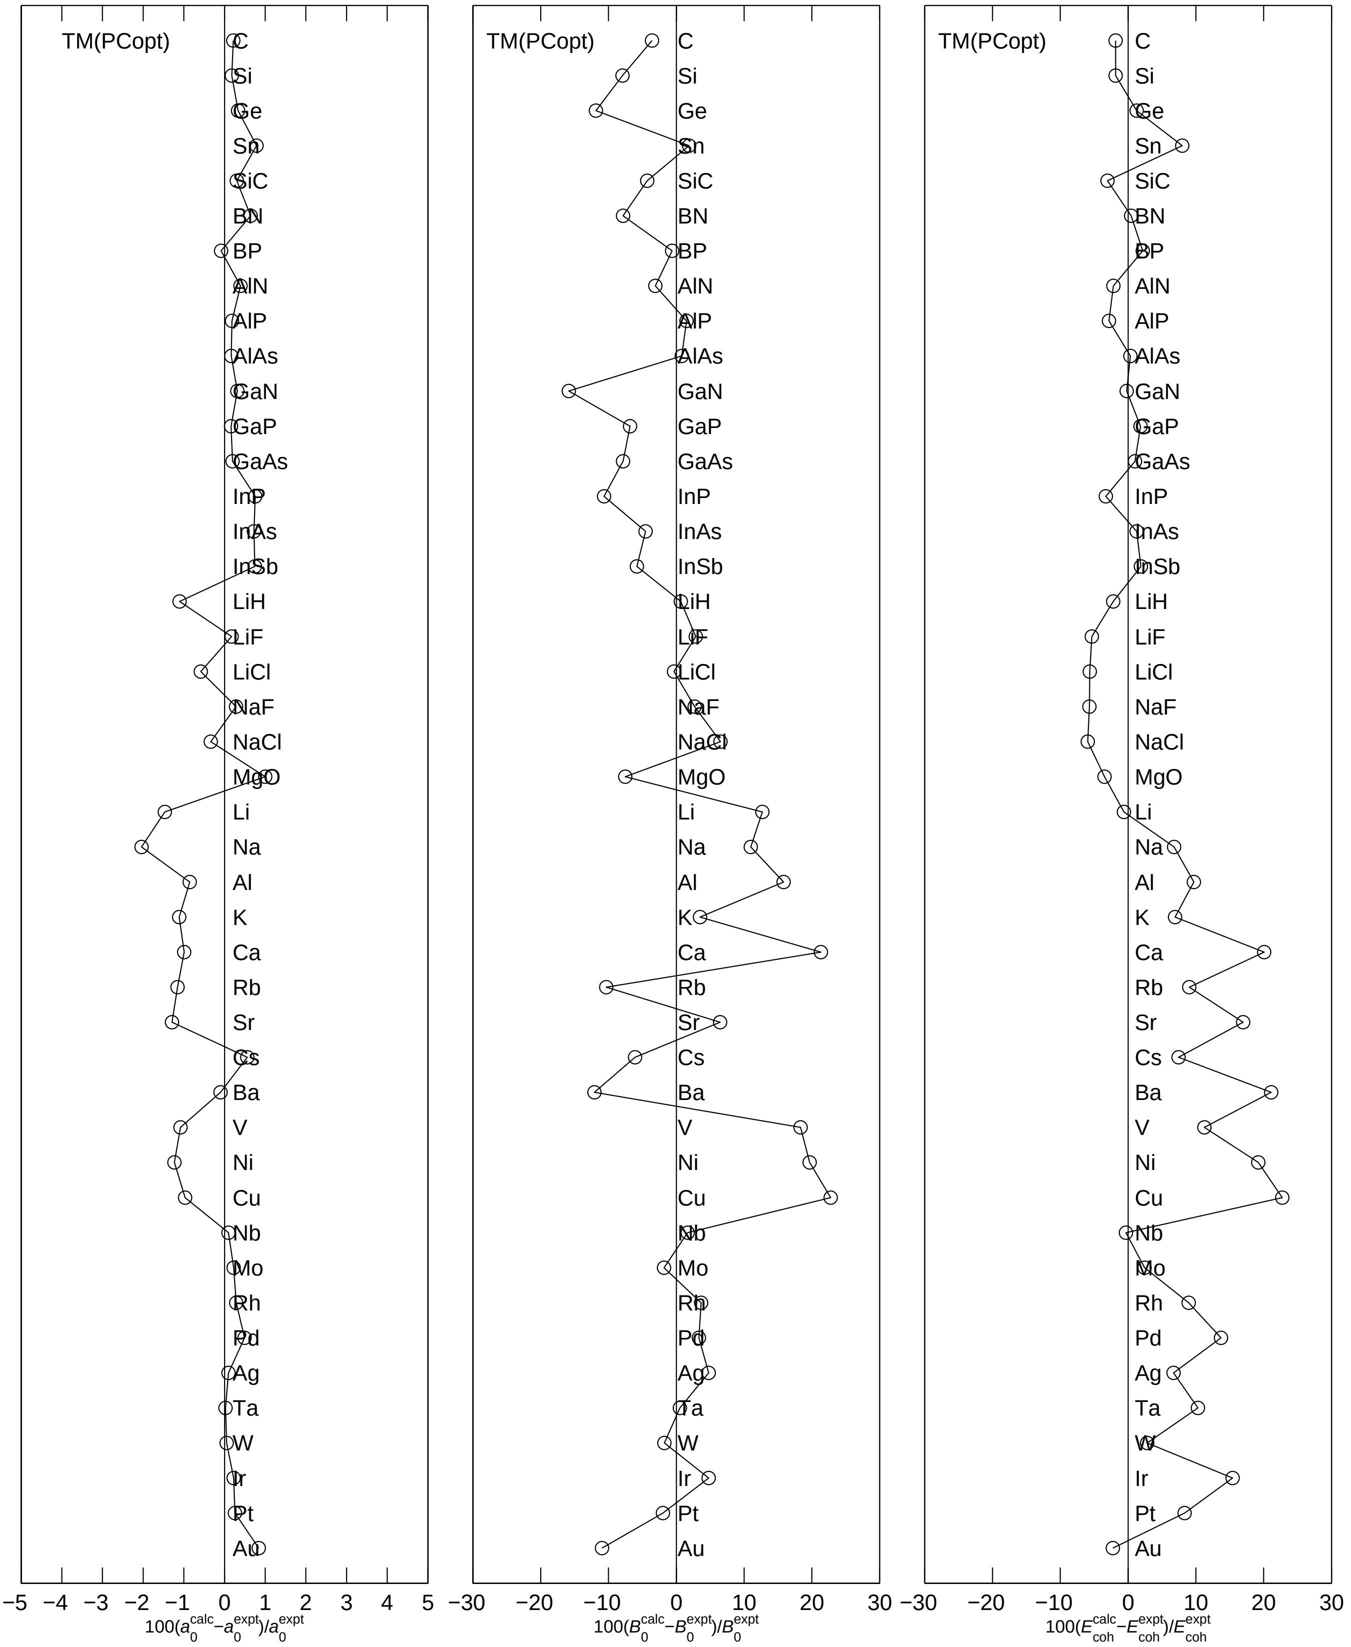


FIG. S23. Relative error (in %) in the calculated lattice constants $a_0$ (left), bulk modulus $B_0$ (middle), and cohesive energy $E_{\rm coh}$ (right) with respect to the experimental values.

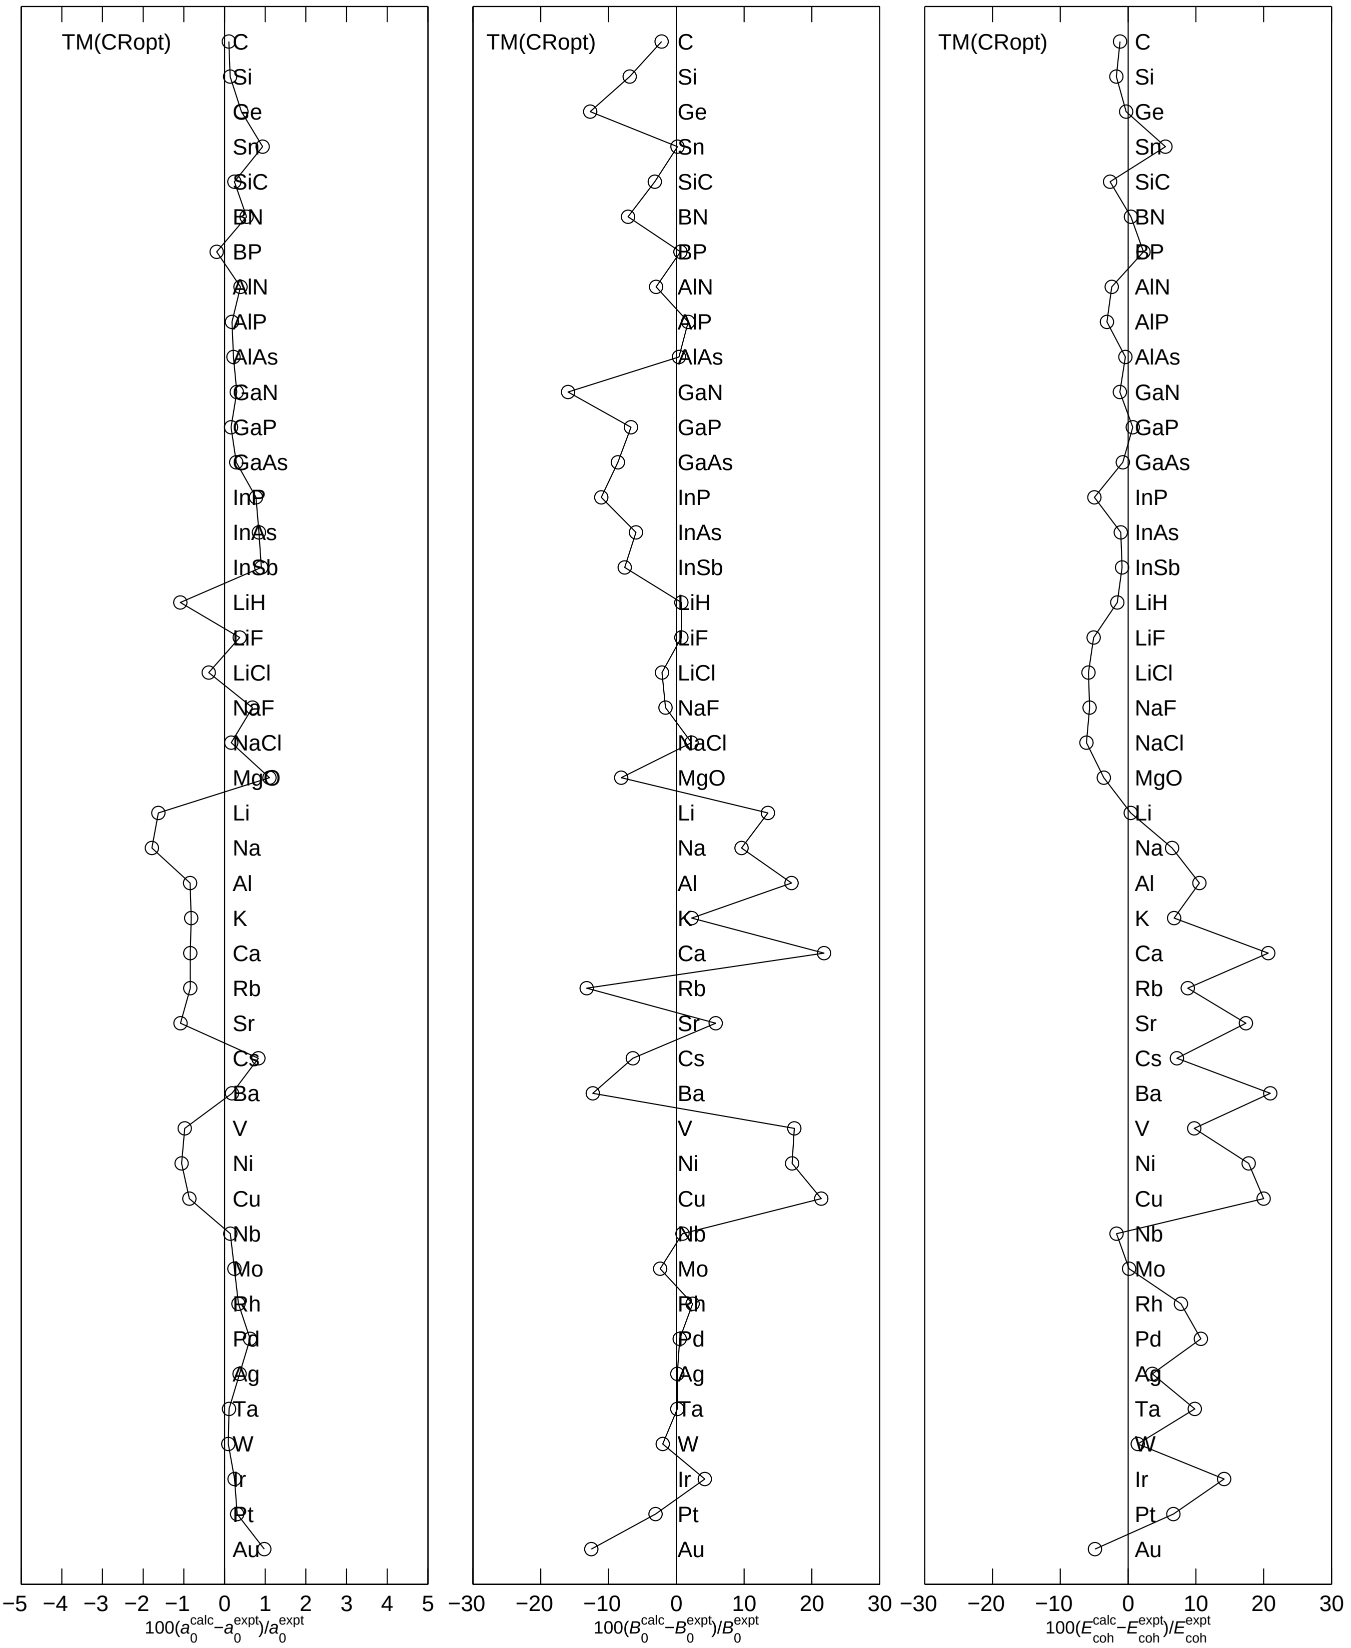


FIG. S24. Relative error (in %) in the calculated lattice constants $a_0$ (left), bulk modulus $B_0$ (middle), and cohesive energy $E_{\mathrm{coh}}$ (right) with respect to the experimental values.

TABLE S10. Experimental[3–6] lattice constants (in Å) and angles (in degrees) of the unit cell for the solids considered in this work. When necessary, the positions of atoms (in internal units) are indicated at the second line. The space group number is indicated in parenthesis. For $Cr_2O_3$, $Fe_2O_3$, MnO, FeO, CoO and NiO, the antiferromagnetic order leads to a lowering of the symmetry (second indicated space group).

| solid | $a$ | $b$ | $c$ | $\alpha$ | $\beta$ | $\gamma$ |
|---|---|---|---|---|---|---|
| Ne (225) | 4.470 | 4.470 | 4.470 | 90 | 90 | 90 |
| Ar (225) | 5.260 | 5.260 | 5.260 | 90 | 90 | 90 |
| Kr (225) | 5.640 | 5.640 | 5.640 | 90 | 90 | 90 |
| Xe (225) | 6.130 | 6.130 | 6.130 | 90 | 90 | 90 |
| C (227) | 3.567 | 3.567 | 3.567 | 90 | 90 | 90 |
| Si (227) | 5.430 | 5.430 | 5.430 | 90 | 90 | 90 |
| Ge (227) | 5.652 | 5.652 | 5.652 | 90 | 90 | 90 |
| $Al_2O_3$ (167) | 4.757 | 4.757 | 12.988 | 90 | 90 | 120 |
| Al(0,0,0.35218), O(0.30625,0,1/4) | | | | | | |
| SiC (216) | 4.358 | 4.358 | 4.358 | 90 | 90 | 90 |
| $SiO_2$ ($\alpha$-quartz,152) | 4.921 | 4.921 | 5.400 | 90 | 90 | 120 |
| Si(0.528,0,1/3), O(0.408,0.143,0.1193) | | | | | | |
| $SiO_2$ ($\beta$-cristobalite,227) | 7.126 | 7.126 | 7.126 | 90 | 90 | 90 |
| BN (216) | 3.616 | 3.616 | 3.616 | 90 | 90 | 90 |
| BP (216) | 4.538 | 4.538 | 4.538 | 90 | 90 | 90 |
| BAs (216) | 4.777 | 4.777 | 4.777 | 90 | 90 | 90 |
| AlN (216) | 4.342 | 4.342 | 4.342 | 90 | 90 | 90 |
| AlN (wurtzite,186) | 3.111 | 3.111 | 4.978 | 90 | 90 | 120 |
| Al(1/3,2/3,0), N(1/3,2/3,0.385) | | | | | | |
| AlP (216) | 5.463 | 5.463 | 5.463 | 90 | 90 | 90 |
| AlAs (216) | 5.661 | 5.661 | 5.661 | 90 | 90 | 90 |
| AlSb (216) | 6.136 | 6.136 | 6.136 | 90 | 90 | 90 |
| GaN (216) | 4.523 | 4.523 | 4.523 | 90 | 90 | 90 |
| GaN (wurtzite,186) | 3.180 | 3.180 | 5.166 | 90 | 90 | 120 |
| Ga(1/3,2/3,0), N(1/3,2/3,0.385) | | | | | | |
| GaP (216) | 5.451 | 5.451 | 5.451 | 90 | 90 | 90 |
| GaSb (216) | 6.096 | 6.096 | 6.096 | 90 | 90 | 90 |
| GaAs (216) | 5.648 | 5.648 | 5.648 | 90 | 90 | 90 |
| InN (wurtzite,186) | 3.533 | 3.533 | 5.693 | 90 | 90 | 120 |
| In(1/3,2/3,0), N(1/3,2/3,0.385) | | | | | | |
| InP (216) | 5.869 | 5.869 | 5.869 | 90 | 90 | 90 |
| InAs (216) | 6.058 | 6.058 | 6.058 | 90 | 90 | 90 |
| InSb (216) | 6.479 | 6.479 | 6.479 | 90 | 90 | 90 |
| $SnO_2$ (136) | 4.737 | 4.737 | 3.186 | 90 | 90 | 90 |
| Sn(0,0,0), O(0.30562,0.30562,0) | | | | | | |
| SnSe (62) | 11.500 | 4.154 | 4.446 | 90 | 90 | 90 |
| Sn(0.618,1/4,0.3957), Se(0.3559,1/4,0.0164) | | | | | | |
| SnTe (225) | 6.318 | 6.318 | 6.318 | 90 | 90 | 90 |
| $Sb_2Te_3$ (166) | 4.264 | 4.264 | 30.458 | 90 | 90 | 120 |
| Sb(0,0,0.3988), Te1(0,0,0.7872), Te2(0,0,0) | | | | | | |
| LiH (225) | 4.084 | 4.084 | 4.084 | 90 | 90 | 90 |
| LiF (225) | 4.010 | 4.010 | 4.010 | 90 | 90 | 90 |
| LiCl (225) | 5.106 | 5.106 | 5.106 | 90 | 90 | 90 |
| NaF (225) | 4.609 | 4.609 | 4.609 | 90 | 90 | 90 |
| NaCl (225) | 5.595 | 5.595 | 5.595 | 90 | 90 | 90 |
| KF (225) | 5.347 | 5.347 | 5.347 | 90 | 90 | 90 |
| KCl (225) | 6.293 | 6.293 | 6.293 | 90 | 90 | 90 |
| BeO (wurtzite,186) | 2.694 | 2.694 | 4.384 | 90 | 90 | 120 |
| Be(1/3,2/3,0), O(1/3,2/3,0.3778) | | | | | | |
| MgO (225) | 4.207 | 4.207 | 4.207 | 90 | 90 | 90 |
| MgS (216) | 5.622 | 5.622 | 5.622 | 90 | 90 | 90 |
| MgSe (225) | 5.400 | 5.400 | 5.400 | 90 | 90 | 90 |
| MgTe (216) | 6.420 | 6.420 | 6.420 | 90 | 90 | 90 |
| CaO (225) | 4.811 | 4.811 | 4.811 | 90 | 90 | 90 |
| $CaF_2$ (225) | 5.463 | 5.463 | 5.463 | 90 | 90 | 90 |
| BaS (225) | 6.389 | 6.389 | 6.389 | 90 | 90 | 90 |
| BaSe (225) | 6.595 | 6.595 | 6.595 | 90 | 90 | 90 |
| BaTe (225) | 7.007 | 7.007 | 7.007 | 90 | 90 | 90 |
| ScN (225) | 4.500 | 4.500 | 4.500 | 90 | 90 | 90 |
| $TiO_2$ (rutile,136) | 4.594 | 4.594 | 2.959 | 90 | 90 | 90 |
| Ti(0,0,0), O(0.305,0.305,0) | | | | | | |
| $TiO_2$ (anatase,141) | 3.785 | 3.785 | 9.512 | 90 | 90 | 90 |
| Ti(0,1/4,3/8), O(1/2,3/4,0.08314) | | | | | | |
| $SrTiO_3$ (221) | 3.901 | 3.901 | 3.901 | 90 | 90 | 90 |
| $VO_2$ ($M_1$,14) | 5.743 | 4.517 | 5.375 | 90 | 122.6 | 90 |
| V(0.242,0.975,0.025), O1(0.1,0.21,0.2), O2(0.39,0.69,0.29) | | | | | | |
| $Cr_2O_3$ (167,146) | 4.953 | 4.953 | 13.588 | 90 | 90 | 120 |
| Cr(0,0,0.3475), O(0.3058,0,1/4) | | | | | | |
| $Fe_2O_3$ (167,146) | 5.035 | 5.035 | 13.747 | 90 | 90 | 120 |
| Fe(0,0,0.35534), O(0.3056,0,1/4) | | | | | | |
| MnO (225,166) | 4.445 | 4.445 | 4.445 | 90 | 90 | 90 |
| FeO (225,166) | 4.334 | 4.334 | 4.334 | 90 | 90 | 90 |
| CoO (225,166) | 4.254 | 4.254 | 4.254 | 90 | 90 | 90 |
| NiO (225,166) | 4.171 | 4.171 | 4.171 | 90 | 90 | 90 |
| $Cu_2O$ (224) | 4.267 | 4.267 | 4.267 | 90 | 90 | 90 |
| CuSCN (160) | 3.856 | 3.856 | 16.452 | 90 | 90 | 120 |
| Cu(0,0,0), S(0.28904,0.28904,0.28904), C(0.18674,0.18674,0.18674), N(0.1169,0.1169,0.1169) | | | | | | |
| CuCl (216) | 5.501 | 5.501 | 5.501 | 90 | 90 | 90 |
| CuBr (216) | 5.820 | 5.820 | 5.820 | 90 | 90 | 90 |
| CuI (216) | 6.063 | 6.063 | 6.063 | 90 | 90 | 90 |
| ZnO (wurtzite,186) | 3.258 | 3.258 | 5.220 | 90 | 90 | 120 |
| Zn(1/3,2/3,0), O(1/3,2/3,0.382) | | | | | | |
| ZnS (216) | 5.409 | 5.409 | 5.409 | 90 | 90 | 90 |
| ZnSe (216) | 5.668 | 5.668 | 5.668 | 90 | 90 | 90 |
| ZnTe (216) | 6.089 | 6.089 | 6.089 | 90 | 90 | 90 |
| $MoS_2$ (194) | 3.160 | 3.160 | 12.294 | 90 | 90 | 120 |
| Mo(1/3,2/3,1/4), S(1/3,2/3,0.621) | | | | | | |
| AgCl (225) | 5.546 | 5.546 | 5.546 | 90 | 90 | 90 |
| AgBr (225) | 5.772 | 5.772 | 5.772 | 90 | 90 | 90 |
| AgI (216) | 6.499 | 6.499 | 6.499 | 90 | 90 | 90 |
| CdS (216) | 5.818 | 5.818 | 5.818 | 90 | 90 | 90 |
| CdSe (216) | 6.052 | 6.052 | 6.052 | 90 | 90 | 90 |
| CdTe (216) | 6.480 | 6.480 | 6.480 | 90 | 90 | 90 |

TABLE S11. Fundamental band gap (in eV) of 76 solids calculated with mBJLDA (mBJ) and its deorbitalized versions. The experimental values[1,6–15] are also shown.

| Solid | mBJ | mBJ(GEA2L) | mBJ(TW02L) | mBJ(PC) | mBJ(CR) | mBJ(GEAloc) | mBJ(PCopt) | mBJ(CRopt) | Expt. |
|---|---|---|---|---|---|---|---|---|---|
| Ne (225) | 22.33 | 21.62 | 20.24 | 14.79 | 21.68 | 30.24 | 16.95 | 27.73 | 21.48 |
| Ar (225) | 13.84 | 14.13 | 13.54 | 11.24 | 14.14 | 20.01 | 12.98 | 18.08 | 14.15 |
| Kr (225) | 10.80 | 10.90 | 10.54 | 9.23 | 10.91 | 15.55 | 10.51 | 13.58 | 11.59 |
| Xe (225) | 8.48 | 8.59 | 8.38 | 7.71 | 8.59 | 11.17 | 8.62 | 10.41 | 9.29 |
| C (227) | 4.92 | 4.57 | 4.59 | 4.54 | 4.59 | 5.29 | 5.20 | 4.96 | 5.50 |
| Si (227) | 1.15 | 0.93 | 0.92 | 0.94 | 0.93 | 1.63 | 1.47 | 1.24 | 1.17 |
| Ge (227) | 0.83 | 0.20 | 0.19 | 0.20 | 0.21 | 0.66 | 0.50 | 0.22 | 0.74 |
| $Al_2O_3$ (167) | 8.34 | 7.15 | 7.11 | 7.13 | 7.20 | 8.62 | 7.89 | 8.35 | 8.80 |
| SiC (216) | 2.25 | 1.76 | 1.76 | 1.77 | 1.77 | 2.47 | 2.36 | 2.21 | 2.42 |
| $SiO_2$ ($\alpha$-quartz,152) | 8.70 | 7.37 | 7.29 | 6.95 | 7.42 | 8.84 | 7.74 | 8.57 | 9.65 |
| $SiO_2$ ($\beta$-cristobalite,227) | 10.43 | 9.26 | 8.99 | 8.52 | 9.32 | 10.79 | 9.65 | 10.54 | 8.90 |
| BN (216) | 5.80 | 5.17 | 5.16 | 5.19 | 5.19 | 6.32 | 6.07 | 5.90 | 6.36 |
| BP (216) | 1.85 | 1.60 | 1.60 | 1.59 | 1.61 | 2.26 | 2.16 | 1.94 | 2.10 |
| BAs (216) | 1.71 | 1.53 | 1.53 | 1.53 | 1.53 | 2.01 | 1.91 | 1.78 | 1.46 |
| AlN (216) | 4.88 | 3.95 | 3.93 | 4.00 | 3.96 | 4.98 | 4.70 | 4.74 | 4.90 |
| AlN (wurtzite,186) | 5.51 | 4.60 | 4.59 | 4.57 | 4.64 | 5.42 | 5.05 | 5.29 | 6.19 |
| AlP (216) | 2.31 | 2.05 | 2.04 | 2.08 | 2.05 | 2.94 | 2.69 | 2.53 | 2.50 |
| AlAs (216) | 2.13 | 1.88 | 1.86 | 1.91 | 1.88 | 2.54 | 2.33 | 2.25 | 2.23 |
| AlSb (216) | 1.75 | 1.57 | 1.55 | 1.58 | 1.57 | 2.03 | 1.85 | 1.81 | 1.69 |
| GaN (216) | 2.85 | 1.92 | 1.91 | 1.86 | 1.95 | 2.44 | 2.26 | 2.38 | 3.28 |
| GaN (wurtzite,186) | 3.17 | 2.22 | 2.21 | 2.16 | 2.26 | 2.78 | 2.57 | 2.71 | 3.50 |
| GaP (216) | 2.25 | 2.07 | 2.06 | 2.07 | 2.08 | 2.79 | 2.57 | 2.38 | 2.35 |
| GaSb (216) | 0.95 | 0.25 | 0.24 | 0.25 | 0.25 | 0.69 | 0.54 | 0.30 | 0.82 |
| GaAs (216) | 1.64 | 0.85 | 0.83 | 0.86 | 0.85 | 1.48 | 1.25 | 1.04 | 1.52 |
| InN (wurtzite,186) | 0.89 | 0.15 | 0.14 | 0.12 | 0.17 | 0.63 | 0.47 | 0.53 | 0.72 |
| InP (216) | 1.62 | 1.06 | 1.04 | 1.06 | 1.07 | 1.83 | 1.51 | 1.39 | 1.42 |
| InAs (216) | 0.67 | 0.08 | 0.06 | 0.09 | 0.08 | 0.71 | 0.47 | 0.28 | 0.42 |
| InSb (216) | 0.47 | 0.00 | 0.00 | 0.00 | 0.00 | 0.41 | 0.24 | 0.03 | 0.24 |
| $SnO_2$ (136) | 3.19 | 1.83 | 1.82 | 1.77 | 1.87 | 3.00 | 2.49 | 2.68 | 3.59 |
| SnSe (62) | 0.89 | 0.81 | 0.80 | 0.84 | 0.81 | 1.20 | 1.05 | 1.12 | 0.90 |
| SnTe (225) | 0.15 | 0.16 | 0.15 | 0.19 | 0.16 | 0.43 | 0.32 | 0.41 | 0.36 |
| $Sb_2Te_3$ (166) | 0.24 | 0.17 | 0.16 | 0.18 | 0.17 | 0.29 | 0.32 | 0.31 | 0.28 |
| LiH (225) | 5.06 | 4.24 | 4.18 | 4.93 | 4.12 | 6.69 | 5.03 | 5.25 | 4.94 |
| LiF (225) | 12.89 | 11.23 | 11.15 | 10.69 | 11.30 | 14.74 | 11.94 | 13.99 | 14.20 |
| LiCl (225) | 8.64 | 8.08 | 8.01 | 7.81 | 8.10 | 11.04 | 8.88 | 9.97 | 9.40 |
| NaF (225) | 11.46 | 9.76 | 9.55 | 8.66 | 9.80 | 14.36 | 9.82 | 13.17 | 11.50 |
| NaCl (225) | 8.45 | 7.88 | 7.72 | 7.22 | 7.89 | 12.19 | 8.37 | 10.40 | 8.50 |
| KF (225) | 10.40 | 9.41 | 9.14 | 8.30 | 9.44 | 12.29 | 9.38 | 11.75 | 10.90 |
| KCl (225) | 8.48 | 8.15 | 7.90 | 7.15 | 8.16 | 11.76 | 8.29 | 10.46 | 8.50 |
| BeO (wurtzite,186) | 9.66 | 8.44 | 8.42 | 8.38 | 8.50 | 9.92 | 9.26 | 9.71 | 10.60 |
| MgO (225) | 7.13 | 5.86 | 5.82 | 5.91 | 5.91 | 7.57 | 6.68 | 7.24 | 7.83 |
| MgS (216) | 5.17 | 4.63 | 4.58 | 4.66 | 4.64 | 6.34 | 5.48 | 5.73 | 4.78 |
| MgSe (225) | 2.93 | 2.59 | 2.54 | 2.70 | 2.59 | 3.54 | 3.12 | 3.16 | 2.47 |
| MgTe (216) | 3.61 | 3.20 | 3.16 | 3.25 | 3.20 | 4.22 | 3.75 | 3.85 | 3.60 |
| CaO (225) | 5.35 | 4.64 | 4.58 | 4.72 | 4.65 | 5.60 | 5.13 | 5.21 | 7.00 |
| $CaF_2$ (225) | 10.34 | 9.70 | 9.58 | 9.53 | 9.71 | 10.31 | 9.84 | 10.09 | 11.80 |
| BaS (225) | 3.27 | 2.97 | 2.92 | 3.00 | 2.97 | 4.03 | 3.51 | 3.55 | 3.88 |
| BaSe (225) | 2.86 | 2.60 | 2.56 | 2.65 | 2.60 | 3.41 | 3.02 | 3.05 | 3.58 |
| BaTe (225) | 2.28 | 2.11 | 2.07 | 2.16 | 2.11 | 2.74 | 2.43 | 2.46 | 3.08 |
| ScN (225) | 0.88 | 0.44 | 0.42 | 0.49 | 0.45 | 1.06 | 0.87 | 0.78 | 0.90 |
| $TiO_2$ (rutile,136) | 2.56 | 2.17 | 2.16 | 2.19 | 2.17 | 2.49 | 2.28 | 2.30 | 3.30 |
| $TiO_2$ (anatase,141) | 2.92 | 2.47 | 2.46 | 2.50 | 2.47 | 2.87 | 2.61 | 2.65 | 3.40 |
| $SrTiO_3$ (221) | 2.68 | 2.24 | 2.23 | 2.27 | 2.24 | 2.63 | 2.40 | 2.43 | 3.30 |
| $VO_2$ ($M_1$,14) | 0.51 | 0.02 | 0.00 | 0.04 | 0.02 | 0.48 | 0.43 | 0.35 | 0.60 |
| $Cr_2O_3$ (167,146) | 3.68 | 2.43 | 2.42 | 2.46 | 2.44 | 3.66 | 3.27 | 3.13 | 3.40 |
| $Fe_2O_3$ (167,146) | 2.35 | 1.27 | 1.21 | 1.36 | 1.27 | 1.88 | 1.85 | 1.37 | 2.20 |
| MnO (225,166) | 2.94 | 1.64 | 1.59 | 1.69 | 1.67 | 2.98 | 2.67 | 2.69 | 3.90 |
| FeO (225,166) | 1.84 | 0.77 | 0.73 | 0.84 | 0.77 | 1.91 | 1.66 | 1.48 | 2.40 |
| CoO (225,166) | 3.13 | 1.24 | 1.18 | 1.35 | 1.24 | 2.84 | 2.53 | 2.17 | 2.50 |
| NiO (225,166) | 4.14 | 1.94 | 1.91 | 2.01 | 1.95 | 3.24 | 2.98 | 2.55 | 4.30 |
| $Cu_2O$ (224) | 0.81 | 0.64 | 0.64 | 0.63 | 0.65 | 0.92 | 0.75 | 0.95 | 2.17 |
| CuSCN (160) | 2.79 | 2.71 | 2.68 | 2.66 | 2.71 | 2.91 | 2.84 | 2.91 | 3.94 |
| CuCl (216) | 1.69 | 1.14 | 1.09 | 1.10 | 1.15 | 2.10 | 1.71 | 2.10 | 3.40 |
| CuBr (216) | 1.56 | 1.02 | 0.98 | 0.99 | 1.03 | 1.95 | 1.61 | 1.89 | 3.07 |
| CuI (216) | 2.20 | 1.68 | 1.65 | 1.67 | 1.68 | 2.48 | 2.23 | 2.35 | 3.12 |
| ZnO (wurtzite,186) | 2.65 | 1.43 | 1.40 | 1.41 | 1.46 | 2.46 | 2.18 | 2.44 | 3.44 |
| ZnS (216) | 3.65 | 2.86 | 2.82 | 2.84 | 2.87 | 4.06 | 3.58 | 3.60 | 3.84 |
| ZnSe (216) | 2.75 | 1.93 | 1.89 | 1.93 | 1.93 | 2.92 | 2.55 | 2.49 | 2.82 |
| ZnTe (216) | 2.42 | 1.68 | 1.66 | 1.69 | 1.69 | 2.40 | 2.15 | 2.02 | 2.39 |
| $MoS_2$ (194) | 1.08 | 1.04 | 1.03 | 1.10 | 1.04 | 1.25 | 1.15 | 1.14 | 1.29 |
| AgCl (225) | 2.95 | 2.01 | 1.95 | 2.08 | 2.01 | 3.83 | 3.23 | 3.31 | 3.25 |
| AgBr (225) | 2.50 | 1.62 | 1.57 | 1.70 | 1.62 | 3.17 | 2.70 | 2.68 | 2.71 |
| AgI (216) | 2.77 | 2.21 | 2.15 | 2.16 | 2.22 | 3.43 | 2.93 | 2.98 | 2.91 |
| CdS (216) | 2.67 | 2.02 | 1.97 | 1.99 | 2.02 | 3.34 | 2.77 | 2.76 | 2.50 |
| CdSe (216) | 1.99 | 1.36 | 1.31 | 1.35 | 1.36 | 2.44 | 2.00 | 1.93 | 1.85 |
| CdTe (216) | 1.79 | 1.26 | 1.23 | 1.26 | 1.26 | 2.07 | 1.75 | 1.62 | 1.61 |

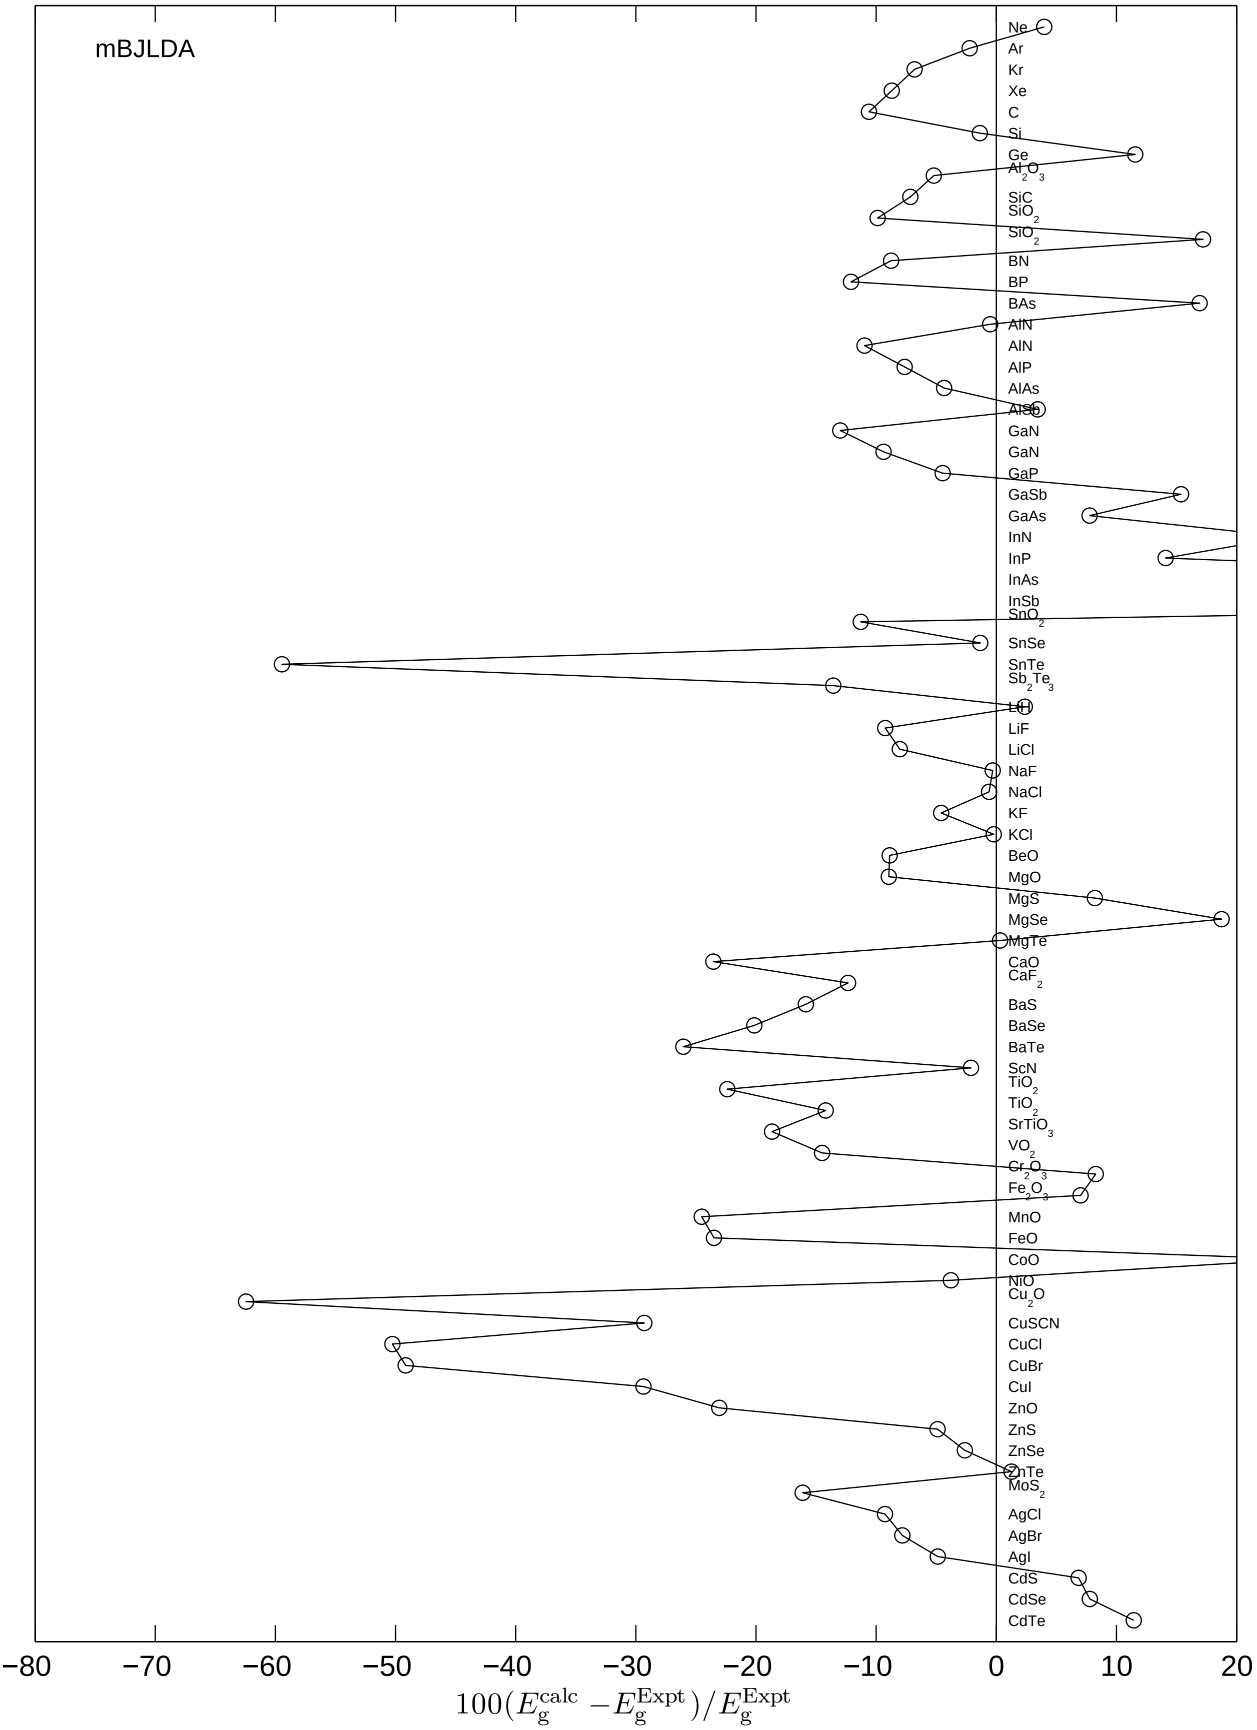


FIG. S25. Relative error (in %) in the calculated band gap $E_g$ with respect to the experimental values.

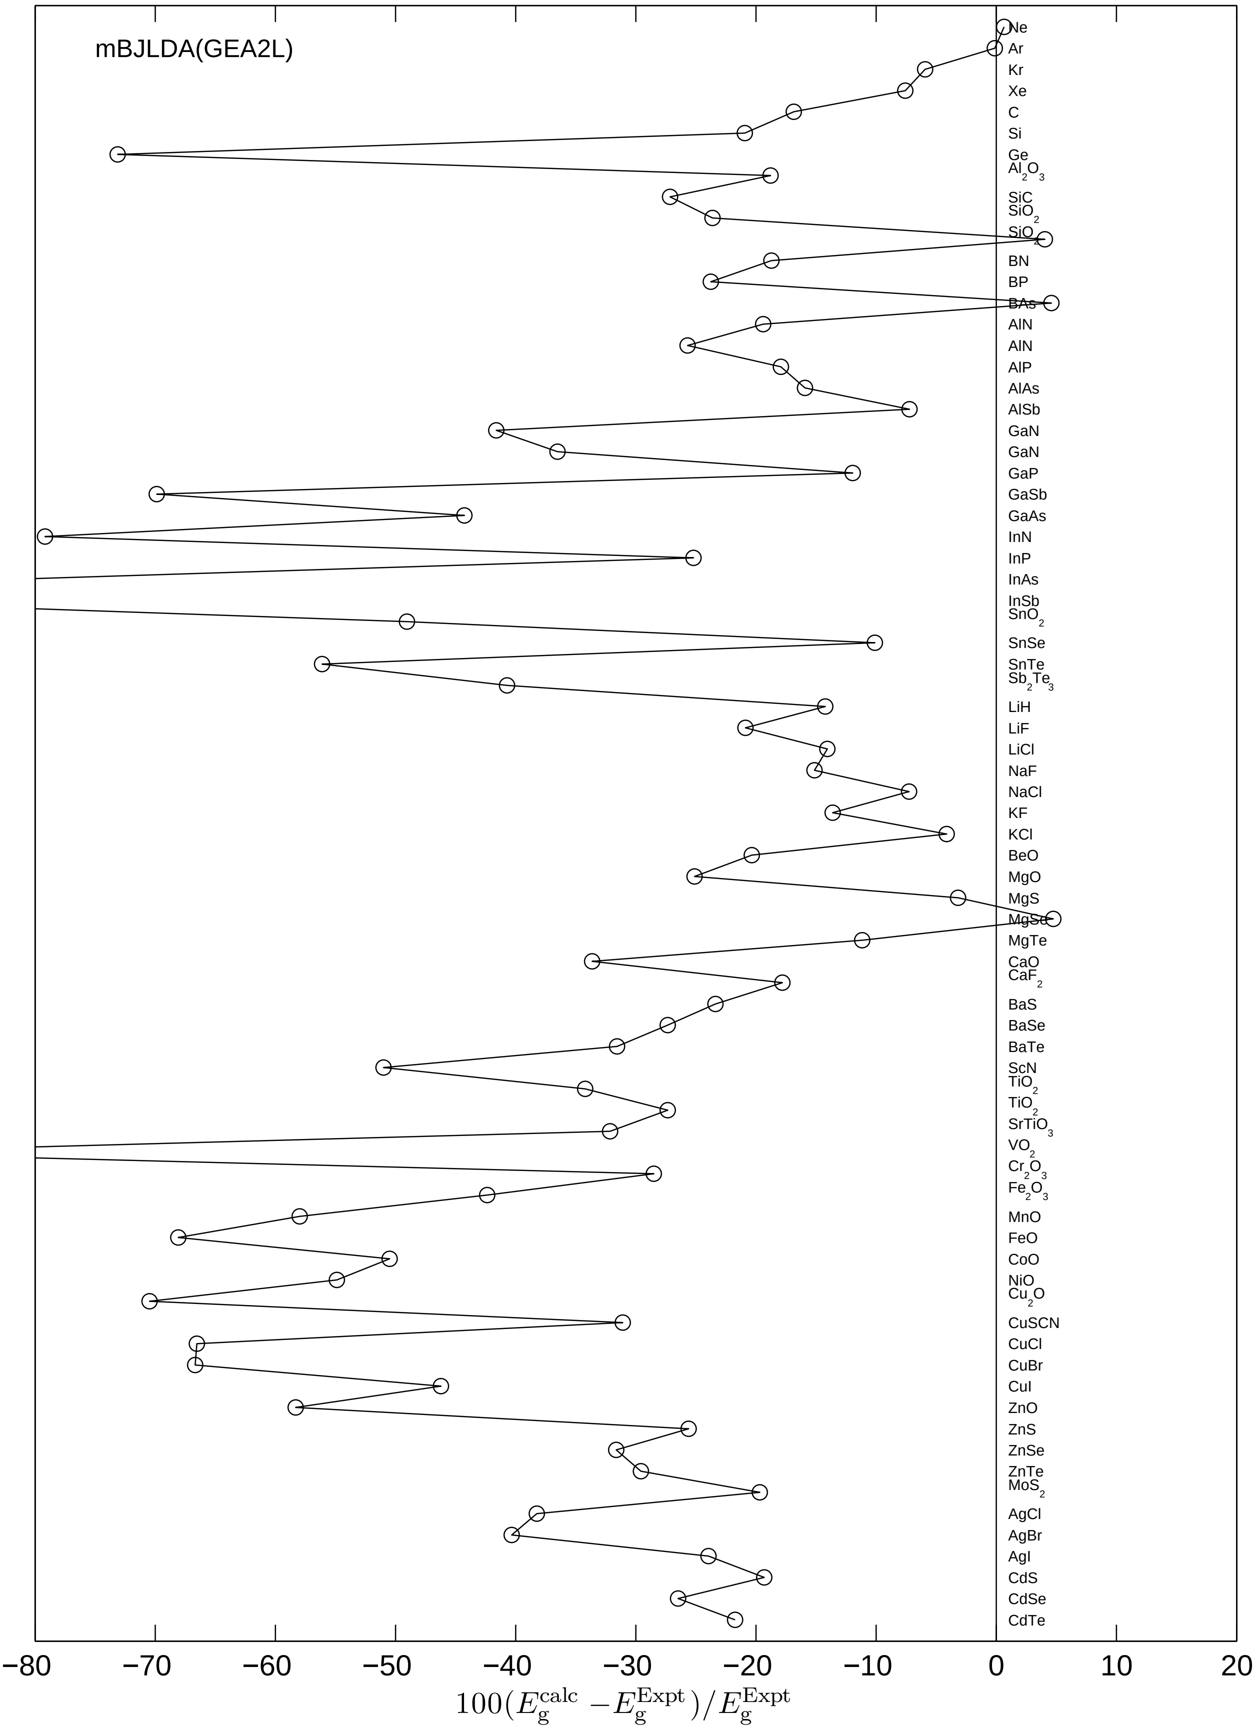


FIG. S26. Relative error (in %) in the calculated band gap $E_g$ with respect to the experimental values.

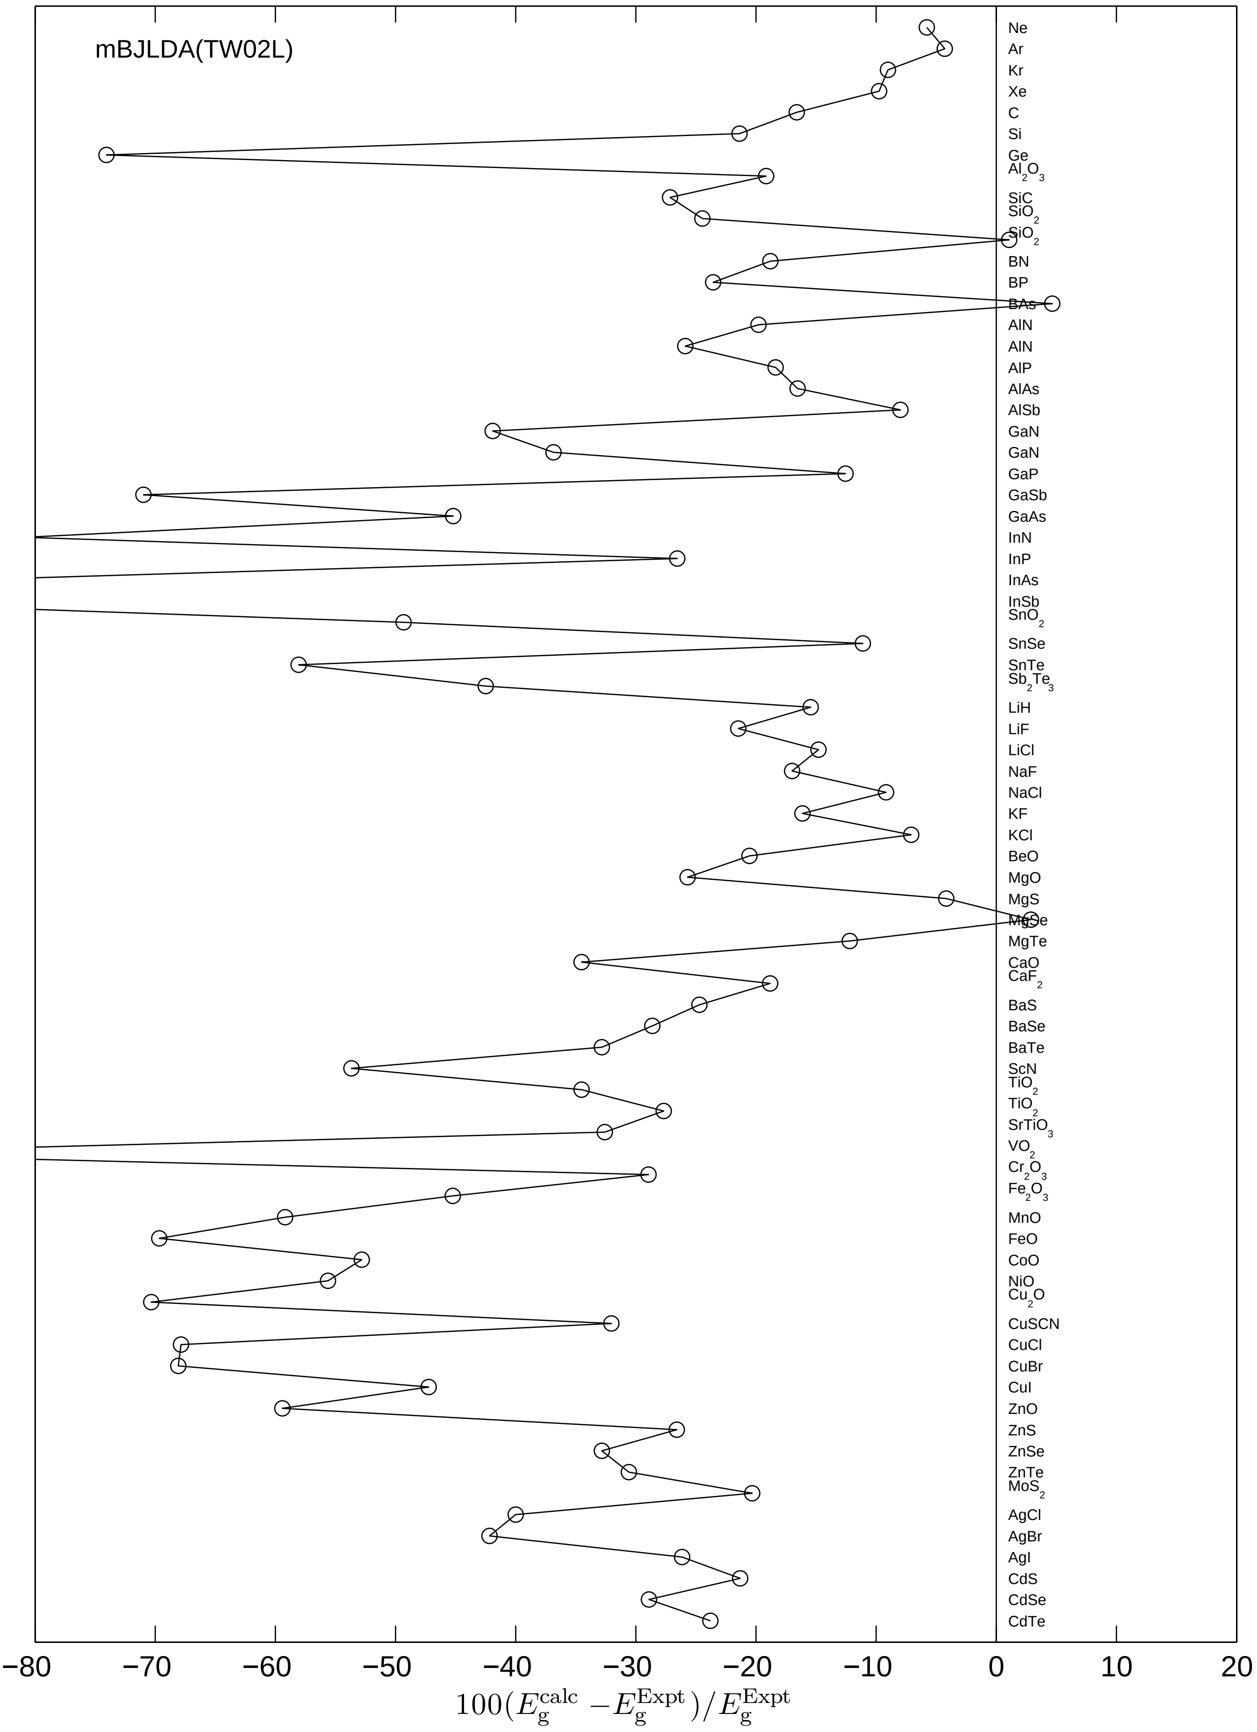


FIG. S27. Relative error (in %) in the calculated band gap $E_g$ with respect to the experimental values.

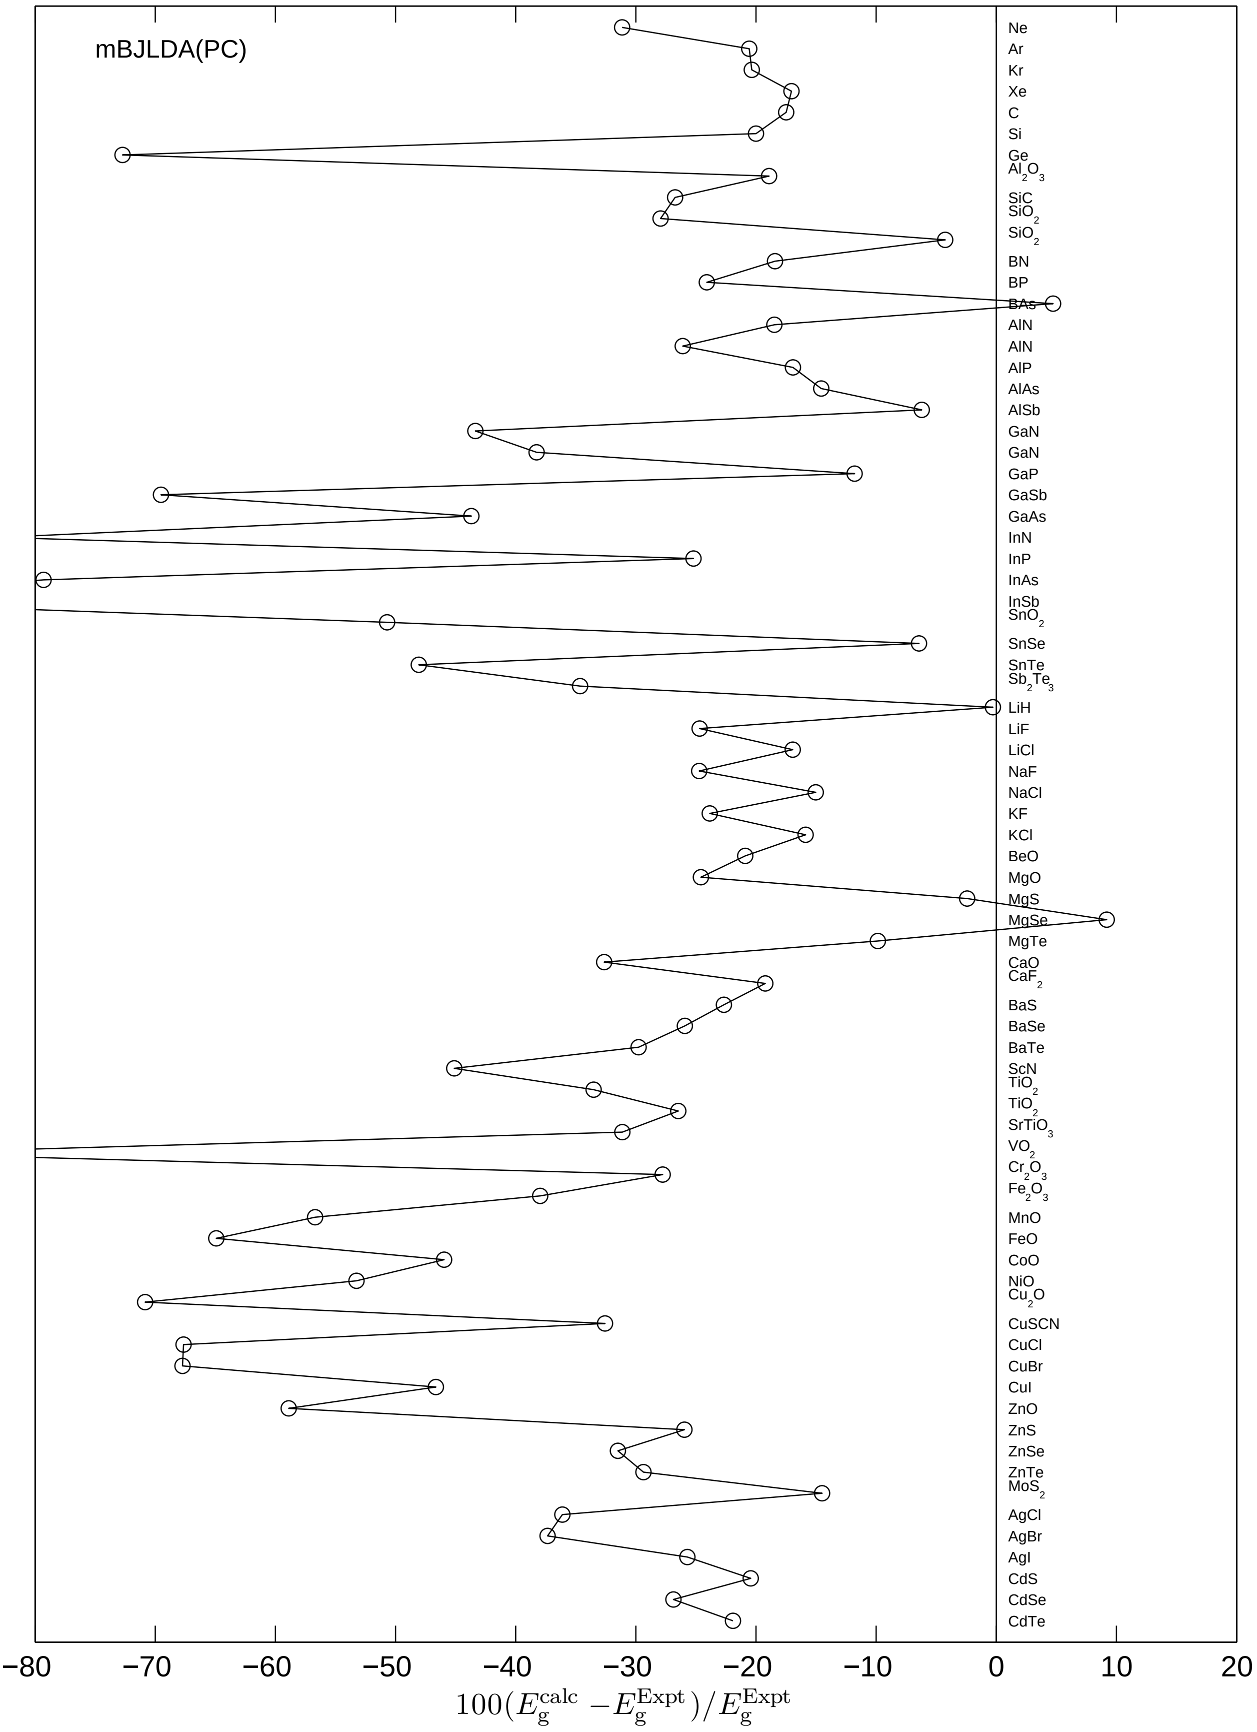


FIG. S28. Relative error (in %) in the calculated band gap $E_g$ with respect to the experimental values.

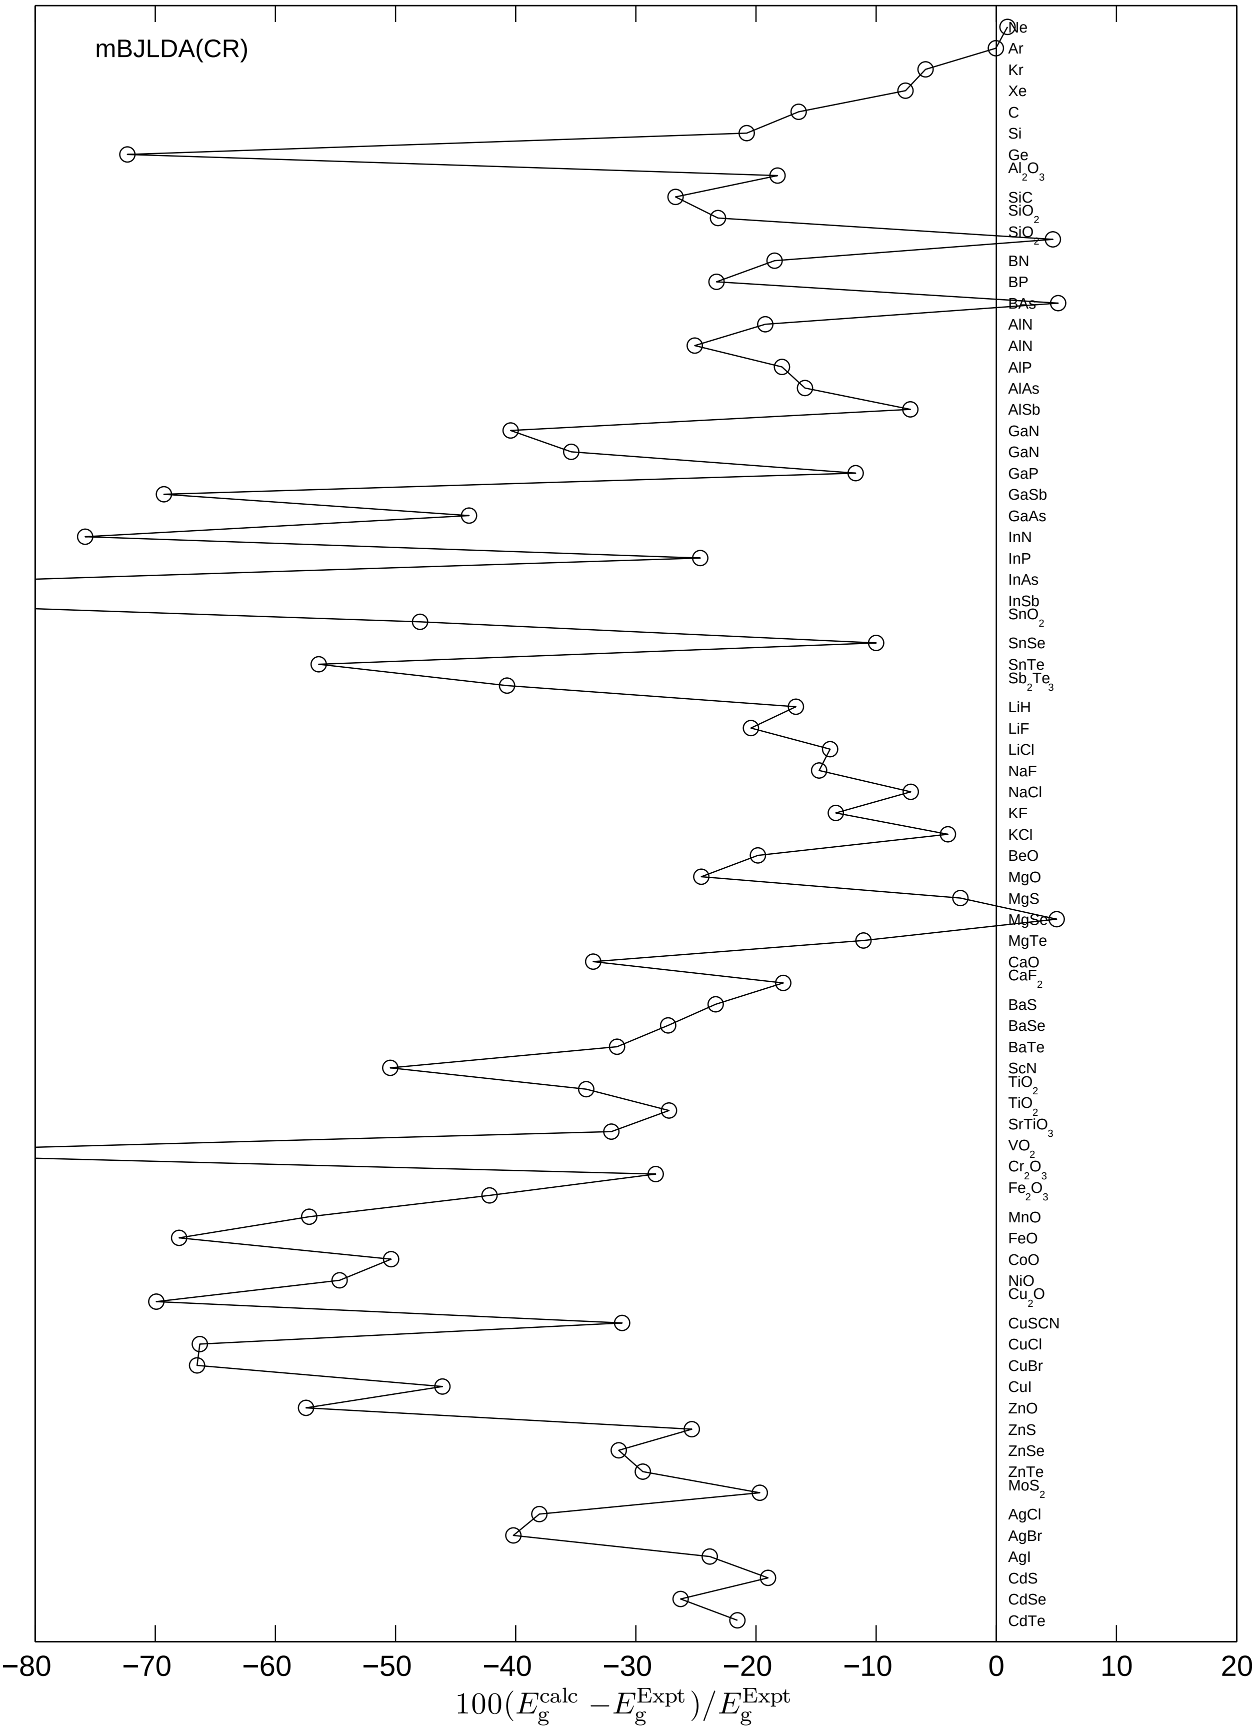


FIG. S29. Relative error (in %) in the calculated band gap $E_g$ with respect to the experimental values.

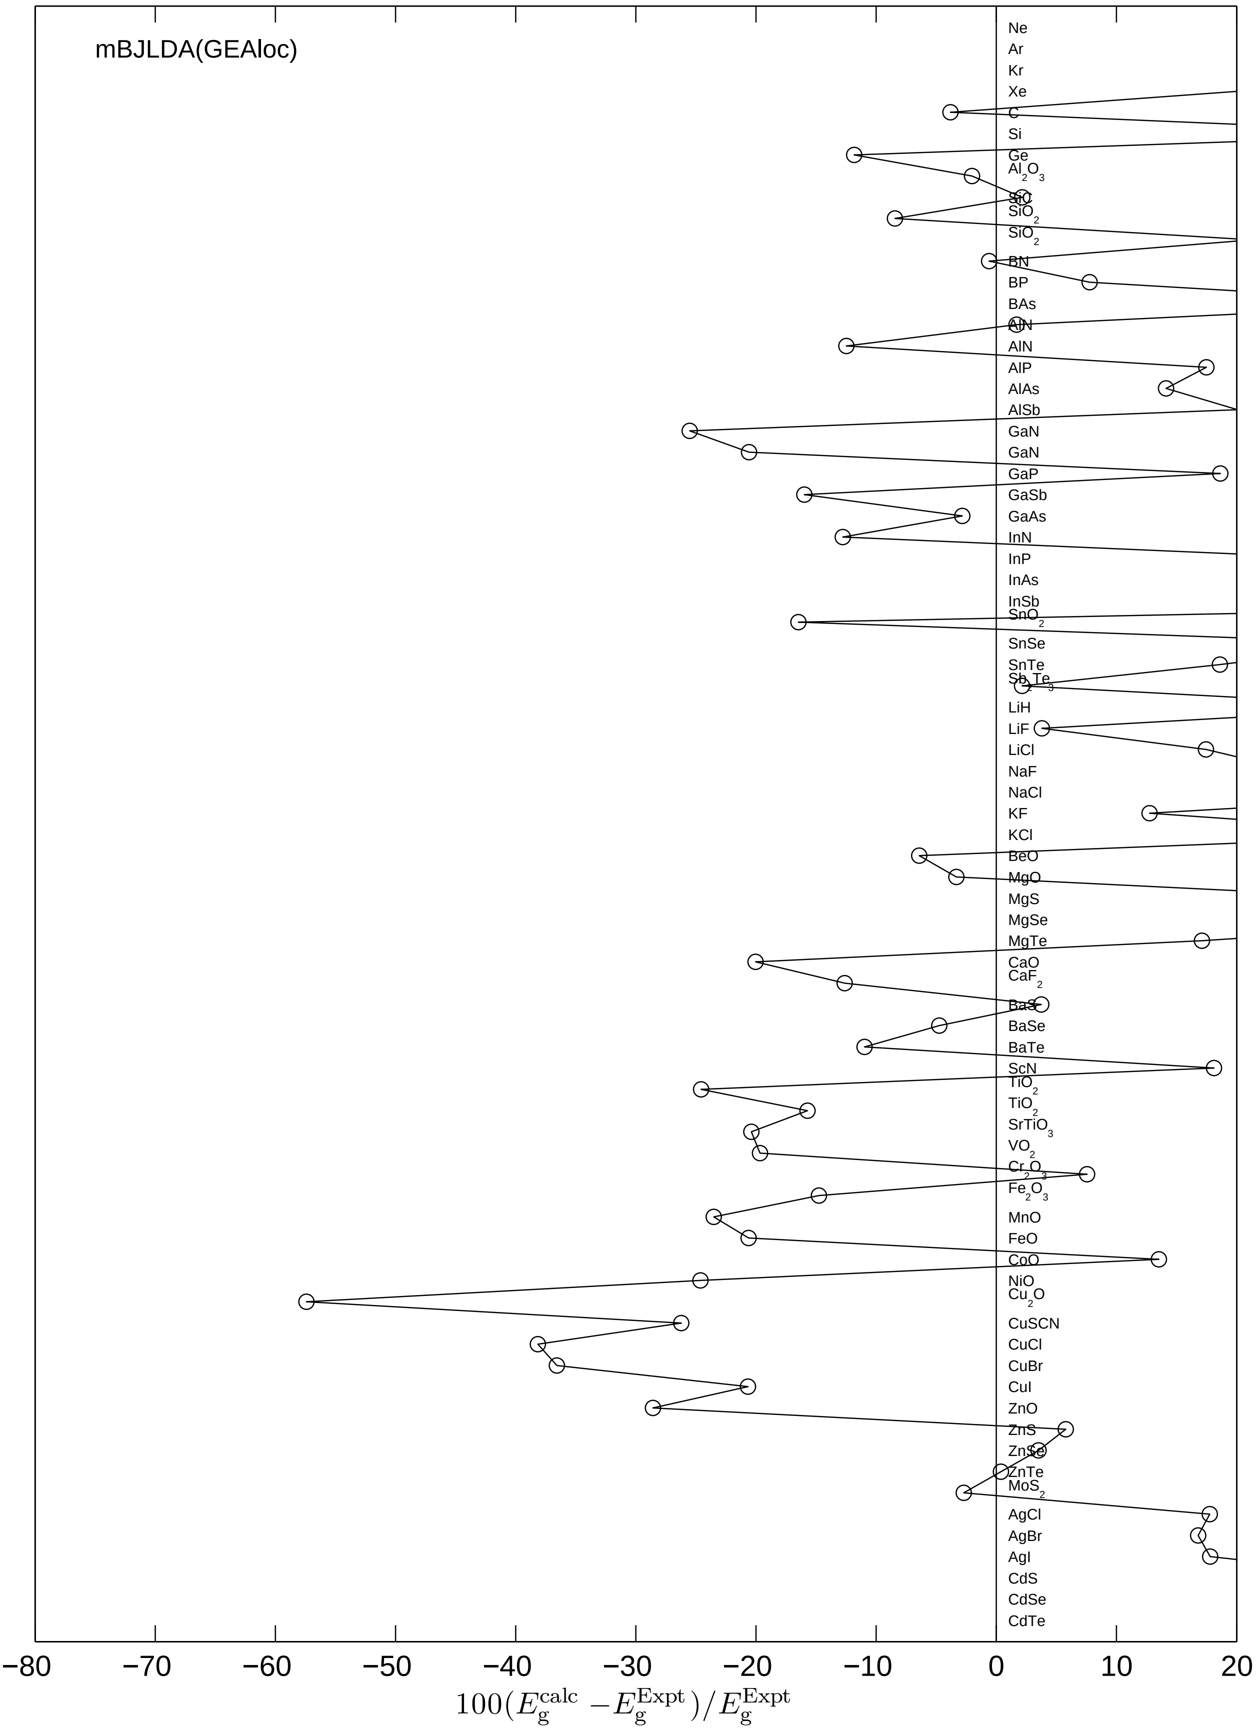


FIG. S30. Relative error (in %) in the calculated band gap $E_{\mathrm{g}}$ with respect to the experimental values.

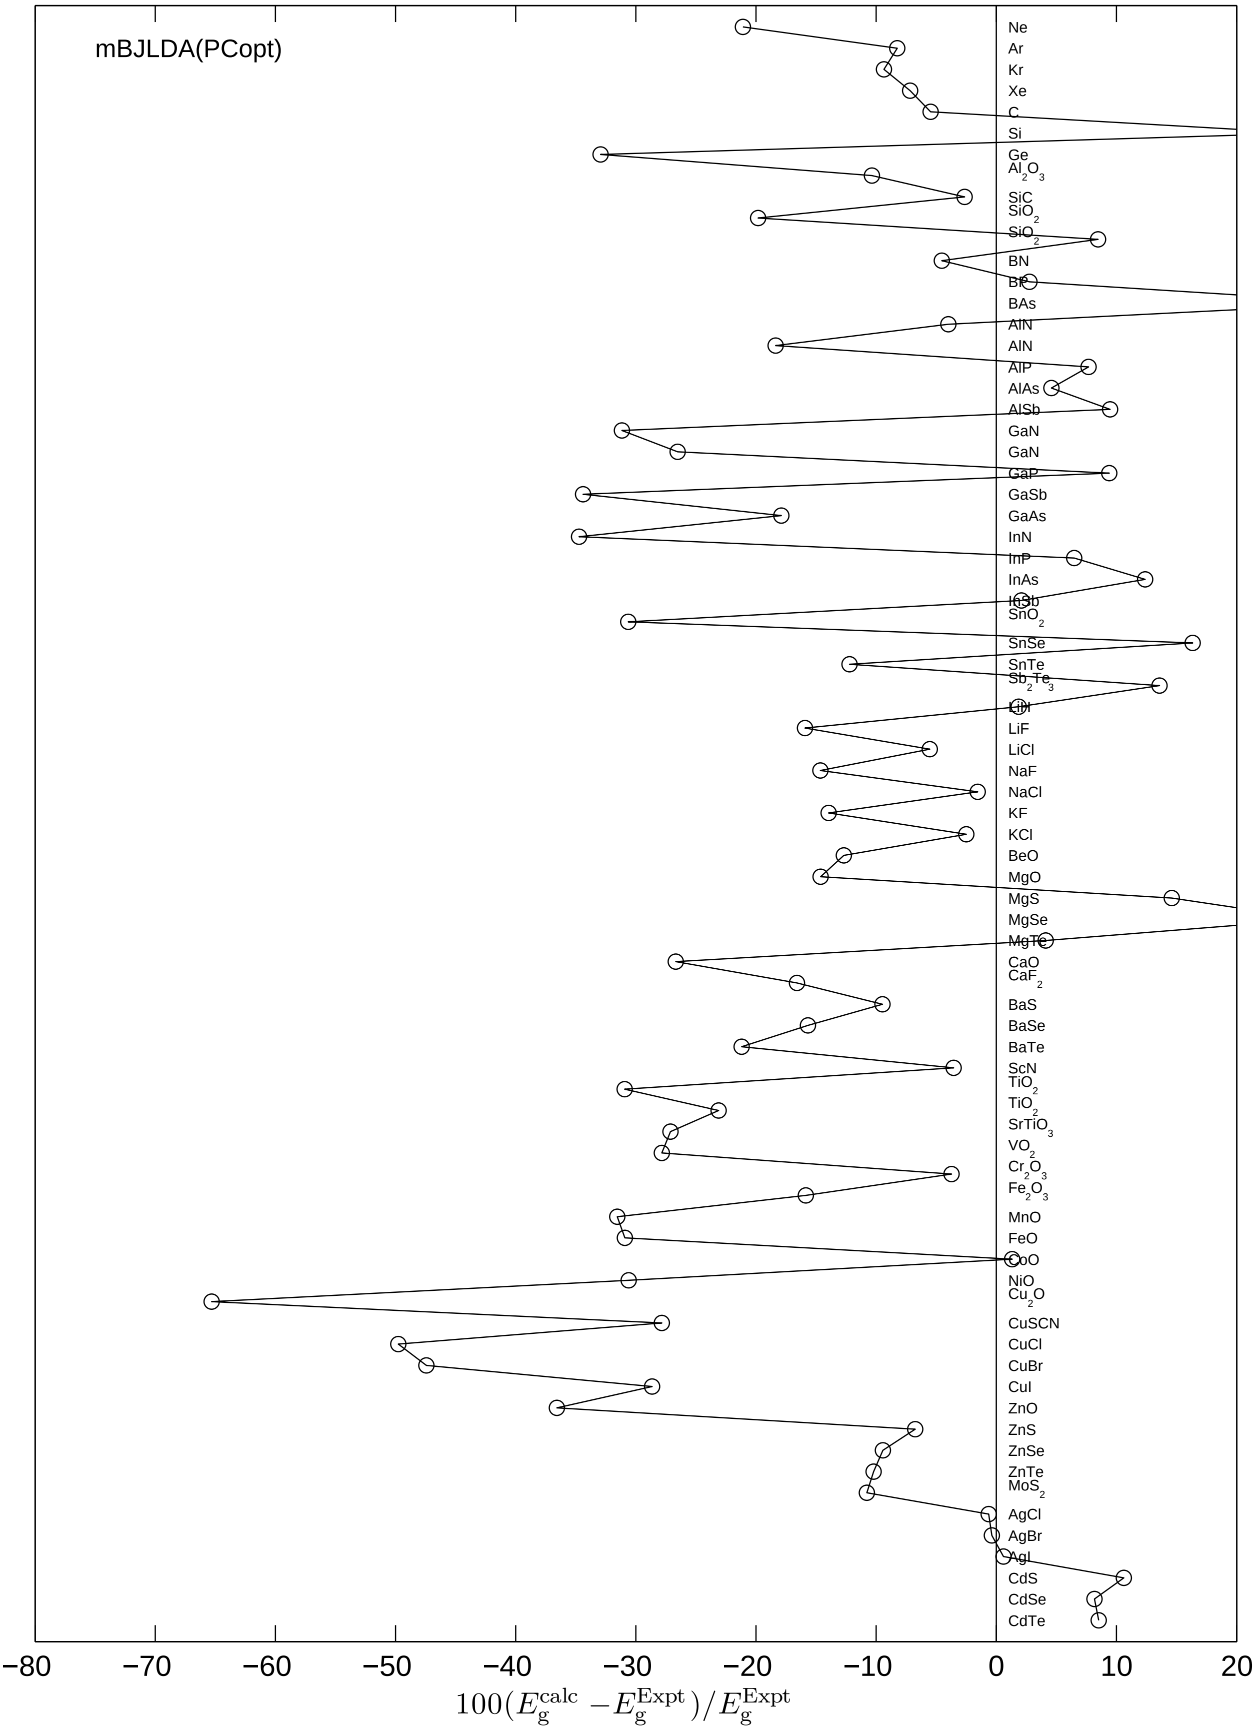


FIG. S31. Relative error (in %) in the calculated band gap $E_g$ with respect to the experimental values.

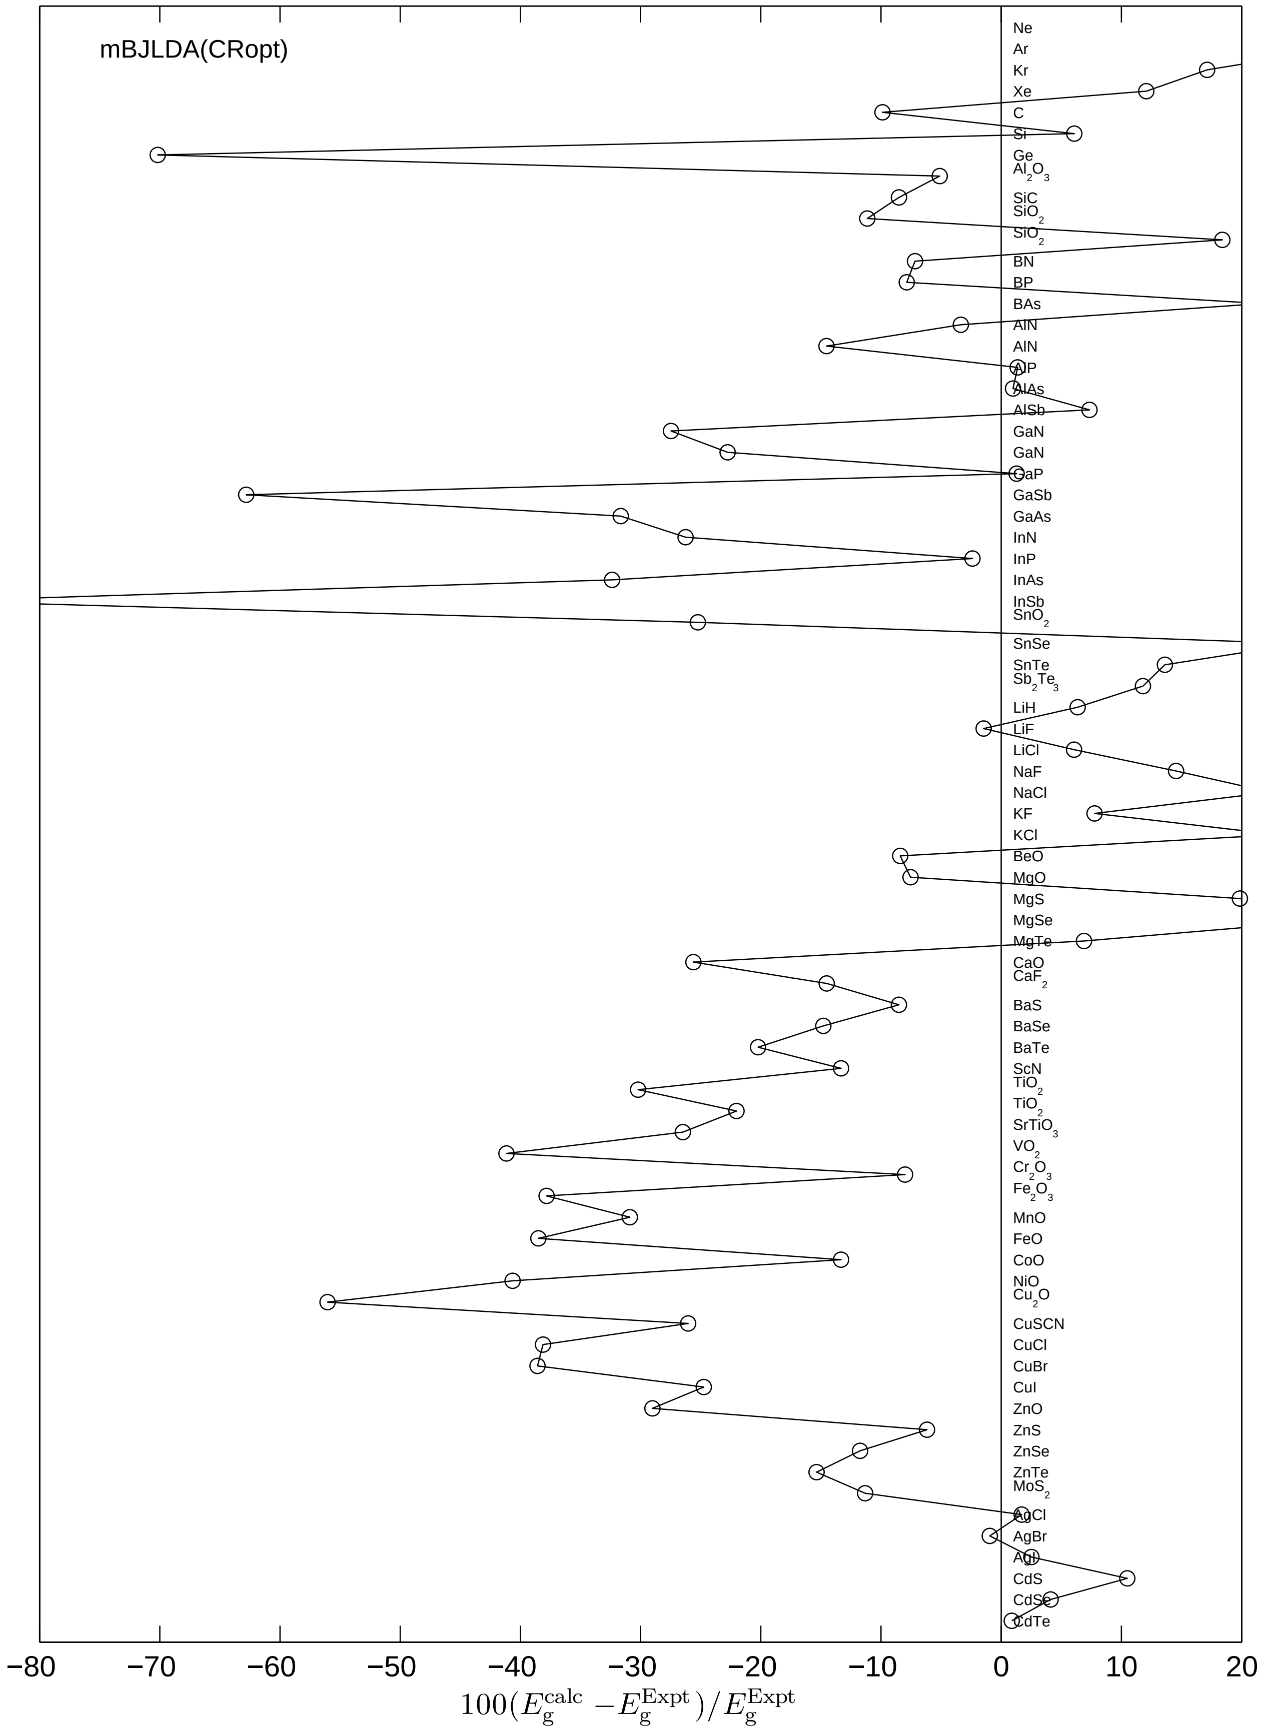


FIG. S32. Relative error (in %) in the calculated band gap $E_g$ with respect to the experimental values.

[1] L. Schimka, J. Harl, and G. Kresse, J. Chem. Phys. **134**, 024116 (2011).
[2] K. Lejaeghere, V. Van Speybroeck, G. Van Oost, and S. Cottenier, Crit. Rev. Solid State Mater. Sci. **39**, 1 (2014).
[3] ICSD, Inorganic Crystal Structure Database, http://icsd.fiz-karlsruhe.de.
[4] American Mineralogist Crystal Structure Database, http://rruff.geo.arizona.edu/AMS/amcsd.php.
[5] J. Heyd, J. E. Peralta, G. E. Scuseria, and R. L. Martin, J. Chem. Phys. **123**, 174101 (2005).
[6] J. M. Crowley, J. Tahir-Kheli, and W. A. Goddard, III, J. Phys. Chem. Lett. **7**, 1198 (2016).
[7] M. J. Lucero, T. M. Henderson, and G. E. Scuseria, J. Phys.: Condens. Matter **24**, 145504 (2012).
[8] S. Bernstorff and V. Saile, Opt. Commun. **58**, 181 (1986).
[9] R. Gillen and J. Robertson, J. Phys.: Condens. Matter **25**, 165502 (2013).
[10] D. Koller, P. Blaha, and F. Tran, J. Phys.: Condens. Matter **25**, 435503 (2013).
[11] J. H. Skone, M. Govoni, and G. Galli, Phys. Rev. B **89**, 195112 (2014).
[12] H. Shi, R. I. Eglitis, and G. Borstel, Phys. Rev. B **72**, 045109 (2005).
[13] J. Lee, A. Seko, K. Shitara, K. Nakayama, and I. Tanaka, Phys. Rev. B **93**, 115104 (2016).
[14] A. M. Ganose and D. O. Scanlon, J. Mater. Chem. C **4**, 1467 (2016).
[15] D. Groh, R. Pandey, M. B. Sahariah, E. Amzallag, I. Baraille, and M. Rérat, J. Phys. Chem. Solids **70**, 789 (2009).
